# Supplementary material for: Consequences of Weyl Consistency Conditions
Source: arXiv:1308.1096 ancillary file (2014-06-13)
Supplement: Supplementary file 1 [file WeylConsistencyConditionsIn6D.nb.pdf]

# Weyl consistency conditions in $d = 6$

Below we present to the interested reader the forty one consistency conditions that constrain the generating functional  $W$  in six dimensions. The  $(n,m)$  notation indicates the number of derivatives on each variational parameter:  $n$  on  $\sigma_1$  and  $m$  on  $\sigma_2$ . For example, in the (1,4) consistency conditions, we have selected terms proportional to  $\partial_\mu \sigma_1 \nabla^4 \sigma_2$  even though the actual condition is proportional to  $\partial_\mu \sigma_{[1} \nabla^4 \sigma_{2]}$ . This reduces clutter and elucidates the consistency conditions. Terms that match from the  $\sum_p \int d^6 x \sqrt{\gamma} \sigma \mathcal{T}_p$  contribution to the anomaly are prefaced with T[n]; similarly, terms that match from the  $\sum_q \int d^6 x \sqrt{\gamma} \sigma \mathcal{Z}_q$  contribution to the anomaly are prefaced with Z[n].

These form of these consistency conditions is not unique (for example, the Einstein tensor  $G^{\mu\nu}$  has been chosen in favor of the Ricci tensor  $R^{\mu\nu}$ ) and, furthermore, the relations below could be further decomposed in certain cases that capture specific arrangements of derivatives on the spacetime-dependent couplings  $\lambda^i(x)$ . We have chosen a basis convenient for the purposes of this work, specifically to elucidate a candidate for the  $\mathcal{A}$ -theorem. The relation that provides this candidate, equation (3.3) in the paper, can be found in consistency condition 32 below, which is the (0,1) consistency condition proportional to the Lovelock tensor  $H_1^{\mu\nu}$ . As another example, the relations in equation (3.4) in the paper can be found in consistency conditions 8, 36, and 38.

## (1,4) terms: one consistency condition

### ■ 1) $\partial_\mu \sigma_1 \nabla^4 \sigma_2 - \partial_\mu \sigma_2 \nabla^4 \sigma_1$

$$T[15]: -2 \mathcal{I}^4{}^m (\nabla_a \sigma_1) (\nabla^a \lambda_m) (\nabla_c \nabla^c \nabla_b \nabla^b \sigma_2)$$

$$T[48]: -3 \beta^m (\nabla_a \sigma_1) (\nabla^a \mathcal{J}_m) (\nabla_c \nabla^c \nabla_b \nabla^b \sigma_2) + \\ 3 \mathcal{J}^m (\nabla_a \sigma_1) (\nabla^a \beta_m) (\nabla_c \nabla^c \nabla_b \nabla^b \sigma_2) + 4 \mathcal{J}^m (\nabla_a \sigma_1) (\nabla^a \lambda_m) (\nabla_c \nabla^c \nabla_b \nabla^b \sigma_2)$$

$$Z[4]: 4 (\nabla_a \sigma_1) (\nabla^a b_{11}) (\nabla_c \nabla^c \nabla_b \nabla^b \sigma_2)$$

$$Z[11]: 2 \mathcal{G}^4{}^m (\nabla_a \sigma_1) (\nabla^a \lambda_m) (\nabla_c \nabla^c \nabla_b \nabla^b \sigma_2)$$

$$Z[16]: 5 \mathcal{H}^5{}^m (\nabla_a \sigma_1) (\nabla^a \lambda_m) (\nabla_c \nabla^c \nabla_b \nabla^b \sigma_2)$$

$$Z[17]: 2 \mathcal{H}^6{}^m (\nabla_a \sigma_1) (\nabla^a \lambda_m) (\nabla_c \nabla^c \nabla_b \nabla^b \sigma_2)$$

$$Z[27]: -\mathcal{A} \mathbf{p}^{mn} \beta_n (\nabla_a \sigma_1) (\nabla^a \lambda_m) (\nabla_c \nabla^c \nabla_b \nabla^b \sigma_2)$$

(1,3) terms: two consistency conditions

$$\blacksquare \textbf{2) } (\partial_\mu \sigma_1 \partial_\nu \nabla^2 \sigma_2 - \partial_\mu \sigma_2 \partial_\nu \nabla^2 \sigma_1) G^{\mu\nu}$$

$$Z[1]: -4 G[\nabla]^{ab} b_8 (\nabla_a \sigma_1) (\nabla_b \nabla_c \nabla^c \sigma_2)$$

$$Z[5]: -2 G[\nabla]^{ab} b_{12} (\nabla_a \sigma_1) (\nabla_b \nabla_c \nabla^c \sigma_2)$$

$$Z[6]: -2 G[\nabla]^{ab} b_{13} (\nabla_a \sigma_1) (\nabla_b \nabla_c \nabla^c \sigma_2)$$

$$Z[22]: -\frac{1}{2} G[\nabla]^{ab} c^m \beta_m (\nabla_a \sigma_1) (\nabla_b \nabla_c \nabla^c \sigma_2)$$

$$\blacksquare \textbf{3) } \partial_\mu \sigma_1 \partial_\nu \nabla^2 \sigma_2 - \partial_\mu \sigma_2 \partial_\nu \nabla^2 \sigma_1$$

$$T[27]: 2 \mathcal{HH}5^{mn} (\nabla_a \sigma_1) (\nabla^a \lambda_m) (\nabla_b \nabla_c \nabla^c \sigma_2) (\nabla^b \lambda_n)$$

$$T[28]: -\mathcal{HH}6^{mn} (\nabla_a \sigma_1) (\nabla^a \lambda_m) (\nabla_b \nabla_c \nabla^c \sigma_2) (\nabla^b \lambda_n)$$

$$T[48]: -4 (\nabla_a \sigma_1) (\nabla^a \mathcal{A}^m) (\nabla_b \nabla_c \nabla^c \sigma_2) (\nabla^b \beta_m) - 2 \beta^m (\nabla^a \sigma_1) (\nabla_b \nabla_c \nabla^c \sigma_2) (\nabla^b \nabla_a \mathcal{A}_m) - \\ 2 \mathcal{A}^m (\nabla^a \sigma_1) (\nabla_b \nabla_c \nabla^c \sigma_2) (\nabla^b \nabla_a \beta_m) - 8 \mathcal{A}^m (\nabla^a \sigma_1) (\nabla_b \nabla_c \nabla^c \sigma_2) (\nabla^b \nabla_a \lambda_m)$$

$$T[57]: \frac{1}{2} \mathcal{AAcheckpp}^{np}_m \beta^m (\nabla_a \sigma_1) (\nabla^a \lambda_n) (\nabla_b \nabla_c \nabla^c \sigma_2) (\nabla^b \lambda_p)$$

$$Z[4]: 4 (\nabla^a \sigma_1) (\nabla_b \nabla_c \nabla^c \sigma_2) (\nabla^b \nabla_a b_{11})$$

$$Z[16]: 4 (\nabla_a \sigma_1) (\nabla^a \mathcal{H}5^m) (\nabla_b \nabla_c \nabla^c \sigma_2) (\nabla^b \lambda_m) + 4 \mathcal{H}5^m (\nabla^a \sigma_1) (\nabla_b \nabla_c \nabla^c \sigma_2) (\nabla^b \nabla_a \lambda_m)$$

$$Z[17]: 2 (\nabla_a \sigma_1) (\nabla^a \mathcal{H}6^m) (\nabla_b \nabla_c \nabla^c \sigma_2) (\nabla^b \lambda_m) + 2 \mathcal{H}6^m (\nabla^a \sigma_1) (\nabla_b \nabla_c \nabla^c \sigma_2) (\nabla^b \nabla_a \lambda_m)$$

$$Z[18]: -4 \mathcal{F}^m (\nabla^a \sigma_1) (\nabla_b \nabla_c \nabla^c \sigma_2) (\nabla^b \nabla_a \lambda_m)$$

$$Z[20]: 2 \delta\delta^{mn} (\nabla_a \sigma_1) (\nabla^a \lambda_m) (\nabla_b \nabla_c \nabla^c \sigma_2) (\nabla^b \lambda_n)$$

$$Z[26]: -\mathcal{AA}^{mn} \beta_m (\nabla^a \sigma_1) (\nabla_b \nabla_c \nabla^c \sigma_2) (\nabla^b \nabla_a \lambda_n)$$

$$Z[27]: -2 \mathcal{AP}^{mn} (\nabla_a \sigma_1) (\nabla^a \beta_n) (\nabla_b \nabla_c \nabla^c \sigma_2) (\nabla^b \lambda_m)$$

## (1,2) terms: eight consistency conditions

■ 4)  $(\partial_\mu \sigma_1 \nabla^2 \sigma_2 - \partial_\mu \sigma_2 \nabla^2 \sigma_1) R$ 

$$T[10]: -R[\nabla] (\nabla_a \sigma_1) (\nabla^a b_6) (\nabla_b \nabla^b \sigma_2)$$

$$T[14]: -\frac{2}{5} R[\nabla] \mathcal{I}3^m (\nabla_a \sigma_1) (\nabla^a \lambda_m) (\nabla_b \nabla^b \sigma_2)$$

$$T[15]: -\frac{2}{5} R[\nabla] \mathcal{I}4^m (\nabla_a \sigma_1) (\nabla^a \lambda_m) (\nabla_b \nabla^b \sigma_2)$$

$$T[16]: -2 R[\nabla] \mathcal{I}5^m (\nabla_a \sigma_1) (\nabla^a \lambda_m) (\nabla_b \nabla^b \sigma_2)$$

$$T[17]: -5 R[\nabla] \mathcal{I}6^m (\nabla_a \sigma_1) (\nabla^a \lambda_m) (\nabla_b \nabla^b \sigma_2)$$

$$T[18]: -R[\nabla] \mathcal{I}7^m (\nabla_a \sigma_1) (\nabla^a \lambda_m) (\nabla_b \nabla^b \sigma_2)$$

$$T[42]: -\frac{2}{5} R[\nabla] \beta^m (\nabla_a \sigma_1) (\nabla^a \mathcal{B}_m) (\nabla_b \nabla^b \sigma_2) + \\ \frac{2}{5} R[\nabla] \mathcal{B}^m (\nabla_a \sigma_1) (\nabla^a \beta_m) (\nabla_b \nabla^b \sigma_2) + \frac{4}{5} R[\nabla] \mathcal{B}^m (\nabla_a \sigma_1) (\nabla^a \lambda_m) (\nabla_b \nabla^b \sigma_2)$$

$$Z[3]: \frac{2}{5} R[\nabla] (\nabla_a \sigma_1) (\nabla^a b_{10}) (\nabla_b \nabla^b \sigma_2)$$

$$Z[4]: \frac{2}{5} R[\nabla] (\nabla_a \sigma_1) (\nabla^a b_{11}) (\nabla_b \nabla^b \sigma_2)$$

$$Z[5]: 2 R[\nabla] (\nabla_a \sigma_1) (\nabla^a b_{12}) (\nabla_b \nabla^b \sigma_2)$$

$$Z[6]: 5 R[\nabla] (\nabla_a \sigma_1) (\nabla^a b_{13}) (\nabla_b \nabla^b \sigma_2)$$

$$Z[7]: R[\nabla] (\nabla_a \sigma_1) (\nabla^a b_{14}) (\nabla_b \nabla^b \sigma_2)$$

$$Z[10]: \frac{4}{5} R[\nabla] \mathcal{G}3^m (\nabla_a \sigma_1) (\nabla^a \lambda_m) (\nabla_b \nabla^b \sigma_2)$$

$$Z[11]: \frac{2}{5} R[\nabla] \mathcal{G}4^m (\nabla_a \sigma_1) (\nabla^a \lambda_m) (\nabla_b \nabla^b \sigma_2)$$

$$Z[13]: 2 R[\nabla] \mathcal{H}2^m (\nabla_a \sigma_1) (\nabla^a \lambda_m) (\nabla_b \nabla^b \sigma_2)$$

$$Z[14]: 5 R[\nabla] \mathcal{H}3^m (\nabla_a \sigma_1) (\nabla^a \lambda_m) (\nabla_b \nabla^b \sigma_2)$$

$$Z[15]: R[\nabla] \mathcal{H}4^m (\nabla_a \sigma_1) (\nabla^a \lambda_m) (\nabla_b \nabla^b \sigma_2)$$

$$Z[16]: 5 R[\nabla] \mathcal{H}5^m (\nabla_a \sigma_1) (\nabla^a \lambda_m) (\nabla_b \nabla^b \sigma_2)$$

$$Z[17]: \frac{2}{5} R[\nabla] \mathcal{H}6^m (\nabla_a \sigma_1) (\nabla^a \lambda_m) (\nabla_b \nabla^b \sigma_2)$$

$$Z[18]: -2 R[\nabla] \mathcal{F}^m (\nabla_a \sigma_1) (\nabla^a \lambda_m) (\nabla_b \nabla^b \sigma_2)$$

$$Z[25]: -\frac{1}{5} R[\nabla] \mathcal{B}\mathcal{B}_m^n \beta^m (\nabla_a \sigma_1) (\nabla^a \lambda_n) (\nabla_b \nabla^b \sigma_2)$$

■ 5)  $(\partial_\mu \sigma_1 \nabla^2 \sigma_2 - \partial_\mu \sigma_2 \nabla^2 \sigma_1) \partial^\mu R$

$$T[10]: -b6 (\nabla_a \sigma_1) (\nabla^a R[\nabla]) (\nabla_b \nabla^b \sigma_2)$$

$$T[11]: 4 b7 (\nabla_a \sigma_1) (\nabla^a R[\nabla]) (\nabla_b \nabla^b \sigma_2)$$

$$T[42]: -\frac{2}{5} \mathcal{B}^m \beta_m (\nabla_a \sigma_1) (\nabla^a R[\nabla]) (\nabla_b \nabla^b \sigma_2)$$

$$Z[18]: -\frac{1}{2} \mathcal{F}^m \beta_m (\nabla_a \sigma_1) (\nabla^a R[\nabla]) (\nabla_b \nabla^b \sigma_2)$$

$$Z[19]: -\frac{1}{5} \mathcal{E}^m \beta_m (\nabla_a \sigma_1) (\nabla^a R[\nabla]) (\nabla_b \nabla^b \sigma_2)$$

■ 6)  $(\partial_\nu \sigma_1 \nabla^2 \sigma_2 - \partial_\nu \sigma_2 \nabla^2 \sigma_1) G^{\mu\nu}$

$$T[16]: -2 G[\nabla]^{ab} I5^m (\nabla_a \lambda_m) (\nabla_b \sigma_1) (\nabla_c \nabla^c \sigma_2)$$

$$T[17]: -6 G[\nabla]^{ab} I6^m (\nabla_a \lambda_m) (\nabla_b \sigma_1) (\nabla_c \nabla^c \sigma_2)$$

$$Z[1]: -4 G[\nabla]^{ab} (\nabla_a b8) (\nabla_b \sigma_1) (\nabla_c \nabla^c \sigma_2)$$

$$Z[6]: 4 G[\nabla]^{ab} (\nabla_a b13) (\nabla_b \sigma_1) (\nabla_c \nabla^c \sigma_2)$$

$$Z[13]: 2 G[\nabla]^{ab} \mathcal{H}2^m (\nabla_a \lambda_m) (\nabla_b \sigma_1) (\nabla_c \nabla^c \sigma_2)$$

$$Z[14]: 6 G[\nabla]^{ab} \mathcal{H}3^m (\nabla_a \lambda_m) (\nabla_b \sigma_1) (\nabla_c \nabla^c \sigma_2)$$

$$Z[16]: 6 G[\nabla]^{ab} \mathcal{H}5^m (\nabla_a \lambda_m) (\nabla_b \sigma_1) (\nabla_c \nabla^c \sigma_2)$$

$$Z[18]: -4 G[\nabla]^{ab} \mathcal{F}^m (\nabla_a \lambda_m) (\nabla_b \sigma_1) (\nabla_c \nabla^c \sigma_2)$$

$$Z[22]: -\frac{1}{2} G[\nabla]^{ab} C^m (\nabla_a \beta_m) (\nabla_b \sigma_1) (\nabla_c \nabla^c \sigma_2)$$

$$Z[24]: -\frac{1}{2} G[\nabla]^{ab} CC^{mn} \beta_n (\nabla_a \lambda_m) (\nabla_b \sigma_1) (\nabla_c \nabla^c \sigma_2)$$

■ 7)  $(\partial_\mu \sigma_1 \nabla_\nu \partial_\rho \sigma_2 - \partial_\mu \sigma_2 \nabla_\nu \partial_\rho \sigma_1) G^{\nu\rho}$

$$T[12]: 4 G[\nabla]^{ab} I1^m (\nabla_b \nabla_a \sigma_2) (\nabla_c \sigma_1) (\nabla^c \lambda_m)$$

$$T[17]: -4 G[\nabla]^{ab} I6^m (\nabla_b \nabla_a \sigma_2) (\nabla_c \sigma_1) (\nabla^c \lambda_m)$$

$$Z[1]: -4 G[\nabla]^{ab} (\nabla_b \nabla_a \sigma_2) (\nabla_c \sigma_1) (\nabla^c b8)$$

$$Z[6]: 4 G[\nabla]^{ab} (\nabla_b \nabla_a \sigma_2) (\nabla_c \sigma_1) (\nabla^c b13)$$

$$Z[8]: -4 G[\nabla]^{ab} \mathcal{G}1^m (\nabla_b \nabla_a \sigma_2) (\nabla_c \sigma_1) (\nabla^c \lambda_m)$$

$$Z[14]: 4 G[\nabla]^{ab} \mathcal{H}3^m (\nabla_b \nabla_a \sigma_2) (\nabla_c \sigma_1) (\nabla^c \lambda_m)$$

$$Z[16]: 4 G[\nabla]^{ab} \mathcal{H}5^m (\nabla_b \nabla_a \sigma_2) (\nabla_c \sigma_1) (\nabla^c \lambda_m)$$

$$Z[22]: -G[\nabla]^{ab} C^m (\nabla_b \nabla_a \sigma_2) (\nabla_c \sigma_1) (\nabla^c \beta_m) - 2 G[\nabla]^{ab} C^m (\nabla_b \nabla_a \sigma_2) (\nabla_c \sigma_1) (\nabla^c \lambda_m)$$

$$Z[23]: -\frac{1}{2} G[\nabla]^{ab} CC^{mn} \beta_n (\nabla_b \nabla_a \sigma_2) (\nabla_c \sigma_1) (\nabla^c \lambda_m)$$

■ 8)  $(\partial_\mu \sigma_1 \nabla_\nu \partial_\rho \sigma_2 - \partial_\mu \sigma_2 \nabla_\nu \partial_\rho \sigma_1) \nabla^\mu G^{\nu\rho}$

$$T[11]: 8 \, b7 \, (\nabla_a G[\nabla]^{bc}) \, (\nabla^a \sigma_1) \, (\nabla_c \nabla_b \sigma_2)$$

$$Z[18]: -\mathcal{F}^m \, \beta_m \, (\nabla_a G[\nabla]^{bc}) \, (\nabla^a \sigma_1) \, (\nabla_c \nabla_b \sigma_2)$$

■ 9)  $(\partial_\nu \sigma_1 \nabla_\rho \partial_\sigma \sigma_2 - \partial_\nu \sigma_2 \nabla_\rho \partial_\sigma \sigma_1) R^{\mu\sigma\nu\rho}$

$$T[18]: -4 \, R[\nabla]^{abcd} \, I7^m \, (\nabla_a \lambda_m) \, (\nabla_c \sigma_1) \, (\nabla_d \nabla_b \sigma_2)$$

$$Z[7]: 4 \, R[\nabla]^{abcd} \, (\nabla_a b14) \, (\nabla_c \sigma_1) \, (\nabla_d \nabla_b \sigma_2)$$

$$Z[12]: 16 \, R[\nabla]^{abcd} \, \mathcal{H}1^m \, (\nabla_a \lambda_m) \, (\nabla_c \sigma_1) \, (\nabla_d \nabla_b \sigma_2)$$

$$Z[15]: 4 \, R[\nabla]^{abcd} \, \mathcal{H}4^m \, (\nabla_a \lambda_m) \, (\nabla_c \sigma_1) \, (\nabla_d \nabla_b \sigma_2)$$

$$Z[16]: -8 \, R[\nabla]^{abcd} \, \mathcal{H}5^m \, (\nabla_a \lambda_m) \, (\nabla_c \sigma_1) \, (\nabla_d \nabla_b \sigma_2)$$

$$Z[21]: -R[\nabla]^{abcd} \, \mathcal{D}\mathcal{D}^{mn} \, \beta_n \, (\nabla_a \lambda_m) \, (\nabla_c \sigma_1) \, (\nabla_d \nabla_b \sigma_2)$$

■ 10)  $\partial_\mu \sigma_1 \nabla^2 \sigma_2 - \partial_\mu \sigma_2 \nabla^2 \sigma_1$

$$T[15]: -4 \, I4^m \, (\nabla_a \nabla_c \nabla^c \lambda_m) \, (\nabla^a \sigma_1) \, (\nabla_b \nabla^b \sigma_2) - 4 \, (\nabla_a \sigma_1) \, (\nabla^a I4^m) \, (\nabla_b \nabla^b \lambda_m) \, (\nabla_c \nabla^c \sigma_2) - \\ 4 \, (\nabla^a \lambda^m) \, (\nabla_b \nabla_a I4_m) \, (\nabla^b \sigma_1) \, (\nabla_c \nabla^c \sigma_2) - 4 \, (\nabla^a I4^m) \, (\nabla_b \nabla_a \lambda_m) \, (\nabla^b \sigma_1) \, (\nabla_c \nabla^c \sigma_2)$$

$$T[22]: 2 \, (\nabla_a \lambda^n) \, (\nabla^a \lambda^m) \, (\nabla_b \mathcal{G}\mathcal{G}4_{mn}) \, (\nabla^b \sigma_1) \, (\nabla_c \nabla^c \sigma_2) + 4 \, \mathcal{G}\mathcal{G}4^{mn} \, (\nabla^a \lambda_m) \, (\nabla_b \nabla_a \lambda_n) \, (\nabla^b \sigma_1) \, (\nabla_c \nabla^c \sigma_2)$$

$$T[27]: 2 \, \mathcal{H}\mathcal{H}5^{mn} \, (\nabla_a \sigma_1) \, (\nabla^a \lambda_m) \, (\nabla_b \nabla^b \lambda_n) \, (\nabla_c \nabla^c \sigma_2) + \\ 2 \, (\nabla_a \sigma_1) \, (\nabla^a \lambda^m) \, (\nabla_b \mathcal{H}\mathcal{H}5_{mn}) \, (\nabla^b \lambda^n) \, (\nabla_c \nabla^c \sigma_2) + 2 \, \mathcal{H}\mathcal{H}5^{mn} \, (\nabla_a \nabla_b \lambda_n) \, (\nabla^a \lambda_m) \, (\nabla^b \sigma_1) \, (\nabla_c \nabla^c \sigma_2) + \\ (\nabla_a \lambda^n) \, (\nabla^a \lambda^m) \, (\nabla_b \mathcal{H}\mathcal{H}5_{mn}) \, (\nabla^b \sigma_1) \, (\nabla_c \nabla^c \sigma_2) + 2 \, \mathcal{H}\mathcal{H}5^{mn} \, (\nabla^a \lambda_m) \, (\nabla_b \nabla_a \lambda_n) \, (\nabla^b \sigma_1) \, (\nabla_c \nabla^c \sigma_2)$$

$$T[28]: \mathcal{H}\mathcal{H}6^{mn} \, (\nabla_a \sigma_1) \, (\nabla^a \lambda_m) \, (\nabla_b \nabla^b \lambda_n) \, (\nabla_c \nabla^c \sigma_2) + \\ (\nabla_a \sigma_1) \, (\nabla^a \lambda^m) \, (\nabla_b \mathcal{H}\mathcal{H}6_{mn}) \, (\nabla^b \lambda^n) \, (\nabla_c \nabla^c \sigma_2) + \mathcal{H}\mathcal{H}6^{mn} \, (\nabla_a \nabla_b \lambda_n) \, (\nabla^a \lambda_m) \, (\nabla^b \sigma_1) \, (\nabla_c \nabla^c \sigma_2)$$

$$T[29]: 2 \, \mathcal{F}\mathcal{F}^{mn} \, (\nabla_a \sigma_1) \, (\nabla^a \lambda_m) \, (\nabla_b \nabla^b \lambda_n) \, (\nabla_c \nabla^c \sigma_2)$$

$$T[30]: 2 \, \mathcal{F}\mathcal{F}p^{mn} \, (\nabla^a \lambda_m) \, (\nabla_b \nabla_a \lambda_n) \, (\nabla^b \sigma_1) \, (\nabla_c \nabla^c \sigma_2)$$

$$T[31]: \mathcal{F}\mathcal{F}\mathcal{F}^{mnp} \, (\nabla_a \sigma_1) \, (\nabla^a \lambda_m) \, (\nabla_b \lambda_p) \, (\nabla^b \lambda_n) \, (\nabla_c \nabla^c \sigma_2)$$

$$T[32]: -2 \, \mathcal{E}\mathcal{E}\text{hat}^{mn} \, (\nabla_a \sigma_1) \, (\nabla^a \lambda_m) \, (\nabla_b \nabla^b \lambda_n) \, (\nabla_c \nabla^c \sigma_2)$$

$$T[33]: -\mathcal{E}\mathcal{E}\mathcal{E}^{mnp} \, (\nabla_a \sigma_1) \, (\nabla^a \lambda_m) \, (\nabla_b \lambda_p) \, (\nabla^b \lambda_n) \, (\nabla_c \nabla^c \sigma_2)$$

$$T[48]: -3 \, \beta^m \, (\nabla_a \nabla_c \nabla^c \mathcal{J}_m) \, (\nabla^a \sigma_1) \, (\nabla_b \nabla^b \sigma_2) + \\ 3 \, \mathcal{J}^m \, (\nabla_a \nabla_c \nabla^c \beta_m) \, (\nabla^a \sigma_1) \, (\nabla_b \nabla^b \sigma_2) + 8 \, \mathcal{J}^m \, (\nabla^a \sigma_1) \, (\nabla_b \nabla^b \sigma_2) \, (\nabla_c \nabla_a \nabla^c \beta_m) + \\ 8 \, \mathcal{J}^m \, (\nabla^a \sigma_1) \, (\nabla_b \nabla^b \sigma_2) \, (\nabla_c \nabla_a \nabla^c \lambda_m) - (\nabla_a \sigma_1) \, (\nabla^a \beta^m) \, (\nabla_b \nabla^b \mathcal{J}_m) \, (\nabla_c \nabla^c \sigma_2) + \\ (\nabla_a \sigma_1) \, (\nabla^a \mathcal{J}^m) \, (\nabla_b \nabla^b \beta_m) \, (\nabla_c \nabla^c \sigma_2) + 12 \, (\nabla_a \sigma_1) \, (\nabla^a \mathcal{J}^m) \, (\nabla_b \nabla^b \lambda_m) \, (\nabla_c \nabla^c \sigma_2) - \\ 8 \, (\nabla_a \nabla_b \beta_m) \, (\nabla^a \mathcal{J}^m) \, (\nabla^b \sigma_1) \, (\nabla_c \nabla^c \sigma_2) - 16 \, (\nabla_a \nabla_b \lambda_m) \, (\nabla^a \mathcal{J}^m) \, (\nabla^b \sigma_1) \, (\nabla_c \nabla^c \sigma_2) + \\ 4 \, (\nabla_a \nabla_b \mathcal{J}_m) \, (\nabla^a \beta^m) \, (\nabla^b \sigma_1) \, (\nabla_c \nabla^c \sigma_2) + 8 \, (\nabla_a \nabla_b \mathcal{J}_m) \, (\nabla^a \lambda^m) \, (\nabla^b \sigma_1) \, (\nabla_c \nabla^c \sigma_2) + \\ 4 \, (\nabla^a \mathcal{J}^m) \, (\nabla_b \nabla_a \beta_m) \, (\nabla^b \sigma_1) \, (\nabla_c \nabla^c \sigma_2) + 8 \, (\nabla^a \mathcal{J}^m) \, (\nabla_b \nabla_a \lambda_m) \, (\nabla^b \sigma_1) \, (\nabla_c \nabla^c \sigma_2) - \\ 8 \, \mathcal{J}^m \, (\nabla^a \sigma_1) \, (\nabla_b \nabla^b \sigma_2) \, (\nabla_c \nabla^c \nabla_a \beta_m) - 8 \, \mathcal{J}^m \, (\nabla^a \sigma_1) \, (\nabla_b \nabla^b \sigma_2) \, (\nabla_c \nabla^c \nabla_a \lambda_m)$$

$$T[49]: -2 \, \mathcal{A}\mathcal{A}\text{hat}^{mn} \, \beta_m \, (\nabla_a \nabla_c \nabla^c \lambda_n) \, (\nabla^a \sigma_1) \, (\nabla_b \nabla^b \sigma_2) - 2 \, \beta^m \, (\nabla_a \sigma_1) \, (\nabla^a \mathcal{A}\mathcal{A}\text{hat}_m^n) \, (\nabla_b \nabla^b \lambda_n) \, (\nabla_c \nabla^c \sigma_2) + \\ 2 \, \mathcal{A}\mathcal{A}\text{hat}^{mn} \, (\nabla_a \sigma_1) \, (\nabla^a \beta_m) \, (\nabla_b \nabla^b \lambda_n) \, (\nabla_c \nabla^c \sigma_2) + 4 \, \mathcal{A}\mathcal{A}\text{hat}^{mn} \, (\nabla_a \sigma_1) \, (\nabla^a \lambda_m) \, (\nabla_b \nabla^b \lambda_n) \, (\nabla_c \nabla^c \sigma_2)$$

$$T[50]: \mathcal{A}\mathcal{A}\text{hat}p_m^n \, \beta^m \, (\nabla_a \nabla_c \nabla^c \lambda_n) \, (\nabla^a \sigma_1) \, (\nabla_b \nabla^b \sigma_2)$$

$$\begin{aligned}
\text{T}[54] &: \mathcal{A}\mathcal{A}\text{hatpp}^{\text{mnp}} \beta_p (\nabla_a \sigma_1) (\nabla^a \lambda_m) (\nabla_b \nabla^b \lambda_n) (\nabla_c \nabla^c \sigma_2) \\
\text{T}[55] &: \mathcal{A}\mathcal{A}\text{hatp}^{\text{np}}_m \beta^m (\nabla_a \nabla_b \lambda_p) (\nabla^a \lambda_n) (\nabla^b \sigma_1) (\nabla_c \nabla^c \sigma_2) \\
\text{T}[56] &: \mathcal{A}\mathcal{A}\text{checkp}^{\text{mnp}} (\nabla_a \sigma_1) (\nabla^a \beta_p) (\nabla_b \lambda_n) (\nabla^b \lambda_m) (\nabla_c \nabla^c \sigma_2) + \\
& 2 \mathcal{A}\mathcal{A}\text{checkp}^{\text{mnp}} (\nabla_a \lambda_n) (\nabla^a \lambda_m) (\nabla_b \sigma_1) (\nabla^b \lambda_p) (\nabla_c \nabla^c \sigma_2) - \\
& \beta^m (\nabla_a \lambda^p) (\nabla^a \lambda^n) (\nabla_b \mathcal{A}\mathcal{A}\text{checkp}_{\text{npm}}) (\nabla^b \sigma_1) (\nabla_c \nabla^c \sigma_2) - \\
& 2 \mathcal{A}\mathcal{A}\text{checkp}^{\text{np}}_m \beta^m (\nabla^a \lambda_n) (\nabla_b \nabla_a \lambda_p) (\nabla^b \sigma_1) (\nabla_c \nabla^c \sigma_2) \\
\text{T}[57] &: -\frac{1}{2} \mathcal{A}\mathcal{A}\text{checkpp}^{\text{np}}_m \beta^m (\nabla_a \sigma_1) (\nabla^a \lambda_n) (\nabla_b \nabla^b \lambda_p) (\nabla_c \nabla^c \sigma_2) + \\
& \frac{1}{2} \mathcal{A}\mathcal{A}\text{checkpp}^{\text{mnp}} (\nabla_a \lambda_m) (\nabla^a \beta_p) (\nabla_b \sigma_1) (\nabla^b \lambda_n) (\nabla_c \nabla^c \sigma_2) - \\
& \frac{1}{2} \beta^m (\nabla_a \sigma_1) (\nabla^a \lambda^n) (\nabla_b \mathcal{A}\mathcal{A}\text{checkpp}_{\text{npm}}) (\nabla^b \lambda^p) (\nabla_c \nabla^c \sigma_2) - \\
& \frac{1}{2} \mathcal{A}\mathcal{A}\text{checkpp}^{\text{np}}_m \beta^m (\nabla_a \nabla_b \lambda_p) (\nabla^a \lambda_n) (\nabla^b \sigma_1) (\nabla_c \nabla^c \sigma_2) \\
\text{Z}[4] &: 2 (\nabla_a \nabla_c \nabla^c b_{11}) (\nabla^a \sigma_1) (\nabla_b \nabla^b \sigma_2) \\
\text{Z}[16] &: 4 \mathcal{H}5^m (\nabla_a \nabla_c \nabla^c \lambda_m) (\nabla^a \sigma_1) (\nabla_b \nabla^b \sigma_2) + 4 \mathcal{H}5^m (\nabla^a \sigma_1) (\nabla_b \nabla^b \sigma_2) (\nabla_c \nabla_a \nabla^c \lambda_m) - \\
& 4 (\nabla_a \sigma_1) (\nabla^a \lambda^m) (\nabla_b \nabla^b \mathcal{H}5_m) (\nabla_c \nabla^c \sigma_2) + 8 (\nabla_a \sigma_1) (\nabla^a \mathcal{H}5^m) (\nabla_b \nabla^b \lambda_m) (\nabla_c \nabla^c \sigma_2) - \\
& 4 (\nabla_a \nabla_b \lambda_m) (\nabla^a \mathcal{H}5^m) (\nabla^b \sigma_1) (\nabla_c \nabla^c \sigma_2) + 8 (\nabla_a \nabla_b \mathcal{H}5_m) (\nabla^a \lambda^m) (\nabla^b \sigma_1) (\nabla_c \nabla^c \sigma_2) + \\
& 4 (\nabla^a \mathcal{H}5^m) (\nabla_b \nabla_a \lambda_m) (\nabla^b \sigma_1) (\nabla_c \nabla^c \sigma_2) - 4 \mathcal{H}5^m (\nabla^a \sigma_1) (\nabla_b \nabla^b \sigma_2) (\nabla_c \nabla^c \nabla_a \lambda_m) \\
\text{Z}[17] &: 2 \mathcal{H}6^m (\nabla_a \nabla_c \nabla^c \lambda_m) (\nabla^a \sigma_1) (\nabla_b \nabla^b \sigma_2) + 2 \mathcal{H}6^m (\nabla^a \sigma_1) (\nabla_b \nabla^b \sigma_2) (\nabla_c \nabla_a \nabla^c \lambda_m) - \\
& 2 (\nabla_a \sigma_1) (\nabla^a \lambda^m) (\nabla_b \nabla^b \mathcal{H}6_m) (\nabla_c \nabla^c \sigma_2) + 4 (\nabla_a \sigma_1) (\nabla^a \mathcal{H}6^m) (\nabla_b \nabla^b \lambda_m) (\nabla_c \nabla^c \sigma_2) - \\
& 2 (\nabla_a \nabla_b \lambda_m) (\nabla^a \mathcal{H}6^m) (\nabla^b \sigma_1) (\nabla_c \nabla^c \sigma_2) + 4 (\nabla_a \nabla_b \mathcal{H}6_m) (\nabla^a \lambda^m) (\nabla^b \sigma_1) (\nabla_c \nabla^c \sigma_2) + \\
& 2 (\nabla^a \mathcal{H}6^m) (\nabla_b \nabla_a \lambda_m) (\nabla^b \sigma_1) (\nabla_c \nabla^c \sigma_2) - 2 \mathcal{H}6^m (\nabla^a \sigma_1) (\nabla_b \nabla^b \sigma_2) (\nabla_c \nabla^c \nabla_a \lambda_m) \\
\text{Z}[18] &: -5 \mathcal{F}^m (\nabla_a \nabla_c \nabla^c \lambda_m) (\nabla^a \sigma_1) (\nabla_b \nabla^b \sigma_2) - \\
& (\nabla_a \sigma_1) (\nabla^a \mathcal{F}^m) (\nabla_b \nabla^b \lambda_m) (\nabla_c \nabla^c \sigma_2) - 4 (\nabla_a \nabla_b \lambda_m) (\nabla^a \mathcal{F}^m) (\nabla^b \sigma_1) (\nabla_c \nabla^c \sigma_2) \\
\text{Z}[19] &: -2 \mathcal{E}^m (\nabla_a \nabla_c \nabla^c \lambda_m) (\nabla^a \sigma_1) (\nabla_b \nabla^b \sigma_2) - 2 (\nabla_a \sigma_1) (\nabla^a \mathcal{E}^m) (\nabla_b \nabla^b \lambda_m) (\nabla_c \nabla^c \sigma_2) \\
\text{Z}[21] &: \mathcal{D}\mathcal{D}^{\text{mn}} (\nabla_a \sigma_1) (\nabla^a \lambda_m) (\nabla_b \nabla^b \lambda_n) (\nabla_c \nabla^c \sigma_2) - \mathcal{D}\mathcal{D}^{\text{mn}} (\nabla_a \nabla_b \lambda_n) (\nabla^a \lambda_m) (\nabla^b \sigma_1) (\nabla_c \nabla^c \sigma_2) \\
\text{Z}[25] &: 2 \mathcal{B}\mathcal{B}^{\text{mn}} (\nabla_a \sigma_1) (\nabla^a \lambda_m) (\nabla_b \nabla^b \lambda_n) (\nabla_c \nabla^c \sigma_2) \\
\text{Z}[26] &: -\mathcal{A}\mathcal{A}^{\text{mn}} \beta_n (\nabla_a \nabla_c \nabla^c \lambda_m) (\nabla^a \sigma_1) (\nabla_b \nabla^b \sigma_2) - \beta^m (\nabla_a \nabla_b \lambda_n) (\nabla^a \mathcal{A}\mathcal{A}_m^n) (\nabla^b \sigma_1) (\nabla_c \nabla^c \sigma_2) - \\
& \mathcal{A}\mathcal{A}^{\text{mn}} (\nabla_a \nabla_b \lambda_n) (\nabla^a \beta_m) (\nabla^b \sigma_1) (\nabla_c \nabla^c \sigma_2) + \beta^m (\nabla^a \mathcal{A}\mathcal{A}_m^n) (\nabla_b \nabla_a \lambda_n) (\nabla^b \sigma_1) (\nabla_c \nabla^c \sigma_2) \\
\text{Z}[27] &: \\
& -2 \mathcal{A}\mathcal{A}\mathbf{p}^{\text{mn}} (\nabla_a \sigma_1) (\nabla^a \beta_n) (\nabla_b \nabla^b \lambda_m) (\nabla_c \nabla^c \sigma_2) + 2 \mathcal{A}\mathcal{A}\mathbf{p}^{\text{mn}} (\nabla_a \sigma_1) (\nabla^a \lambda_m) (\nabla_b \nabla^b \lambda_n) (\nabla_c \nabla^c \sigma_2) - \\
& 2 (\nabla_a \lambda_m) (\nabla^a \mathcal{A}\mathcal{A}\mathbf{p}^{\text{mn}}) (\nabla_b \sigma_1) (\nabla^b \beta_n) (\nabla_c \nabla^c \sigma_2) + 2 (\nabla_a \beta_n) (\nabla^a \mathcal{A}\mathcal{A}\mathbf{p}^{\text{mn}}) (\nabla_b \sigma_1) (\nabla^b \lambda_m) (\nabla_c \nabla^c \sigma_2) + \\
& 2 \mathcal{A}\mathcal{A}\mathbf{p}^{\text{mn}} (\nabla_a \nabla_b \lambda_m) (\nabla^a \beta_n) (\nabla^b \sigma_1) (\nabla_c \nabla^c \sigma_2) - 2 \mathcal{A}\mathcal{A}\mathbf{p}^{\text{mn}} (\nabla_a \nabla_b \beta_n) (\nabla^a \lambda_m) (\nabla^b \sigma_1) (\nabla_c \nabla^c \sigma_2) \\
\text{Z}[28] &: \\
& -\mathcal{A}\mathcal{A}\mathcal{A}^{\text{mno}} \beta_n (\nabla_a \sigma_1) (\nabla^a \lambda_m) (\nabla_b \nabla^b \lambda_o) (\nabla_c \nabla^c \sigma_2) - \mathcal{A}\mathcal{A}\mathcal{A}^{\text{mno}} \beta_o (\nabla^a \lambda_m) (\nabla_b \nabla_a \lambda_n) (\nabla^b \sigma_1) (\nabla_c \nabla^c \sigma_2) \\
\text{Z}[29] &: -\mathcal{A}\mathcal{A}\mathbf{p}_m^{\text{no}} \beta^m (\nabla_a \nabla_b \lambda_o) (\nabla^a \lambda_n) (\nabla^b \sigma_1) (\nabla_c \nabla^c \sigma_2) \\
\text{Z}[30] &: -\frac{1}{2} \mathcal{A}\mathcal{A}\mathcal{A}^{\text{nop}}_m \beta^m (\nabla_a \lambda_o) (\nabla^a \lambda_n) (\nabla_b \sigma_1) (\nabla^b \lambda_p) (\nabla_c \nabla^c \sigma_2)
\end{aligned}$$

■ 11)  $\partial_\mu \sigma_1 \nabla_\nu \partial_\rho \sigma_2 - \partial_\mu \sigma_2 \nabla_\nu \partial_\rho \sigma_1$

T[27]:

$$8 \mathcal{HH5}^{mn} (\nabla^a \lambda_m) (\nabla_b \nabla^c \lambda_n) (\nabla^b \sigma_1) (\nabla_c \nabla_a \sigma_2) + 4 (\nabla^a \lambda^m) (\nabla_b \nabla_a \sigma_2) (\nabla^b \lambda^n) (\nabla_c \mathcal{HH5}_{mn}) (\nabla^c \sigma_1)$$

$$T[29]: -2 \mathcal{FF}^{mn} (\nabla_a \sigma_1) (\nabla^a \lambda_m) (\nabla_c \nabla_b \sigma_2) (\nabla^c \nabla^b \lambda_n)$$

$$T[30]: -2 \mathcal{FFP}^{mn} (\nabla^a \lambda_m) (\nabla_b \nabla^c \lambda_n) (\nabla^b \sigma_1) (\nabla_c \nabla_a \sigma_2)$$

$$T[31]: -\mathcal{FFF}^{mnp} (\nabla_a \sigma_1) (\nabla^a \lambda_m) (\nabla^b \lambda_n) (\nabla_c \nabla_b \sigma_2) (\nabla^c \lambda_p)$$

$$T[48]: -4 (\nabla^a \mathcal{J}^m) (\nabla_b \nabla^c \beta_m) (\nabla^b \sigma_1) (\nabla_c \nabla_a \sigma_2) - 8 (\nabla^a \mathcal{J}^m) (\nabla_b \nabla^c \lambda_m) (\nabla^b \sigma_1) (\nabla_c \nabla_a \sigma_2) - \\ 8 (\nabla_a \sigma_1) (\nabla^a \mathcal{J}^m) (\nabla_c \nabla_b \sigma_2) (\nabla^c \nabla^b \beta_m) - 16 (\nabla_a \sigma_1) (\nabla^a \mathcal{J}^m) (\nabla_c \nabla_b \sigma_2) (\nabla^c \nabla^b \lambda_m) - \\ 4 \mathcal{J}^m (\nabla^a \sigma_1) (\nabla_c \nabla_a \nabla_b \beta_m) (\nabla^c \nabla^b \sigma_2) - 8 \mathcal{J}^m (\nabla^a \sigma_1) (\nabla_c \nabla_a \nabla_b \lambda_m) (\nabla^c \nabla^b \sigma_2)$$

$$T[51]: \mathcal{Ahatpp}_m^n \beta^m (\nabla_a \nabla_c \nabla_b \lambda_n) (\nabla^a \sigma_1) (\nabla^c \nabla^b \sigma_2)$$

$$T[57]: \mathcal{AAcheckpp}^{mnp} (\nabla^a \beta_p) (\nabla_b \sigma_1) (\nabla^b \lambda_m) (\nabla_c \nabla_a \sigma_2) (\nabla^c \lambda_n) + \\ 2 \mathcal{AAcheckpp}^{mnp} (\nabla_a \sigma_1) (\nabla^a \lambda_m) (\nabla^b \lambda_n) (\nabla_c \nabla_b \sigma_2) (\nabla^c \lambda_p)$$

$$T[62]: \frac{1}{2} \mathcal{AAcheckpp}^{nop}_m \beta^m (\nabla_a \sigma_1) (\nabla^a \lambda_n) (\nabla^b \lambda_o) (\nabla_c \nabla_b \sigma_2) (\nabla^c \lambda_p)$$

$$Z[18]: -4 (\nabla_a \sigma_1) (\nabla^a \mathcal{F}^m) (\nabla_c \nabla_b \sigma_2) (\nabla^c \nabla^b \lambda_m) - 4 \mathcal{F}^m (\nabla_a \nabla_c \nabla_b \lambda_m) (\nabla^a \sigma_1) (\nabla^c \nabla^b \sigma_2)$$

$$Z[21]: -\mathcal{DD}^{mn} (\nabla^a \lambda_m) (\nabla^b \sigma_1) (\nabla_c \nabla_a \sigma_2) (\nabla^c \nabla_b \lambda_n) + \mathcal{DD}^{mn} (\nabla_a \sigma_1) (\nabla^a \lambda_m) (\nabla_c \nabla_b \sigma_2) (\nabla^c \nabla^b \lambda_n)$$

$$Z[26]: -2 \mathcal{AJ}^{mn} (\nabla^a \beta_m) (\nabla_b \nabla^c \lambda_n) (\nabla^b \sigma_1) (\nabla_c \nabla_a \sigma_2) - 4 \mathcal{AJ}^{mn} (\nabla^a \lambda_m) (\nabla_b \nabla^c \lambda_n) (\nabla^b \sigma_1) (\nabla_c \nabla_a \sigma_2)$$

Z[27]:

$$2 (\nabla^a \mathcal{AP}^{mn}) (\nabla_b \nabla_a \sigma_2) (\nabla^b \beta_n) (\nabla_c \sigma_1) (\nabla^c \lambda_m) + 4 (\nabla^a \mathcal{AP}^{mn}) (\nabla_b \sigma_1) (\nabla^b \lambda_m) (\nabla_c \nabla_a \sigma_2) (\nabla^c \lambda_n) + \\ 2 \mathcal{AP}^{mn} (\nabla^a \beta_n) (\nabla^b \sigma_1) (\nabla_c \nabla_a \sigma_2) (\nabla^c \nabla_b \lambda_m) + 4 \mathcal{AP}^{mn} (\nabla^a \lambda_n) (\nabla^b \sigma_1) (\nabla_c \nabla_a \sigma_2) (\nabla^c \nabla_b \lambda_m) - \\ 2 \mathcal{AP}^{mn} (\nabla_a \sigma_1) (\nabla^a \lambda_m) (\nabla_c \nabla_b \sigma_2) (\nabla^c \nabla^b \beta_n) - 4 \mathcal{AP}^{mn} (\nabla_a \sigma_1) (\nabla^a \lambda_m) (\nabla_c \nabla_b \sigma_2) (\nabla^c \nabla^b \lambda_n)$$

$$Z[29]: -\mathcal{AAP}^{no}_m \beta^m (\nabla^a \lambda_n) (\nabla_b \nabla^c \lambda_o) (\nabla^b \sigma_1) (\nabla_c \nabla_a \sigma_2)$$

## (1,1) terms: six consistency conditions

■ 12)  $\partial_{[\mu} \sigma_1 \partial_{\nu]} \sigma_2 R$ 

$$T[17]: 4 R[\nabla] (\nabla_a \sigma_1) (\nabla^a I6^m) (\nabla_b \sigma_2) (\nabla^b \lambda_m)$$

$$T[18]: -R[\nabla] (\nabla_a \sigma_1) (\nabla^a I7^m) (\nabla_b \sigma_2) (\nabla^b \lambda_m)$$

$$T[30]: -R[\nabla] \mathcal{F}\mathcal{F}P^{mn} (\nabla_a \sigma_1) (\nabla^a \lambda_m) (\nabla_b \sigma_2) (\nabla^b \lambda_n)$$

$$T[48]: -2 R[\nabla] (\nabla_a \sigma_1) (\nabla^a \mathcal{A}^m) (\nabla_b \sigma_2) (\nabla^b \beta_m) - 4 R[\nabla] (\nabla_a \sigma_1) (\nabla^a \mathcal{A}^m) (\nabla_b \sigma_2) (\nabla^b \lambda_m)$$

$$Z[12]: -8 R[\nabla] (\nabla_a \sigma_1) (\nabla^a \mathcal{H}1^m) (\nabla_b \sigma_2) (\nabla^b \lambda_m)$$

$$Z[13]: -\frac{4}{5} R[\nabla] (\nabla_a \sigma_1) (\nabla^a \mathcal{H}2^m) (\nabla_b \sigma_2) (\nabla^b \lambda_m)$$

$$Z[14]: -4 R[\nabla] (\nabla_a \sigma_1) (\nabla^a \mathcal{H}3^m) (\nabla_b \sigma_2) (\nabla^b \lambda_m)$$

$$Z[16]: -4 R[\nabla] (\nabla_a \sigma_1) (\nabla^a \mathcal{H}5^m) (\nabla_b \sigma_2) (\nabla^b \lambda_m)$$

$$Z[17]: -\frac{2}{5} R[\nabla] (\nabla_a \sigma_1) (\nabla^a \mathcal{H}6^m) (\nabla_b \sigma_2) (\nabla^b \lambda_m)$$

$$Z[20]: \frac{2}{5} R[\nabla] \mathcal{E}\mathcal{E}^{mn} (\nabla_a \sigma_1) (\nabla^a \lambda_m) (\nabla_b \sigma_2) (\nabla^b \lambda_n)$$

$$Z[21]: -\frac{1}{2} R[\nabla] \mathcal{D}\mathcal{D}^{mn} (\nabla_a \sigma_1) (\nabla^a \lambda_m) (\nabla_b \sigma_2) (\nabla^b \lambda_n)$$

$$Z[25]: \frac{2}{5} R[\nabla] \mathcal{B}\mathcal{B}^{mn} (\nabla_a \sigma_1) (\nabla^a \beta_m) (\nabla_b \sigma_2) (\nabla^b \lambda_n)$$

$$Z[27]: 2 R[\nabla] \mathcal{A}\mathcal{A}P^{mn} (\nabla_a \sigma_1) (\nabla^a \beta_n) (\nabla_b \sigma_2) (\nabla^b \lambda_m) - 4 R[\nabla] \mathcal{A}\mathcal{A}P^{mn} (\nabla_a \sigma_1) (\nabla^a \lambda_m) (\nabla_b \sigma_2) (\nabla^b \lambda_n)$$



■ 13)  $\partial_{[\mu} \sigma_1 \partial_{\nu]} \sigma_2 \partial^\mu R$

$$T[16]: -\frac{4}{5} I5^m (\nabla_a \sigma_1) (\nabla^a R[\nabla]) (\nabla_b \sigma_2) (\nabla^b \lambda_m)$$

$$T[17]: 4 I6^m (\nabla_a \sigma_1) (\nabla^a R[\nabla]) (\nabla_b \sigma_2) (\nabla^b \lambda_m)$$

$$T[30]: \frac{1}{2} \mathcal{F}\mathcal{F}P^{mn} \beta_n (\nabla_a \sigma_1) (\nabla^a R[\nabla]) (\nabla_b \sigma_2) (\nabla^b \lambda_m)$$

$$Z[5]: -\frac{4}{5} (\nabla_a \sigma_1) (\nabla^a R[\nabla]) (\nabla_b \sigma_2) (\nabla^b b_{12})$$

$$Z[6]: -4 (\nabla_a \sigma_1) (\nabla^a R[\nabla]) (\nabla_b \sigma_2) (\nabla^b b_{13})$$

$$Z[12]: -8 \mathcal{H}1^m (\nabla_a \sigma_1) (\nabla^a R[\nabla]) (\nabla_b \sigma_2) (\nabla^b \lambda_m)$$

$$Z[13]: -\frac{4}{5} \mathcal{H}2^m (\nabla_a \sigma_1) (\nabla^a R[\nabla]) (\nabla_b \sigma_2) (\nabla^b \lambda_m)$$

$$Z[14]: -4 \mathcal{H}3^m (\nabla_a \sigma_1) (\nabla^a R[\nabla]) (\nabla_b \sigma_2) (\nabla^b \lambda_m)$$

$$Z[17]: \frac{2}{5} \mathcal{H}6^m (\nabla_a \sigma_1) (\nabla^a R[\nabla]) (\nabla_b \sigma_2) (\nabla^b \lambda_m)$$

$$Z[18]: -\mathcal{F}^m (\nabla_a \sigma_1) (\nabla^a R[\nabla]) (\nabla_b \sigma_2) (\nabla^b \beta_m)$$

$$Z[19]: -\frac{2}{5} \mathcal{E}^m (\nabla_a \sigma_1) (\nabla^a R[\nabla]) (\nabla_b \sigma_2) (\nabla^b \beta_m) - \frac{4}{5} \mathcal{E}^m (\nabla_a \sigma_1) (\nabla^a R[\nabla]) (\nabla_b \sigma_2) (\nabla^b \lambda_m)$$

$$Z[20]: \frac{1}{5} \mathcal{E}\mathcal{E}^{mn} \beta_n (\nabla_a \sigma_1) (\nabla^a R[\nabla]) (\nabla_b \sigma_2) (\nabla^b \lambda_m)$$

■ 14)  $\partial_{[\nu} \sigma_1 \partial_{\rho]} \sigma_2 G^{\mu\nu}$

$$\begin{aligned}
T[17] &: -8 G[\nabla]^{ab} (\nabla_a \lambda_m) (\nabla_b \sigma_1) (\nabla_c \sigma_2) (\nabla^c I6^m) - 8 G[\nabla]^{ab} I6^m (\nabla_a \sigma_1) (\nabla_c \nabla_b \lambda_m) (\nabla^c \sigma_2) \\
T[18] &: 2 G[\nabla]^{ab} (\nabla_a \lambda_m) (\nabla_b \sigma_1) (\nabla_c \sigma_2) (\nabla^c I7^m) + 2 G[\nabla]^{ab} I7^m (\nabla_a \sigma_1) (\nabla_c \nabla_b \lambda_m) (\nabla^c \sigma_2) \\
T[23] &: 16 G[\nabla]^{ab} \mathcal{HH}1^{mn} (\nabla_a \lambda_m) (\nabla_b \sigma_1) (\nabla_c \sigma_2) (\nabla^c \lambda_n) \\
T[25] &: 4 G[\nabla]^{ab} \mathcal{HH}3^{mn} (\nabla_a \lambda_m) (\nabla_b \sigma_1) (\nabla_c \sigma_2) (\nabla^c \lambda_n) \\
T[26] &: -G[\nabla]^{ab} \mathcal{HH}4^{mn} (\nabla_a \lambda_m) (\nabla_b \sigma_1) (\nabla_c \sigma_2) (\nabla^c \lambda_n) \\
T[27] &: -4 G[\nabla]^{ab} \mathcal{HH}5^{mn} (\nabla_a \lambda_m) (\nabla_b \sigma_1) (\nabla_c \sigma_2) (\nabla^c \lambda_n) \\
T[30] &: 2 G[\nabla]^{ab} \mathcal{FF}P^{mn} (\nabla_a \lambda_n) (\nabla_b \sigma_1) (\nabla_c \sigma_2) (\nabla^c \lambda_m) \\
T[37] &: -\frac{1}{2} G[\nabla]^{ab} C\mathcal{C}hatP_m^n \beta^m (\nabla_a \sigma_1) (\nabla_c \nabla_b \lambda_n) (\nabla^c \sigma_2) \\
T[38] &: -\frac{1}{4} G[\nabla]^{ab} C\mathcal{C}C^{np}_m \beta^m (\nabla_a \lambda_n) (\nabla_b \sigma_1) (\nabla_c \sigma_2) (\nabla^c \lambda_p) \\
T[39] &: -\frac{1}{2} G[\nabla]^{ab} C\mathcal{C}C\mathcal{P}^{mnp} \beta_p (\nabla_a \lambda_m) (\nabla_b \sigma_1) (\nabla_c \sigma_2) (\nabla^c \lambda_n) \\
T[48] &: 4 G[\nabla]^{ab} (\nabla_a \beta_m) (\nabla_b \sigma_1) (\nabla_c \sigma_2) (\nabla^c \mathcal{A}^m) + 8 G[\nabla]^{ab} (\nabla_a \lambda_m) (\nabla_b \sigma_1) (\nabla_c \sigma_2) (\nabla^c \mathcal{A}^m) + \\
& 4 G[\nabla]^{ab} \mathcal{A}^m (\nabla_a \sigma_1) (\nabla_c \nabla_b \beta_m) (\nabla^c \sigma_2) + 8 G[\nabla]^{ab} \mathcal{A}^m (\nabla_a \sigma_1) (\nabla_c \nabla_b \lambda_m) (\nabla^c \sigma_2) \\
Z[12] &: 16 G[\nabla]^{ab} (\nabla_a \lambda_m) (\nabla_b \sigma_1) (\nabla_c \sigma_2) (\nabla^c \mathcal{H}1^m) - 16 G[\nabla]^{ab} (\nabla_a \mathcal{H}1^m) (\nabla_b \sigma_1) (\nabla_c \sigma_2) (\nabla^c \lambda_m) \\
Z[14] &: 4 G[\nabla]^{ab} (\nabla_a \lambda_m) (\nabla_b \sigma_1) (\nabla_c \sigma_2) (\nabla^c \mathcal{H}3^m) - 4 G[\nabla]^{ab} (\nabla_a \mathcal{H}3^m) (\nabla_b \sigma_1) (\nabla_c \sigma_2) (\nabla^c \lambda_m) \\
Z[15] &: -G[\nabla]^{ab} (\nabla_a \lambda_m) (\nabla_b \sigma_1) (\nabla_c \sigma_2) (\nabla^c \mathcal{H}4^m) + G[\nabla]^{ab} (\nabla_a \mathcal{H}4^m) (\nabla_b \sigma_1) (\nabla_c \sigma_2) (\nabla^c \lambda_m) \\
Z[16] &: 4 G[\nabla]^{ab} (\nabla_a \lambda_m) (\nabla_b \sigma_1) (\nabla_c \sigma_2) (\nabla^c \mathcal{H}5^m) - 4 G[\nabla]^{ab} (\nabla_a \mathcal{H}5^m) (\nabla_b \sigma_1) (\nabla_c \sigma_2) (\nabla^c \lambda_m) \\
Z[18] &: 4 G[\nabla]^{ab} \mathcal{F}^m (\nabla_a \sigma_1) (\nabla_c \nabla_b \lambda_m) (\nabla^c \sigma_2) \\
Z[21] &: -G[\nabla]^{ab} \mathcal{D}\mathcal{D}^{mn} (\nabla_a \lambda_m) (\nabla_b \sigma_1) (\nabla_c \sigma_2) (\nabla^c \lambda_n) \\
Z[22] &: G[\nabla]^{ab} (\nabla_a C^m) (\nabla_b \sigma_1) (\nabla_c \sigma_2) (\nabla^c \beta_m) + 2 G[\nabla]^{ab} (\nabla_a C^m) (\nabla_b \sigma_1) (\nabla_c \sigma_2) (\nabla^c \lambda_m) \\
Z[23] &: \frac{1}{2} G[\nabla]^{ab} C\mathcal{C}^{mn} (\nabla_a \lambda_n) (\nabla_b \sigma_1) (\nabla_c \sigma_2) (\nabla^c \lambda_m) + \\
& \frac{1}{2} G[\nabla]^{ab} \beta^m (\nabla_a C\mathcal{C}^n_m) (\nabla_b \sigma_1) (\nabla_c \sigma_2) (\nabla^c \lambda_n) - \frac{1}{2} G[\nabla]^{ab} C\mathcal{C}^{mn} (\nabla_a \lambda_m) (\nabla_b \sigma_1) (\nabla_c \sigma_2) (\nabla^c \lambda_n) + \\
& \frac{1}{2} G[\nabla]^{ab} C\mathcal{C}^{mn} \beta_n (\nabla_a \sigma_1) (\nabla_c \nabla_b \lambda_m) (\nabla^c \sigma_2) - \frac{1}{2} G[\nabla]^{ab} C\mathcal{C}^{mn} \beta_m (\nabla_a \sigma_1) (\nabla_c \nabla_b \lambda_n) (\nabla^c \sigma_2) \\
Z[24] &: \\
& -G[\nabla]^{ab} C\mathcal{C}P^{mn} (\nabla_a \lambda_m) (\nabla_b \sigma_1) (\nabla_c \sigma_2) (\nabla^c \beta_n) - 2 G[\nabla]^{ab} C\mathcal{C}P^{mn} (\nabla_a \lambda_m) (\nabla_b \sigma_1) (\nabla_c \sigma_2) (\nabla^c \lambda_n) \\
Z[27] &: -2 G[\nabla]^{ab} \mathcal{A}\mathcal{A}P^{mn} (\nabla_a \lambda_m) (\nabla_b \sigma_1) (\nabla_c \sigma_2) (\nabla^c \beta_n) + \\
& 4 G[\nabla]^{ab} \mathcal{A}\mathcal{A}P^{mn} (\nabla_a \beta_n) (\nabla_b \sigma_1) (\nabla_c \sigma_2) (\nabla^c \lambda_m) + \\
& 8 G[\nabla]^{ab} \mathcal{A}\mathcal{A}P^{mn} (\nabla_a \lambda_n) (\nabla_b \sigma_1) (\nabla_c \sigma_2) (\nabla^c \lambda_m) - 4 G[\nabla]^{ab} \mathcal{A}\mathcal{A}P^{mn} (\nabla_a \lambda_m) (\nabla_b \sigma_1) (\nabla_c \sigma_2) (\nabla^c \lambda_n)
\end{aligned}$$

■ 15)  $\partial_{[\nu} \sigma_1 \partial_{\rho]} \sigma_2 \nabla^\nu G^{\mu\rho}$

$$\begin{aligned}
\text{T}[17]: & 4 \text{I}6^{\text{m}} (\nabla^a \lambda_{\text{m}}) (\nabla_b G[\nabla]_{\text{ac}}) (\nabla^b \sigma_1) (\nabla^c \sigma_2) - 4 \text{I}6^{\text{m}} (\nabla^a \lambda_{\text{m}}) (\nabla^b \sigma_1) (\nabla_c G[\nabla]_{\text{ab}}) (\nabla^c \sigma_2) \\
\text{T}[18]: & - \text{I}7^{\text{m}} (\nabla^a \lambda_{\text{m}}) (\nabla_b G[\nabla]_{\text{ac}}) (\nabla^b \sigma_1) (\nabla^c \sigma_2) + \text{I}7^{\text{m}} (\nabla^a \lambda_{\text{m}}) (\nabla^b \sigma_1) (\nabla_c G[\nabla]_{\text{ab}}) (\nabla^c \sigma_2) \\
\text{T}[30]: & \frac{1}{2} \mathcal{FFP}^{\text{mn}} \beta_{\text{n}} (\nabla^a \lambda_{\text{m}}) (\nabla_b G[\nabla]_{\text{ac}}) (\nabla^b \sigma_1) (\nabla^c \sigma_2) - \frac{1}{2} \mathcal{FFP}^{\text{mn}} \beta_{\text{n}} (\nabla^a \lambda_{\text{m}}) (\nabla^b \sigma_1) (\nabla_c G[\nabla]_{\text{ab}}) (\nabla^c \sigma_2) \\
\text{Z}[6]: & -4 (\nabla^a b_{13}) (\nabla_b G[\nabla]_{\text{ac}}) (\nabla^b \sigma_1) (\nabla^c \sigma_2) + 4 (\nabla^a b_{13}) (\nabla^b \sigma_1) (\nabla_c G[\nabla]_{\text{ab}}) (\nabla^c \sigma_2) \\
\text{Z}[7]: & (\nabla^a b_{14}) (\nabla_b G[\nabla]_{\text{ac}}) (\nabla^b \sigma_1) (\nabla^c \sigma_2) - (\nabla^a b_{14}) (\nabla^b \sigma_1) (\nabla_c G[\nabla]_{\text{ab}}) (\nabla^c \sigma_2) \\
\text{Z}[12]: & -16 \mathcal{H}1^{\text{m}} (\nabla^a \lambda_{\text{m}}) (\nabla_b G[\nabla]_{\text{ac}}) (\nabla^b \sigma_1) (\nabla^c \sigma_2) + 16 \mathcal{H}1^{\text{m}} (\nabla^a \lambda_{\text{m}}) (\nabla^b \sigma_1) (\nabla_c G[\nabla]_{\text{ab}}) (\nabla^c \sigma_2) \\
\text{Z}[14]: & -4 \mathcal{H}3^{\text{m}} (\nabla^a \lambda_{\text{m}}) (\nabla_b G[\nabla]_{\text{ac}}) (\nabla^b \sigma_1) (\nabla^c \sigma_2) + 4 \mathcal{H}3^{\text{m}} (\nabla^a \lambda_{\text{m}}) (\nabla^b \sigma_1) (\nabla_c G[\nabla]_{\text{ab}}) (\nabla^c \sigma_2) \\
\text{Z}[15]: & \mathcal{H}4^{\text{m}} (\nabla^a \lambda_{\text{m}}) (\nabla_b G[\nabla]_{\text{ac}}) (\nabla^b \sigma_1) (\nabla^c \sigma_2) - \mathcal{H}4^{\text{m}} (\nabla^a \lambda_{\text{m}}) (\nabla^b \sigma_1) (\nabla_c G[\nabla]_{\text{ab}}) (\nabla^c \sigma_2) \\
\text{Z}[16]: & 2 \mathcal{H}5^{\text{m}} (\nabla^a \lambda_{\text{m}}) (\nabla_b G[\nabla]_{\text{ac}}) (\nabla^b \sigma_1) (\nabla^c \sigma_2) - 2 \mathcal{H}5^{\text{m}} (\nabla^a \lambda_{\text{m}}) (\nabla^b \sigma_1) (\nabla_c G[\nabla]_{\text{ab}}) (\nabla^c \sigma_2) \\
\text{Z}[18]: & -2 \mathcal{F}^{\text{m}} (\nabla^a \beta_{\text{m}}) (\nabla_b G[\nabla]_{\text{ac}}) (\nabla^b \sigma_1) (\nabla^c \sigma_2) + 2 \mathcal{F}^{\text{m}} (\nabla^a \lambda_{\text{m}}) (\nabla_b G[\nabla]_{\text{ac}}) (\nabla^b \sigma_1) (\nabla^c \sigma_2) + \\
& 2 \mathcal{F}^{\text{m}} (\nabla^a \beta_{\text{m}}) (\nabla^b \sigma_1) (\nabla_c G[\nabla]_{\text{ab}}) (\nabla^c \sigma_2) - 2 \mathcal{F}^{\text{m}} (\nabla^a \lambda_{\text{m}}) (\nabla^b \sigma_1) (\nabla_c G[\nabla]_{\text{ab}}) (\nabla^c \sigma_2)
\end{aligned}$$

■ 16)  $\partial_{[\nu} \sigma_1 \partial_{\rho]} \sigma_2 R^{\mu\nu\rho\sigma}$

$$\begin{aligned}
\text{T}[18]: & -4 R[\nabla]^{\text{abcd}} (\nabla_a \text{I}7^{\text{m}}) (\nabla_b \sigma_1) (\nabla_c \lambda_{\text{m}}) (\nabla_d \sigma_2) \\
\text{T}[34]: & -R[\nabla]^{\text{abcd}} \mathcal{DDD}^{\text{mnp}} \beta_{\text{p}} (\nabla_a \lambda_{\text{m}}) (\nabla_b \sigma_1) (\nabla_c \lambda_{\text{n}}) (\nabla_d \sigma_2) \\
\text{Z}[21]: & R[\nabla]^{\text{abcd}} \mathcal{DD}^{\text{mn}} (\nabla_a \beta_{\text{n}}) (\nabla_b \sigma_1) (\nabla_c \lambda_{\text{m}}) (\nabla_d \sigma_2) + \\
& R[\nabla]^{\text{abcd}} \mathcal{DD}^{\text{mn}} (\nabla_a \lambda_{\text{m}}) (\nabla_b \sigma_1) (\nabla_c \lambda_{\text{n}}) (\nabla_d \sigma_2) + 2 R[\nabla]^{\text{abcd}} \mathcal{DD}^{\text{mn}} (\nabla_a \beta_{\text{n}}) (\nabla_b \lambda_{\text{m}}) (\nabla_c \sigma_1) (\nabla_d \sigma_2) + \\
& 2 R[\nabla]^{\text{abcd}} \mathcal{DD}^{\text{mn}} (\nabla_a \lambda_{\text{m}}) (\nabla_b \lambda_{\text{n}}) (\nabla_c \sigma_1) (\nabla_d \sigma_2)
\end{aligned}$$

■ 17)  $\partial_{[\mu} \sigma_1 \partial_{\nu]} \sigma_2$

$$\begin{aligned}
\text{T}[27]: & 4 \mathcal{HH}5^{\text{mn}} (\nabla_a \sigma_1) (\nabla^a \lambda_{\text{m}}) (\nabla_b \nabla_c \nabla^c \lambda_{\text{n}}) (\nabla^b \sigma_2) + 8 (\nabla_a \sigma_1) (\nabla^a \lambda_{\text{m}}) (\nabla^b \sigma_2) (\nabla_c \nabla_b \lambda_{\text{n}}) (\nabla^c \mathcal{HH}5^{\text{mn}}) \\
\text{T}[29]: & 2 \mathcal{FF}^{\text{mn}} (\nabla_a \nabla_b \lambda_{\text{n}}) (\nabla^a \sigma_1) (\nabla^b \sigma_2) (\nabla_c \nabla^c \lambda_{\text{m}}) - 2 \mathcal{FF}^{\text{mn}} (\nabla^a \sigma_1) (\nabla_b \nabla_a \lambda_{\text{n}}) (\nabla^b \sigma_2) (\nabla_c \nabla^c \lambda_{\text{m}}) + \\
& 2 \mathcal{FF}^{\text{mn}} (\nabla_a \nabla_b \nabla_c \lambda_{\text{n}}) (\nabla^a \lambda_{\text{m}}) (\nabla^b \sigma_1) (\nabla^c \sigma_2) - 2 \mathcal{FF}^{\text{mn}} (\nabla_a \nabla_c \nabla_b \lambda_{\text{n}}) (\nabla^a \lambda_{\text{m}}) (\nabla^b \sigma_1) (\nabla^c \sigma_2) + \\
& 2 (\nabla_a \lambda_{\text{m}}) (\nabla^a \mathcal{FF}^{\text{mn}}) (\nabla_b \nabla_c \lambda_{\text{n}}) (\nabla^b \sigma_1) (\nabla^c \sigma_2) - 2 (\nabla_a \lambda_{\text{m}}) (\nabla^a \mathcal{FF}^{\text{mn}}) (\nabla^b \sigma_1) (\nabla_c \nabla_b \lambda_{\text{n}}) (\nabla^c \sigma_2) \\
\text{T}[30]: & -2 \mathcal{FFP}^{\text{mn}} (\nabla_a \sigma_1) (\nabla^a \lambda_{\text{m}}) (\nabla_b \nabla_c \nabla^c \lambda_{\text{n}}) (\nabla^b \sigma_2) - 2 (\nabla_a \nabla_c \lambda_{\text{n}}) (\nabla^a \mathcal{FFP}^{\text{mn}}) (\nabla_b \sigma_1) (\nabla^b \lambda_{\text{m}}) (\nabla^c \sigma_2) - \\
& 2 \mathcal{FFP}^{\text{mn}} (\nabla^a \sigma_1) (\nabla^b \sigma_2) (\nabla_c \nabla_b \lambda_{\text{n}}) (\nabla^c \nabla_a \lambda_{\text{m}}) + 2 \mathcal{FFP}^{\text{mn}} (\nabla^a \sigma_1) (\nabla^b \sigma_2) (\nabla_c \nabla_a \lambda_{\text{n}}) (\nabla^c \nabla_b \lambda_{\text{m}}) \\
\text{T}[31]: & -2 \mathcal{FF}^{\text{mnp}} (\nabla_a \nabla_c \lambda_{\text{p}}) (\nabla^a \lambda_{\text{m}}) (\nabla_b \sigma_1) (\nabla^b \lambda_{\text{n}}) (\nabla^c \sigma_2) \\
\text{T}[34]: & \mathcal{DDD}^{\text{mnp}} (\nabla_a \sigma_1) (\nabla^a \lambda_{\text{m}}) (\nabla_b \sigma_2) (\nabla^b \lambda_{\text{n}}) (\nabla_c \nabla^c \lambda_{\text{p}}) - \\
& \mathcal{DDD}^{\text{mnp}} (\nabla_a \sigma_1) (\nabla^a \lambda_{\text{m}}) (\nabla_b \nabla_c \lambda_{\text{p}}) (\nabla^b \lambda_{\text{n}}) (\nabla^c \sigma_2) - \\
& \mathcal{DDD}^{\text{mnp}} (\nabla_a \lambda_{\text{n}}) (\nabla^a \lambda_{\text{m}}) (\nabla_b \nabla_c \lambda_{\text{p}}) (\nabla^b \sigma_1) (\nabla^c \sigma_2) - \\
& \mathcal{DDD}^{\text{mnp}} (\nabla^a \lambda_{\text{m}}) (\nabla_b \sigma_1) (\nabla^b \lambda_{\text{n}}) (\nabla_c \nabla_a \lambda_{\text{p}}) (\nabla^c \sigma_2) + \\
& \mathcal{DDD}^{\text{mnp}} (\nabla_a \lambda_{\text{n}}) (\nabla^a \lambda_{\text{m}}) (\nabla^b \sigma_1) (\nabla_c \nabla_b \lambda_{\text{p}}) (\nabla^c \sigma_2) \\
\text{T}[36]: & -2 \mathcal{CChat}^{\text{mn}} (\nabla_a \nabla_b \lambda_{\text{m}}) (\nabla^a \sigma_1) (\nabla^b \sigma_2) (\nabla_c \nabla^c \lambda_{\text{n}}) + 2 \mathcal{CChat}^{\text{mn}} (\nabla^a \sigma_1) (\nabla_b \nabla_a \lambda_{\text{m}}) (\nabla^b \sigma_2) (\nabla_c \nabla^c \lambda_{\text{n}})
\end{aligned}$$

$$\begin{aligned}
\text{T[38]: } & CCC^{mnp} (\nabla_a \sigma_1) (\nabla^a \lambda_m) (\nabla_b \nabla_c \lambda_p) (\nabla^b \lambda_n) (\nabla^c \sigma_2) \\
\text{T[39]: } & 2 CCCp^{mnp} (\nabla_a \sigma_1) (\nabla^a \lambda_m) (\nabla^b \lambda_n) (\nabla_c \nabla_b \lambda_p) (\nabla^c \sigma_2) \\
\text{T[40]: } & - CCCpp^{mnp} (\nabla_a \lambda_n) (\nabla^a \lambda_m) (\nabla_b \nabla_c \lambda_p) (\nabla^b \sigma_1) (\nabla^c \sigma_2) + \\
& CCCpp^{mnp} (\nabla_a \lambda_n) (\nabla^a \lambda_m) (\nabla^b \sigma_1) (\nabla_c \nabla_b \lambda_p) (\nabla^c \sigma_2) \\
\text{T[48]: } & 4 (\nabla_a \sigma_1) (\nabla^a \beta^m) (\nabla_b \nabla_c \nabla^c \mathcal{A}_m) (\nabla^b \sigma_2) + 8 (\nabla_a \sigma_1) (\nabla^a \lambda^m) (\nabla_b \nabla_c \nabla^c \mathcal{A}_m) (\nabla^b \sigma_2) \\
\text{T[49]: } & 4 \mathcal{A}\mathcal{A}\mathcal{A}\mathcal{A}t^{mn} (\nabla_a \sigma_1) (\nabla^a \beta_m) (\nabla_b \nabla_c \nabla^c \lambda_n) (\nabla^b \sigma_2) + 8 \mathcal{A}\mathcal{A}\mathcal{A}\mathcal{A}t^{mn} (\nabla_a \sigma_1) (\nabla^a \lambda_m) (\nabla_b \nabla_c \nabla^c \lambda_n) (\nabla^b \sigma_2) \\
\text{T[50]: } & -2 \mathcal{A}\mathcal{A}\mathcal{A}\mathcal{A}t^{mn} (\nabla_a \sigma_1) (\nabla^a \beta_m) (\nabla_b \nabla_c \nabla^c \lambda_n) (\nabla^b \sigma_2) - 4 \mathcal{A}\mathcal{A}\mathcal{A}\mathcal{A}t^{mn} (\nabla_a \sigma_1) (\nabla^a \lambda_m) (\nabla_b \nabla_c \nabla^c \lambda_n) (\nabla^b \sigma_2) \\
\text{T[51]: } & - \mathcal{A}\mathcal{A}\mathcal{A}\mathcal{A}t^{pp}_m{}^n \beta^m (\nabla_a \nabla_b \nabla_c \nabla^c \lambda_n) (\nabla^a \sigma_1) (\nabla^b \sigma_2) + \\
& \mathcal{A}\mathcal{A}\mathcal{A}\mathcal{A}t^{pp}_m{}^n \beta^m (\nabla^a \sigma_1) (\nabla_b \nabla_a \nabla_c \nabla^c \lambda_n) (\nabla^b \sigma_2) - \mathcal{A}\mathcal{A}\mathcal{A}\mathcal{A}t^{pp}_{mn} (\nabla_a \sigma_1) (\nabla^a \lambda_m) (\nabla_b \nabla_c \nabla^c \lambda_n) (\nabla^b \sigma_2) - \\
& \beta^m (\nabla^a \sigma_1) (\nabla^b \sigma_2) (\nabla_c \nabla_a \nabla_b \lambda_n) (\nabla^c \mathcal{A}\mathcal{A}\mathcal{A}\mathcal{A}t^{pp}_m{}^n) + \beta^m (\nabla^a \sigma_1) (\nabla^b \sigma_2) (\nabla_c \nabla_b \nabla_a \lambda_n) (\nabla^c \mathcal{A}\mathcal{A}\mathcal{A}\mathcal{A}t^{pp}_m{}^n) + \\
& \mathcal{A}\mathcal{A}\mathcal{A}\mathcal{A}t^{pp}_{mn} (\nabla^a \beta_m) (\nabla_b \nabla_a \nabla_c \lambda_n) (\nabla^b \sigma_1) (\nabla^c \sigma_2) - \mathcal{A}\mathcal{A}\mathcal{A}\mathcal{A}t^{pp}_{mn} (\nabla^a \lambda_m) (\nabla_b \nabla_a \nabla_c \lambda_n) (\nabla^b \sigma_1) (\nabla^c \sigma_2) + \\
& \mathcal{A}\mathcal{A}\mathcal{A}\mathcal{A}t^{pp}_{mn} (\nabla^a \beta_m) (\nabla_b \nabla_c \nabla_a \lambda_n) (\nabla^b \sigma_1) (\nabla^c \sigma_2) - \mathcal{A}\mathcal{A}\mathcal{A}\mathcal{A}t^{pp}_{mn} (\nabla^a \lambda_m) (\nabla_b \nabla_c \nabla_a \lambda_n) (\nabla^b \sigma_1) (\nabla^c \sigma_2) - \\
& \mathcal{A}\mathcal{A}\mathcal{A}\mathcal{A}t^{pp}_{mn} (\nabla^a \beta_m) (\nabla^b \sigma_1) (\nabla_c \nabla_a \nabla_b \lambda_n) (\nabla^c \sigma_2) + \mathcal{A}\mathcal{A}\mathcal{A}\mathcal{A}t^{pp}_{mn} (\nabla^a \lambda_m) (\nabla^b \sigma_1) (\nabla_c \nabla_a \nabla_b \lambda_n) (\nabla^c \sigma_2) - \\
& \mathcal{A}\mathcal{A}\mathcal{A}\mathcal{A}t^{pp}_{mn} (\nabla^a \beta_m) (\nabla^b \sigma_1) (\nabla_c \nabla_b \nabla_a \lambda_n) (\nabla^c \sigma_2) + \mathcal{A}\mathcal{A}\mathcal{A}\mathcal{A}t^{pp}_{mn} (\nabla^a \lambda_m) (\nabla^b \sigma_1) (\nabla_c \nabla_b \nabla_a \lambda_n) (\nabla^c \sigma_2) \\
\text{T[53]: } & \mathcal{A}\mathcal{A}\mathcal{A}\mathcal{A}t^{np}_m \beta^m (\nabla_a \nabla_b \lambda_n) (\nabla^a \sigma_1) (\nabla^b \sigma_2) (\nabla_c \nabla^c \lambda_p) - \\
& \mathcal{A}\mathcal{A}\mathcal{A}\mathcal{A}t^{np}_m \beta^m (\nabla^a \sigma_1) (\nabla_b \nabla_a \lambda_n) (\nabla^b \sigma_2) (\nabla_c \nabla^c \lambda_p) \\
\text{T[54]: } & -2 \mathcal{A}\mathcal{A}\mathcal{A}\mathcal{A}t^{mnp} (\nabla_a \sigma_1) (\nabla^a \beta_p) (\nabla_b \sigma_2) (\nabla^b \lambda_m) (\nabla_c \nabla^c \lambda_n) - \\
& 4 \mathcal{A}\mathcal{A}\mathcal{A}\mathcal{A}t^{mnp} (\nabla_a \sigma_1) (\nabla^a \lambda_m) (\nabla_b \sigma_2) (\nabla^b \lambda_p) (\nabla_c \nabla^c \lambda_n) \\
\text{T[55]: } & - \mathcal{A}\mathcal{A}\mathcal{A}\mathcal{A}t^{np}_m \beta^m (\nabla_a \sigma_1) (\nabla^a \lambda_n) (\nabla_b \nabla_c \nabla^c \lambda_p) (\nabla^b \sigma_2) - \\
& 2 \mathcal{A}\mathcal{A}\mathcal{A}\mathcal{A}t^{mnp} (\nabla_a \sigma_1) (\nabla^a \beta_p) (\nabla_b \nabla_c \lambda_n) (\nabla^b \lambda_m) (\nabla^c \sigma_2) - \\
& 4 \mathcal{A}\mathcal{A}\mathcal{A}\mathcal{A}t^{mnp} (\nabla_a \nabla_c \lambda_n) (\nabla^a \lambda_m) (\nabla_b \sigma_1) (\nabla^b \lambda_p) (\nabla^c \sigma_2) \\
\text{T[56]: } & 4 (\nabla_a \lambda^n) (\nabla^a \lambda^m) (\nabla_b \sigma_1) (\nabla^b \lambda^p) (\nabla_c \mathcal{A}\mathcal{A}\mathcal{A}\mathcal{A}checkp_{mnp}) (\nabla^c \sigma_2) + \\
& 2 (\nabla_a \sigma_1) (\nabla^a \beta^m) (\nabla_b \lambda^p) (\nabla^b \lambda^n) (\nabla_c \mathcal{A}\mathcal{A}\mathcal{A}\mathcal{A}checkp_{nmp}) (\nabla^c \sigma_2) + \\
& 8 \mathcal{A}\mathcal{A}\mathcal{A}\mathcal{A}checkp^{mnp} (\nabla^a \lambda_m) (\nabla_b \sigma_1) (\nabla^b \lambda_p) (\nabla_c \nabla_a \lambda_n) (\nabla^c \sigma_2) + \\
& 4 \mathcal{A}\mathcal{A}\mathcal{A}\mathcal{A}checkp^{mnp} (\nabla_a \sigma_1) (\nabla^a \beta_p) (\nabla^b \lambda_m) (\nabla_c \nabla_b \lambda_n) (\nabla^c \sigma_2) \\
\text{T[57]: } & \mathcal{A}\mathcal{A}\mathcal{A}\mathcal{A}checkpp^{mnp} (\nabla_a \sigma_1) (\nabla^a \beta_p) (\nabla_b \sigma_2) (\nabla^b \lambda_m) (\nabla_c \nabla^c \lambda_n) + \\
& 2 \mathcal{A}\mathcal{A}\mathcal{A}\mathcal{A}checkpp^{mnp} (\nabla_a \sigma_1) (\nabla^a \lambda_m) (\nabla_b \sigma_2) (\nabla^b \lambda_p) (\nabla_c \nabla^c \lambda_n) + \\
& 2 (\nabla_a \sigma_1) (\nabla^a \lambda^m) (\nabla_b \sigma_2) (\nabla^b \lambda^n) (\nabla_c \mathcal{A}\mathcal{A}\mathcal{A}\mathcal{A}checkpp_{mpn}) (\nabla^c \lambda^p) + \\
& (\nabla_a \sigma_1) (\nabla^a \beta^m) (\nabla_b \sigma_2) (\nabla^b \lambda^n) (\nabla_c \mathcal{A}\mathcal{A}\mathcal{A}\mathcal{A}checkpp_{nmp}) (\nabla^c \lambda^p) - \\
& 2 (\nabla_a \sigma_1) (\nabla^a \lambda^m) (\nabla_b \sigma_2) (\nabla^b \lambda^n) (\nabla_c \mathcal{A}\mathcal{A}\mathcal{A}\mathcal{A}checkpp_{nmp}) (\nabla^c \lambda^p) + \\
& \mathcal{A}\mathcal{A}\mathcal{A}\mathcal{A}checkpp^{mnp} (\nabla_a \sigma_1) (\nabla^a \beta_p) (\nabla_b \nabla_c \lambda_n) (\nabla^b \lambda_m) (\nabla^c \sigma_2) - \\
& \mathcal{A}\mathcal{A}\mathcal{A}\mathcal{A}checkpp^{mnp} (\nabla_a \sigma_1) (\nabla^a \lambda_m) (\nabla_b \nabla_c \beta_p) (\nabla^b \lambda_n) (\nabla^c \sigma_2) - \\
& 2 \mathcal{A}\mathcal{A}\mathcal{A}\mathcal{A}checkpp^{mnp} (\nabla_a \sigma_1) (\nabla^a \lambda_m) (\nabla_b \nabla_c \lambda_p) (\nabla^b \lambda_n) (\nabla^c \sigma_2) + \\
& 2 \mathcal{A}\mathcal{A}\mathcal{A}\mathcal{A}checkpp^{mnp} (\nabla_a \nabla_c \lambda_n) (\nabla^a \lambda_m) (\nabla_b \sigma_1) (\nabla^b \lambda_p) (\nabla^c \sigma_2)
\end{aligned}$$



$$\begin{aligned}
Z[29]: & - \mathcal{R}\mathcal{R}\mathcal{P}_m^{no} \beta^m (\nabla_a \nabla^c \lambda_n) (\nabla^a \sigma_1) (\nabla_b \nabla_c \lambda_o) (\nabla^b \sigma_2) + \\
& \mathcal{R}\mathcal{R}\mathcal{P}_m^{no} \beta^m (\nabla_a \nabla_c \lambda_o) (\nabla^a \sigma_1) (\nabla_b \nabla^c \lambda_n) (\nabla^b \sigma_2) - \\
& \mathcal{R}\mathcal{R}\mathcal{P}_m^{no} \beta^m (\nabla^a \sigma_1) (\nabla_b \nabla^c \lambda_n) (\nabla^b \sigma_2) (\nabla_c \nabla_a \lambda_o) + \\
& \mathcal{R}\mathcal{R}\mathcal{P}_m^{no} \beta^m (\nabla_a \nabla^c \lambda_n) (\nabla^a \sigma_1) (\nabla^b \sigma_2) (\nabla_c \nabla_b \lambda_o) + \\
2 & \mathcal{R}\mathcal{R}\mathcal{P}^{mno} (\nabla_a \sigma_1) (\nabla^a \lambda_m) (\nabla_b \nabla_c \lambda_o) (\nabla^b \lambda_n) (\nabla^c \sigma_2) + \\
& \beta^m (\nabla_a \nabla_c \lambda_o) (\nabla^a \lambda^n) (\nabla_b \mathcal{R}\mathcal{R}\mathcal{P}_{mn}^o) (\nabla^b \sigma_1) (\nabla^c \sigma_2) + \\
& \mathcal{R}\mathcal{R}\mathcal{P}_m^{no} \beta^m (\nabla^a \lambda_n) (\nabla_b \nabla_a \nabla_c \lambda_o) (\nabla^b \sigma_1) (\nabla^c \sigma_2) - \\
& \mathcal{R}\mathcal{R}\mathcal{P}^{mno} (\nabla_a \lambda_m) (\nabla^a \beta_o) (\nabla_b \nabla_c \lambda_n) (\nabla^b \sigma_1) (\nabla^c \sigma_2) + \\
& \mathcal{R}\mathcal{R}\mathcal{P}^{mno} (\nabla_a \lambda_o) (\nabla^a \lambda_m) (\nabla_b \nabla_c \lambda_n) (\nabla^b \sigma_1) (\nabla^c \sigma_2) - \\
& \beta^m (\nabla_a \nabla_b \lambda_o) (\nabla^a \lambda^n) (\nabla^b \sigma_1) (\nabla_c \mathcal{R}\mathcal{R}\mathcal{P}_{mn}^o) (\nabla^c \sigma_2) + \\
& \mathcal{R}\mathcal{R}\mathcal{P}^{mno} (\nabla^a \beta_o) (\nabla_b \sigma_1) (\nabla^b \lambda_m) (\nabla_c \nabla_a \lambda_n) (\nabla^c \sigma_2) + \\
& \mathcal{R}\mathcal{R}\mathcal{P}^{mno} (\nabla^a \lambda_m) (\nabla_b \sigma_1) (\nabla^b \lambda_o) (\nabla_c \nabla_a \lambda_n) (\nabla^c \sigma_2) - \\
& \mathcal{R}\mathcal{R}\mathcal{P}_m^{no} \beta^m (\nabla^a \lambda_n) (\nabla^b \sigma_1) (\nabla_c \nabla_a \nabla_b \lambda_o) (\nabla^c \sigma_2) - \\
& \mathcal{R}\mathcal{R}\mathcal{P}^{mno} (\nabla_a \sigma_1) (\nabla^a \lambda_m) (\nabla^b \lambda_o) (\nabla_c \nabla_b \lambda_n) (\nabla^c \sigma_2) + \\
& \mathcal{R}\mathcal{R}\mathcal{P}^{mno} (\nabla_a \lambda_m) (\nabla^a \beta_o) (\nabla^b \sigma_1) (\nabla_c \nabla_b \lambda_n) (\nabla^c \sigma_2) - \\
& \mathcal{R}\mathcal{R}\mathcal{P}^{mno} (\nabla_a \lambda_o) (\nabla^a \lambda_m) (\nabla^b \sigma_1) (\nabla_c \nabla_b \lambda_n) (\nabla^c \sigma_2) \\
Z[30]: & \mathcal{R}\mathcal{R}\mathcal{R}\mathcal{A}_m^{nop} \beta^m (\nabla_a \sigma_1) (\nabla^a \lambda_n) (\nabla_b \sigma_2) (\nabla^b \lambda_o) (\nabla_c \nabla^c \lambda_p) + \\
& \mathcal{R}\mathcal{R}\mathcal{R}\mathcal{A}^{mnop} (\nabla_a \sigma_1) (\nabla^a \beta_p) (\nabla_b \lambda_n) (\nabla^b \lambda_m) (\nabla_c \sigma_2) (\nabla^c \lambda_o) - \\
2 & \mathcal{R}\mathcal{R}\mathcal{R}\mathcal{A}^{mnop} (\nabla_a \lambda_n) (\nabla^a \lambda_m) (\nabla_b \sigma_1) (\nabla^b \lambda_o) (\nabla_c \sigma_2) (\nabla^c \lambda_p)
\end{aligned}$$

## (0,1) terms: twenty four consistency conditions

■ 18)  $(\sigma_1 \partial_\rho \sigma_2 - \sigma_2 \partial_\rho \sigma_1) R^{\mu\nu\rho\sigma}$ 

$$\begin{aligned} T[18]: & -4 R[\nabla]^{abcd} \sigma_1 (\nabla_a \lambda^m) (\nabla_b \nabla_d I 7_m) (\nabla_c \sigma_2) + 4 R[\nabla]^{abcd} \sigma_1 (\nabla_a I 7^m) (\nabla_b \nabla_d \lambda_m) (\nabla_c \sigma_2) + \\ & 4 R[\nabla]^{abcd} \sigma_1 (\nabla_a I 7^m) (\nabla_b \sigma_2) (\nabla_d \nabla_c \lambda_m) - 4 R[\nabla]^{abcd} I 7^m \sigma_1 (\nabla_a \sigma_2) (\nabla_d \nabla_c \nabla_b \lambda_m) \end{aligned}$$

$$\begin{aligned} T[23]: & 8 R[\nabla]^{abcd} \mathcal{H} \mathcal{H} 1^{mn} \sigma_1 (\nabla_a \lambda_m) (\nabla_b \nabla_d \lambda_n) (\nabla_c \sigma_2) - \\ & 8 R[\nabla]^{abcd} \sigma_1 (\nabla_a \lambda^m) (\nabla_b \sigma_2) (\nabla_c \lambda^n) (\nabla_d \mathcal{H} \mathcal{H} 1_{mn}) - \\ & 8 R[\nabla]^{abcd} \mathcal{H} \mathcal{H} 1^{mn} \sigma_1 (\nabla_a \lambda_m) (\nabla_b \sigma_2) (\nabla_d \nabla_c \lambda_n) \end{aligned}$$

$$\begin{aligned} T[26]: & 2 R[\nabla]^{abcd} \mathcal{H} \mathcal{H} 4^{mn} \sigma_1 (\nabla_a \lambda_m) (\nabla_b \nabla_d \lambda_n) (\nabla_c \sigma_2) - \\ & 2 R[\nabla]^{abcd} \sigma_1 (\nabla_a \lambda^m) (\nabla_b \sigma_2) (\nabla_c \lambda^n) (\nabla_d \mathcal{H} \mathcal{H} 4_{mn}) - \\ & 2 R[\nabla]^{abcd} \mathcal{H} \mathcal{H} 4^{mn} \sigma_1 (\nabla_a \lambda_m) (\nabla_b \sigma_2) (\nabla_d \nabla_c \lambda_n) \end{aligned}$$

$$T[29]: -2 R[\nabla]^{abcd} \mathcal{F} \mathcal{F}^{mn} \sigma_1 (\nabla_a \lambda_m) (\nabla_b \nabla_d \lambda_n) (\nabla_c \sigma_2)$$

$$\begin{aligned} T[34]: & -R[\nabla]^{abcd} \mathcal{D} \mathcal{D} \mathcal{D}^{mnp} \beta_p \sigma_1 (\nabla_a \lambda_n) (\nabla_b \nabla_d \lambda_m) (\nabla_c \sigma_2) - \\ & R[\nabla]^{abcd} \mathcal{D} \mathcal{D} \mathcal{D}^{mnp} \beta_n \sigma_1 (\nabla_a \lambda_m) (\nabla_b \nabla_d \lambda_p) (\nabla_c \sigma_2) + \\ & R[\nabla]^{abcd} \mathcal{D} \mathcal{D} \mathcal{D}^{mnp} \sigma_1 (\nabla_a \lambda_m) (\nabla_b \sigma_2) (\nabla_c \lambda_n) (\nabla_d \lambda_p) + \\ & R[\nabla]^{abcd} \mathcal{D} \mathcal{D} \mathcal{D}^{mnp} \sigma_1 (\nabla_a \beta_p) (\nabla_b \lambda_m) (\nabla_c \lambda_n) (\nabla_d \sigma_2) - \\ & R[\nabla]^{abcd} \beta^m \sigma_1 (\nabla_a \mathcal{D} \mathcal{D} \mathcal{D}^{np}_m) (\nabla_b \lambda_p) (\nabla_c \lambda_n) (\nabla_d \sigma_2) + \\ & R[\nabla]^{abcd} \mathcal{D} \mathcal{D} \mathcal{D}^{mnp} \sigma_1 (\nabla_a \lambda_m) (\nabla_b \lambda_p) (\nabla_c \lambda_n) (\nabla_d \sigma_2) - \\ & R[\nabla]^{abcd} \mathcal{D} \mathcal{D} \mathcal{D}^{mnp} \beta_m \sigma_1 (\nabla_a \lambda_n) (\nabla_c \sigma_2) (\nabla_d \nabla_b \lambda_p) + \\ & R[\nabla]^{abcd} \mathcal{D} \mathcal{D} \mathcal{D}^{mnp} \beta_p \sigma_1 (\nabla_a \lambda_m) (\nabla_b \sigma_2) (\nabla_d \nabla_c \lambda_n) \end{aligned}$$

$$T[35]: R[\nabla]^{abcd} \mathcal{D} \mathcal{D} \mathcal{D} \mathcal{D}^{nop} \beta^m \sigma_1 (\nabla_a \lambda_n) (\nabla_b \sigma_2) (\nabla_c \lambda_o) (\nabla_d \lambda_p)$$

$$\begin{aligned} T[51]: & 2 R[\nabla]^{abcd} \mathcal{A} \mathcal{A} \text{hatpp}^{mn} \sigma_1 (\nabla_a \lambda_m) (\nabla_b \nabla_d \lambda_n) (\nabla_c \sigma_2) + \\ & 3 R[\nabla]^{abcd} \beta^m \sigma_1 (\nabla_a \sigma_2) (\nabla_c \mathcal{A} \mathcal{A} \text{hatpp}^n_m) (\nabla_d \nabla_b \lambda_n) - \\ & 2 R[\nabla]^{abcd} \mathcal{A} \mathcal{A} \text{hatpp}^{mn} \sigma_1 (\nabla_a \beta_m) (\nabla_c \sigma_2) (\nabla_d \nabla_b \lambda_n) + \\ & 2 R[\nabla]^{abcd} \mathcal{A} \mathcal{A} \text{hatpp}^{mn} \sigma_1 (\nabla_a \lambda_m) (\nabla_c \sigma_2) (\nabla_d \nabla_b \lambda_n) - \\ & 2 R[\nabla]^{abcd} \mathcal{A} \mathcal{A} \text{hatpp}^n_m \beta^m \sigma_1 (\nabla_a \sigma_2) (\nabla_d \nabla_c \nabla_b \lambda_n) \end{aligned}$$

$$\begin{aligned} Z[21]: & R[\nabla]^{abcd} \mathcal{D} \mathcal{D}^{mn} \sigma_1 (\nabla_a \lambda_m) (\nabla_c \sigma_2) (\nabla_d \nabla_b \beta_n) + \\ & R[\nabla]^{abcd} \mathcal{D} \mathcal{D}^{mn} \sigma_1 (\nabla_a \beta_m) (\nabla_c \sigma_2) (\nabla_d \nabla_b \lambda_n) + R[\nabla]^{abcd} \beta^m \sigma_1 \partial_m \mathcal{D} \mathcal{D}^{no} (\nabla_a \lambda_n) (\nabla_c \sigma_2) (\nabla_d \nabla_b \lambda_o) \end{aligned}$$

■ 19)  $(\sigma_1 \partial_\nu \sigma_2 - \sigma_2 \partial_\nu \sigma_1) G^{\mu\nu}$ 

$$\begin{aligned} T[12]: & -4 G[\nabla]^{ab} I 1^m \sigma_1 (\nabla_a \sigma_2) (\nabla_b \nabla_c \nabla^c \lambda_m) - 4 G[\nabla]^{ab} \sigma_1 (\nabla_a I 1^m) (\nabla_b \sigma_2) (\nabla_c \nabla^c \lambda_m) - \\ & 4 G[\nabla]^{ab} \sigma_1 (\nabla_a \sigma_2) (\nabla_b \nabla_c \lambda_m) (\nabla^c I 1^m) - 4 G[\nabla]^{ab} \sigma_1 (\nabla_a \sigma_2) (\nabla_b \nabla_c I 1_m) (\nabla^c \lambda^m) \end{aligned}$$

$$\begin{aligned} T[17]: & 8 G[\nabla]^{ab} I 6^m \sigma_1 (\nabla_a \sigma_2) (\nabla_b \nabla_c \nabla^c \lambda_m) + 4 G[\nabla]^{ab} \sigma_1 (\nabla_a \lambda^m) (\nabla_b \sigma_2) (\nabla_c \nabla^c I 6_m) + \\ & 4 G[\nabla]^{ab} \sigma_1 (\nabla_a I 6^m) (\nabla_b \sigma_2) (\nabla_c \nabla^c \lambda_m) + 4 G[\nabla]^{ab} \sigma_1 (\nabla_a \sigma_2) (\nabla_b \nabla_c \lambda_m) (\nabla^c I 6^m) + \\ & 8 G[\nabla]^{ab} \sigma_1 (\nabla_a \sigma_2) (\nabla_c \nabla_b \lambda_m) (\nabla^c I 6^m) + 4 G[\nabla]^{ab} \sigma_1 (\nabla_a \sigma_2) (\nabla_c \nabla_b I 6_m) (\nabla^c \lambda^m) \end{aligned}$$

$$\begin{aligned} T[18]: & -G[\nabla]^{ab} I 7^m \sigma_1 (\nabla_a \sigma_2) (\nabla_b \nabla_c \nabla^c \lambda_m) - \\ & G[\nabla]^{ab} \sigma_1 (\nabla_a \lambda^m) (\nabla_b \sigma_2) (\nabla_c \nabla^c I 7_m) - 2 G[\nabla]^{ab} \sigma_1 (\nabla_a \sigma_2) (\nabla_c \nabla_b \lambda_m) (\nabla^c I 7^m) + \\ & G[\nabla]^{ab} \sigma_1 (\nabla_a \sigma_2) (\nabla_b \nabla_c I 7_m) (\nabla^c \lambda^m) - G[\nabla]^{ab} \sigma_1 (\nabla_a \sigma_2) (\nabla_c \nabla_b I 7_m) (\nabla^c \lambda^m) \end{aligned}$$

$$\begin{aligned} T[19]: & 4 G[\nabla]^{ab} \mathcal{G} \mathcal{G} 1^{mn} \sigma_1 (\nabla_a \sigma_2) (\nabla_b \nabla_c \lambda_n) (\nabla^c \lambda_m) + 2 G[\nabla]^{ab} \sigma_1 (\nabla_a \sigma_2) (\nabla_b \mathcal{G} \mathcal{G} 1_{mn}) (\nabla_c \lambda^n) (\nabla^c \lambda^m) \end{aligned}$$

$$\begin{aligned}
\text{T}[23]: & -16 \, G[\nabla]^{ab} \, \mathcal{HH1}^{mn} \, \sigma_1 (\nabla_a \lambda_m) (\nabla_b \sigma_2) (\nabla_c \nabla^c \lambda_n) + \\
& 16 \, G[\nabla]^{ab} \, \mathcal{HH1}^{mn} \, \sigma_1 (\nabla_a \sigma_2) (\nabla_b \nabla_c \lambda_n) (\nabla^c \lambda_m) - 16 \, G[\nabla]^{ab} \, \mathcal{HH1}^{mn} \, \sigma_1 (\nabla_a \sigma_2) (\nabla_c \nabla_b \lambda_n) (\nabla^c \lambda_m) + \\
& 8 \, G[\nabla]^{ab} \, \sigma_1 (\nabla_a \sigma_2) (\nabla_b \mathcal{HH1}_{mn}) (\nabla_c \lambda^n) (\nabla^c \lambda^m) - 16 \, G[\nabla]^{ab} \, \sigma_1 (\nabla_a \lambda^m) (\nabla_b \sigma_2) (\nabla_c \mathcal{HH1}_{mn}) (\nabla^c \lambda^n) \\
\text{T}[25]: & -4 \, G[\nabla]^{ab} \, \mathcal{HH3}^{mn} \, \sigma_1 (\nabla_a \lambda_m) (\nabla_b \sigma_2) (\nabla_c \nabla^c \lambda_n) - \\
& 4 \, G[\nabla]^{ab} \, \mathcal{HH3}^{mn} \, \sigma_1 (\nabla_a \sigma_2) (\nabla_b \nabla_c \lambda_n) (\nabla^c \lambda_m) - 4 \, G[\nabla]^{ab} \, \sigma_1 (\nabla_a \lambda^m) (\nabla_b \sigma_2) (\nabla_c \mathcal{HH3}_{mn}) (\nabla^c \lambda^n) \\
\text{T}[26]: & G[\nabla]^{ab} \, \mathcal{HH4}^{mn} \, \sigma_1 (\nabla_a \lambda_m) (\nabla_b \sigma_2) (\nabla_c \nabla^c \lambda_n) - \\
& G[\nabla]^{ab} \, \mathcal{HH4}^{mn} \, \sigma_1 (\nabla_a \sigma_2) (\nabla_b \nabla_c \lambda_n) (\nabla^c \lambda_m) + G[\nabla]^{ab} \, \mathcal{HH4}^{mn} \, \sigma_1 (\nabla_a \sigma_2) (\nabla_c \nabla_b \lambda_n) (\nabla^c \lambda_m) - \\
& \frac{1}{2} \, G[\nabla]^{ab} \, \sigma_1 (\nabla_a \sigma_2) (\nabla_b \mathcal{HH4}_{mn}) (\nabla_c \lambda^n) (\nabla^c \lambda^m) + G[\nabla]^{ab} \, \sigma_1 (\nabla_a \lambda^m) (\nabla_b \sigma_2) (\nabla_c \mathcal{HH4}_{mn}) (\nabla^c \lambda^n) \\
\text{T}[29]: & 2 \, G[\nabla]^{ab} \, \mathcal{FF}^{mn} \, \sigma_1 (\nabla_a \lambda_n) (\nabla_b \sigma_2) (\nabla_c \nabla^c \lambda_m) + 2 \, G[\nabla]^{ab} \, \sigma_1 (\nabla_a \lambda_n) (\nabla_b \sigma_2) (\nabla_c \lambda_m) (\nabla^c \mathcal{FF}^{mn}) - \\
& \frac{1}{2} \, G[\nabla]^{ab} \, \mathcal{FF}^{mn} \, \sigma_1 (\nabla_a \sigma_2) (\nabla_b \nabla_c \lambda_n) (\nabla^c \lambda_m) + \frac{3}{2} \, G[\nabla]^{ab} \, \mathcal{FF}^{mn} \, \sigma_1 (\nabla_a \sigma_2) (\nabla_c \nabla_b \lambda_n) (\nabla^c \lambda_m) \\
\text{T}[30]: & -\frac{1}{2} \, G[\nabla]^{ab} \, \mathcal{FFP}^{mn} \, \sigma_1 (\nabla_a \lambda_m) (\nabla_b \sigma_2) (\nabla_c \nabla^c \lambda_n) - \frac{1}{2} \, G[\nabla]^{ab} \, \mathcal{FFP}^{mn} \, \sigma_1 (\nabla_a \sigma_2) (\nabla_c \nabla_b \lambda_n) (\nabla^c \lambda_m) \\
\text{T}[31]: & -\frac{1}{2} \, G[\nabla]^{ab} \, \mathcal{FFF}^{mnp} \, \sigma_1 (\nabla_a \lambda_n) (\nabla_b \sigma_2) (\nabla_c \lambda_p) (\nabla^c \lambda_m) \\
\text{T}[34]: & -G[\nabla]^{ab} \, \mathcal{DDD}^{mnp} \, \sigma_1 (\nabla_a \lambda_p) (\nabla_b \sigma_2) (\nabla_c \lambda_n) (\nabla^c \lambda_m) \\
\text{T}[36]: & \frac{1}{2} \, G[\nabla]^{ab} \, \mathcal{CChat}^{mn} \, \beta_m \, \sigma_1 (\nabla_a \sigma_2) (\nabla_b \nabla_c \nabla^c \lambda_n) + \frac{1}{2} \, G[\nabla]^{ab} \, \beta^m \, \sigma_1 (\nabla_a \mathcal{CChat}_m^n) (\nabla_b \sigma_2) (\nabla_c \nabla^c \lambda_n) - \\
& \frac{1}{2} \, G[\nabla]^{ab} \, \mathcal{CChat}^{mn} \, \sigma_1 (\nabla_a \beta_m) (\nabla_b \sigma_2) (\nabla_c \nabla^c \lambda_n) - G[\nabla]^{ab} \, \mathcal{CChat}^{mn} \, \sigma_1 (\nabla_a \lambda_m) (\nabla_b \sigma_2) (\nabla_c \nabla^c \lambda_n) \\
\text{T}[37]: & \frac{1}{2} \, G[\nabla]^{ab} \, \mathcal{CChatp}_m^n \, \beta^m \, \sigma_1 (\nabla_a \sigma_2) (\nabla_b \nabla_c \nabla^c \lambda_n) + \\
& \frac{1}{2} \, G[\nabla]^{ab} \, \beta^m \, \sigma_1 (\nabla_a \sigma_2) (\nabla_c \nabla_b \lambda_n) (\nabla^c \mathcal{CChatp}_m^n) + \\
& \frac{1}{2} \, G[\nabla]^{ab} \, \mathcal{CChatp}^{mn} \, \sigma_1 (\nabla_a \sigma_2) (\nabla_c \nabla_b \lambda_n) (\nabla^c \lambda_m) \\
\text{T}[38]: & \frac{1}{4} \, G[\nabla]^{ab} \, \mathcal{CCC}^{np}_m \, \beta^m \, \sigma_1 (\nabla_a \lambda_n) (\nabla_b \sigma_2) (\nabla_c \nabla^c \lambda_p) + \\
& \frac{1}{4} \, G[\nabla]^{ab} \, \mathcal{CCC}^{mnp} \, \sigma_1 (\nabla_a \lambda_m) (\nabla_b \sigma_2) (\nabla_c \lambda_p) (\nabla^c \lambda_n) - \\
& \frac{1}{4} \, G[\nabla]^{ab} \, \mathcal{CCC}_m^{np} \, \beta^m \, \sigma_1 (\nabla_a \sigma_2) (\nabla_c \nabla_b \lambda_p) (\nabla^c \lambda_n) + \\
& \frac{1}{4} \, G[\nabla]^{ab} \, \mathcal{CCC}^{np}_m \, \beta^m \, \sigma_1 (\nabla_a \sigma_2) (\nabla_c \nabla_b \lambda_p) (\nabla^c \lambda_n) + \\
& \frac{1}{4} \, G[\nabla]^{ab} \, \beta^m \, \sigma_1 (\nabla_a \lambda^n) (\nabla_b \sigma_2) (\nabla_c \mathcal{CCC}_{npm}) (\nabla^c \lambda^p)
\end{aligned}$$



$$\begin{aligned}
T[39]: & \frac{1}{2} G[\nabla]^{ab} CCCP^{mnp} \beta_p \sigma 1 (\nabla_a \lambda_m) (\nabla_b \sigma 2) (\nabla_c \nabla^c \lambda_n) + \\
& \frac{1}{2} G[\nabla]^{ab} \beta^m \sigma 1 (\nabla_a \lambda_n) (\nabla_b \sigma 2) (\nabla_c \lambda_p) (\nabla^c CCCP^{np}_m) - \\
& \frac{1}{2} G[\nabla]^{ab} CCCP^{mnp} \beta_m \sigma 1 (\nabla_a \sigma 2) (\nabla_b \nabla_c \lambda_p) (\nabla^c \lambda_n) + \\
& \frac{1}{2} G[\nabla]^{ab} CCCP^{mnp} \sigma 1 (\nabla_a \lambda_m) (\nabla_b \sigma 2) (\nabla_c \lambda_p) (\nabla^c \lambda_n) + \\
& \frac{1}{2} G[\nabla]^{ab} CCCP^{mnp} \beta_p \sigma 1 (\nabla_a \sigma 2) (\nabla_c \nabla_b \lambda_m) (\nabla^c \lambda_n)
\end{aligned}$$

$$\begin{aligned}
T[40]: & -\frac{1}{4} G[\nabla]^{ab} CCCpp^{mnp} \sigma 1 (\nabla_a \beta_p) (\nabla_b \sigma 2) (\nabla_c \lambda_n) (\nabla^c \lambda_m) - \\
& \frac{1}{2} G[\nabla]^{ab} CCCpp^{mnp} \sigma 1 (\nabla_a \lambda_p) (\nabla_b \sigma 2) (\nabla_c \lambda_n) (\nabla^c \lambda_m) + \\
& \frac{1}{2} G[\nabla]^{ab} CCCpp^{np}_m \beta^m \sigma 1 (\nabla_a \sigma 2) (\nabla_b \nabla_c \lambda_p) (\nabla^c \lambda_n) + \\
& \frac{1}{4} G[\nabla]^{ab} \beta^m \sigma 1 (\nabla_a \sigma 2) (\nabla_b CCCpp_{nmp}) (\nabla_c \lambda^p) (\nabla^c \lambda^n)
\end{aligned}$$

$$T[41]: -\frac{1}{4} G[\nabla]^{ab} CCCC^{nop}_m \beta^m \sigma 1 (\nabla_a \lambda_n) (\nabla_b \sigma 2) (\nabla_c \lambda_p) (\nabla^c \lambda_o)$$

$$\begin{aligned}
T[48]: & 2 G[\nabla]^{ab} \sigma 1 (\nabla_a \beta^m) (\nabla_b \sigma 2) (\nabla_c \nabla^c \mathcal{J}_m) + 4 G[\nabla]^{ab} \sigma 1 (\nabla_a \lambda^m) (\nabla_b \sigma 2) (\nabla_c \nabla^c \mathcal{J}_m) + \\
& 2 G[\nabla]^{ab} \sigma 1 (\nabla_a \sigma 2) (\nabla_c \nabla_b \beta_m) (\nabla^c \mathcal{J}^m) + 4 G[\nabla]^{ab} \sigma 1 (\nabla_a \sigma 2) (\nabla_c \nabla_b \lambda_m) (\nabla^c \mathcal{J}^m)
\end{aligned}$$

$$\begin{aligned}
T[51]: & -2 G[\nabla]^{ab} \mathcal{A}\mathcal{A}\text{hatpp}^n_m \beta^m \sigma 1 (\nabla_a \sigma 2) (\nabla_b \nabla_c \nabla^c \lambda_n) - \\
& 2 G[\nabla]^{ab} \beta^m \sigma 1 (\nabla_a \sigma 2) (\nabla_c \nabla_b \lambda_n) (\nabla^c \mathcal{A}\mathcal{A}\text{hatpp}^n_m) + \\
& G[\nabla]^{ab} \mathcal{A}\mathcal{A}\text{hatpp}^{mn} \sigma 1 (\nabla_a \sigma 2) (\nabla_b \nabla_c \lambda_n) (\nabla^c \beta_m) - \\
& G[\nabla]^{ab} \mathcal{A}\mathcal{A}\text{hatpp}^{mn} \sigma 1 (\nabla_a \sigma 2) (\nabla_b \nabla_c \lambda_n) (\nabla^c \lambda_m) - G[\nabla]^{ab} \mathcal{A}\mathcal{A}\text{hatpp}^{mn} \sigma 1 (\nabla_a \sigma 2) (\nabla_c \nabla_b \lambda_n) (\nabla^c \lambda_m)
\end{aligned}$$

$$T[53]: G[\nabla]^{ab} \mathcal{A}\mathcal{A}\text{hatp}^{np}_m \beta^m \sigma 1 (\nabla_a \lambda_n) (\nabla_b \sigma 2) (\nabla_c \nabla^c \lambda_p)$$

$$T[59]: \frac{1}{2} G[\nabla]^{ab} \mathcal{A}\mathcal{A}\mathcal{A}\text{hatp}^{no\ p}_m \beta^m \sigma 1 (\nabla_a \lambda_p) (\nabla_b \sigma 2) (\nabla_c \lambda_o) (\nabla^c \lambda_n)$$

$$Z[22]: \frac{1}{2} G[\nabla]^{ab} C^m \sigma 1 (\nabla_a \sigma 2) (\nabla_b \nabla_c \nabla^c \beta_m) + \frac{1}{2} G[\nabla]^{ab} \beta^m \sigma 1 \partial_m C^n (\nabla_a \sigma 2) (\nabla_b \nabla_c \nabla^c \lambda_n)$$

$$\begin{aligned}
Z[23]: & \frac{1}{2} G[\nabla]^{ab} CC^{mn} \sigma 1 (\nabla_a \sigma 2) (\nabla_b \nabla_c \lambda_n) (\nabla^c \beta_m) + \\
& \frac{1}{2} G[\nabla]^{ab} CC^{mn} \sigma 1 (\nabla_a \sigma 2) (\nabla_b \nabla_c \beta_n) (\nabla^c \lambda_m) + \frac{1}{2} G[\nabla]^{ab} \beta^m \sigma 1 \partial_m CC^{no} (\nabla_a \sigma 2) (\nabla_b \nabla_c \lambda_o) (\nabla^c \lambda_n)
\end{aligned}$$

$$\begin{aligned}
Z[24]: & \frac{1}{2} G[\nabla]^{ab} CCP^{mn} \sigma 1 (\nabla_a \lambda_m) (\nabla_b \sigma 2) (\nabla_c \nabla^c \beta_n) + \frac{1}{2} G[\nabla]^{ab} CCP^{mn} \sigma 1 (\nabla_a \beta_m) (\nabla_b \sigma 2) (\nabla_c \nabla^c \lambda_n) + \\
& \frac{1}{2} G[\nabla]^{ab} \beta^m \sigma 1 \partial_m CCP^{no} (\nabla_a \lambda_n) (\nabla_b \sigma 2) (\nabla_c \nabla^c \lambda_o)
\end{aligned}$$

■ 20)  $(\sigma_1 \partial_\mu \sigma_2 - \sigma_2 \partial_\mu \sigma_1) G_{\nu\rho}$

$$T[15]: 4 G[\nabla]^{ab} \sigma 1 (\nabla_a \lambda^m) (\nabla_c \nabla_b \mathcal{I}4_m) (\nabla^c \sigma 2) + 4 G[\nabla]^{ab} \sigma 1 (\nabla_a \mathcal{I}4^m) (\nabla_c \nabla_b \lambda_m) (\nabla^c \sigma 2)$$

Printed by Mathematica for Students

$$\begin{aligned}
\text{T}[36]: & \frac{1}{2} G[\nabla]^{ab} \beta^m \sigma 1 (\nabla_b \nabla_a \lambda_n) (\nabla_c \sigma 2) (\nabla^c C\text{Chat}^n_m) - \\
& \frac{1}{2} G[\nabla]^{ab} C\text{Chat}^{mn} \sigma 1 (\nabla_b \nabla_a \lambda_m) (\nabla_c \sigma 2) (\nabla^c \beta_n) - \\
& 2 G[\nabla]^{ab} C\text{Chat}^{mn} \sigma 1 (\nabla_b \nabla_a \lambda_m) (\nabla_c \sigma 2) (\nabla^c \lambda_n) + \frac{1}{2} G[\nabla]^{ab} C\text{Chat}^{mn} \beta_n \sigma 1 (\nabla_b \nabla_a \lambda_m) (\nabla^c \sigma 2) \\
\text{T}[37]: & -\frac{1}{2} G[\nabla]^{ab} C\text{Chatp}^{mn} \sigma 1 (\nabla_b \nabla_a \lambda_n) (\nabla_c \sigma 2) (\nabla^c \lambda_m) - \\
& G[\nabla]^{ab} C\text{Chatp}^{mn} \sigma 1 (\nabla_a \lambda_m) (\nabla_b \nabla_c \lambda_n) (\nabla^c \sigma 2) - \\
& \frac{1}{2} G[\nabla]^{ab} C\text{Chatp}^{mn} \sigma 1 (\nabla_a \beta_m) (\nabla_c \nabla_b \lambda_n) (\nabla^c \sigma 2) + \\
& \frac{1}{2} G[\nabla]^{ab} C\text{Chatp}^{mn} \sigma 1 (\nabla_a \lambda_m) (\nabla_c \nabla_b \lambda_n) (\nabla^c \sigma 2) \\
\text{T}[38]: & -\frac{1}{4} G[\nabla]^{ab} CCC^{mnp} \sigma 1 (\nabla_a \beta_p) (\nabla_b \lambda_m) (\nabla_c \sigma 2) (\nabla^c \lambda_n) - \\
& \frac{3}{4} G[\nabla]^{ab} CCC^{mnp} \sigma 1 (\nabla_a \lambda_m) (\nabla_b \lambda_p) (\nabla_c \sigma 2) (\nabla^c \lambda_n) - \\
& \frac{1}{4} G[\nabla]^{ab} CCC^{mnp} \sigma 1 (\nabla_a \lambda_m) (\nabla_b \lambda_n) (\nabla_c \sigma 2) (\nabla^c \lambda_p) - \\
& \frac{1}{4} G[\nabla]^{ab} CCC_m^{np} \beta^m \sigma 1 (\nabla_a \lambda_n) (\nabla_c \nabla_b \lambda_p) (\nabla^c \sigma 2) \\
\text{T}[39]: & -2 G[\nabla]^{ab} CCCp^{mnp} \sigma 1 (\nabla_a \lambda_n) (\nabla_b \lambda_p) (\nabla_c \sigma 2) (\nabla^c \lambda_m) - \\
& \frac{1}{2} G[\nabla]^{ab} CCCp^{mnp} \sigma 1 (\nabla_a \beta_p) (\nabla_b \lambda_m) (\nabla_c \sigma 2) (\nabla^c \lambda_n) + \\
& \frac{1}{2} G[\nabla]^{ab} CCCp^{mnp} \sigma 1 (\nabla_a \lambda_m) (\nabla_b \lambda_p) (\nabla_c \sigma 2) (\nabla^c \lambda_n) - \\
& \frac{1}{2} G[\nabla]^{ab} CCCp^{mnp} \sigma 1 (\nabla_a \lambda_m) (\nabla_b \lambda_n) (\nabla_c \sigma 2) (\nabla^c \lambda_p) - \\
& \frac{1}{2} G[\nabla]^{ab} CCCp^{mnp} \beta_n \sigma 1 (\nabla_a \lambda_m) (\nabla_b \nabla_c \lambda_p) (\nabla^c \sigma 2) \\
\text{T}[40]: & -\frac{1}{2} G[\nabla]^{ab} CCCpp_m^{np} \beta^m \sigma 1 (\nabla_b \nabla_a \lambda_p) (\nabla_c \sigma 2) (\nabla^c \lambda_n) \\
\text{T}[41]: & -\frac{1}{4} G[\nabla]^{ab} CCCc^{no p}_m \beta^m \sigma 1 (\nabla_a \lambda_n) (\nabla_b \lambda_o) (\nabla_c \sigma 2) (\nabla^c \lambda_p) \\
\text{T}[48]: & -2 G[\nabla]^{ab} \sigma 1 (\nabla_b \nabla_a \beta_m) (\nabla_c \sigma 2) (\nabla^c \mathcal{A}^m) - 4 G[\nabla]^{ab} \sigma 1 (\nabla_b \nabla_a \lambda_m) (\nabla_c \sigma 2) (\nabla^c \mathcal{A}^m) - \\
& 2 G[\nabla]^{ab} \sigma 1 (\nabla_a \beta^m) (\nabla_b \nabla_c \mathcal{A}_m) (\nabla^c \sigma 2) - 4 G[\nabla]^{ab} \sigma 1 (\nabla_a \lambda^m) (\nabla_b \nabla_c \mathcal{A}_m) (\nabla^c \sigma 2) \\
\text{T}[51]: & -G[\nabla]^{ab} \mathcal{A}\text{hatpp}_m^n \beta^m \sigma 1 (\nabla_b \nabla_a \nabla_c \lambda_n) (\nabla^c \sigma 2) - \\
& 2 G[\nabla]^{ab} \beta^m \sigma 1 (\nabla_a \mathcal{A}\text{hatpp}_m^n) (\nabla_b \nabla_c \lambda_n) (\nabla^c \sigma 2) - \\
& 2 G[\nabla]^{ab} \mathcal{A}\text{hatpp}^{mn} \sigma 1 (\nabla_a \lambda_m) (\nabla_b \nabla_c \lambda_n) (\nabla^c \sigma 2) + \\
& G[\nabla]^{ab} \mathcal{A}\text{hatpp}^{mn} \sigma 1 (\nabla_a \beta_m) (\nabla_c \nabla_b \lambda_n) (\nabla^c \sigma 2) - \\
& 2 G[\nabla]^{ab} \mathcal{A}\text{hatpp}^{mn} \sigma 1 (\nabla_a \lambda_m) (\nabla_c \nabla_b \lambda_n) (\nabla^c \sigma 2)
\end{aligned}$$

$$\begin{aligned} \text{T}[55]: & \text{G}[\nabla]^{\text{ab}} \mathcal{A}\mathcal{A}\mathcal{A}\text{hatp}^{\text{mnp}} \sigma_1 (\nabla_a \lambda_m) (\nabla_b \lambda_n) (\nabla_c \sigma_2) (\nabla^c \beta_p) + \\ & 4 \text{G}[\nabla]^{\text{ab}} \mathcal{A}\mathcal{A}\mathcal{A}\text{hatp}^{\text{mnp}} \sigma_1 (\nabla_a \lambda_m) (\nabla_b \lambda_n) (\nabla_c \sigma_2) (\nabla^c \lambda_p) - \\ & \text{G}[\nabla]^{\text{ab}} \beta^m \sigma_1 (\nabla_a \lambda^n) (\nabla_b \lambda^p) (\nabla_c \mathcal{A}\mathcal{A}\mathcal{A}\text{hatp}_{\text{npm}}) (\nabla^c \sigma_2) - \\ & 2 \text{G}[\nabla]^{\text{ab}} \mathcal{A}\mathcal{A}\mathcal{A}\text{hatp}_{\text{m}}^{\text{np}} \beta^m \sigma_1 (\nabla_a \lambda_n) (\nabla_c \nabla_b \lambda_p) (\nabla^c \sigma_2) \end{aligned}$$

$$\begin{aligned} \text{T}[56]: & - \text{G}[\nabla]^{\text{ab}} \mathcal{A}\mathcal{A}\mathcal{A}\text{checkp}^{\text{mnp}} \sigma_1 (\nabla_a \lambda_m) (\nabla_b \lambda_n) (\nabla_c \sigma_2) (\nabla^c \beta_p) - \\ & 4 \text{G}[\nabla]^{\text{ab}} \mathcal{A}\mathcal{A}\mathcal{A}\text{checkp}^{\text{mnp}} \sigma_1 (\nabla_a \lambda_m) (\nabla_b \lambda_n) (\nabla_c \sigma_2) (\nabla^c \lambda_p) + \\ & \text{G}[\nabla]^{\text{ab}} \beta^m \sigma_1 (\nabla_a \lambda^n) (\nabla_b \lambda^p) (\nabla_c \mathcal{A}\mathcal{A}\mathcal{A}\text{checkp}_{\text{npm}}) (\nabla^c \sigma_2) + \\ & 2 \text{G}[\nabla]^{\text{ab}} \mathcal{A}\mathcal{A}\mathcal{A}\text{checkp}_{\text{m}}^{\text{np}} \beta^m \sigma_1 (\nabla_a \lambda_n) (\nabla_c \nabla_b \lambda_p) (\nabla^c \sigma_2) \end{aligned}$$

$$\begin{aligned} \text{T}[57]: & - \frac{1}{2} \text{G}[\nabla]^{\text{ab}} \mathcal{A}\mathcal{A}\mathcal{A}\text{checkpp}^{\text{mnp}} \sigma_1 (\nabla_a \lambda_m) (\nabla_b \lambda_n) (\nabla_c \sigma_2) (\nabla^c \beta_p) + \\ & \text{G}[\nabla]^{\text{ab}} \mathcal{A}\mathcal{A}\mathcal{A}\text{checkpp}^{\text{mnp}} \sigma_1 (\nabla_a \beta_p) (\nabla_b \lambda_m) (\nabla_c \sigma_2) (\nabla^c \lambda_n) + \\ & 2 \text{G}[\nabla]^{\text{ab}} \mathcal{A}\mathcal{A}\mathcal{A}\text{checkpp}^{\text{mnp}} \sigma_1 (\nabla_a \lambda_m) (\nabla_b \lambda_p) (\nabla_c \sigma_2) (\nabla^c \lambda_n) - \\ & 2 \text{G}[\nabla]^{\text{ab}} \mathcal{A}\mathcal{A}\mathcal{A}\text{checkpp}^{\text{mnp}} \sigma_1 (\nabla_a \lambda_m) (\nabla_b \lambda_n) (\nabla_c \sigma_2) (\nabla^c \lambda_p) + \\ & \frac{1}{2} \text{G}[\nabla]^{\text{ab}} \beta^m \sigma_1 (\nabla_a \lambda^n) (\nabla_b \lambda^p) (\nabla_c \mathcal{A}\mathcal{A}\mathcal{A}\text{checkpp}_{\text{npm}}) (\nabla^c \sigma_2) + \\ & \text{G}[\nabla]^{\text{ab}} \mathcal{A}\mathcal{A}\mathcal{A}\text{checkpp}_{\text{m}}^{\text{np}} \beta^m \sigma_1 (\nabla_a \lambda_n) (\nabla_c \nabla_b \lambda_p) (\nabla^c \sigma_2) \end{aligned}$$

$$\begin{aligned} \text{T}[60]: & \frac{1}{2} \text{G}[\nabla]^{\text{ab}} \mathcal{A}\mathcal{A}\mathcal{A}\mathcal{A}\text{hatpp}_{\text{m}}^{\text{no p}} \beta^m \sigma_1 (\nabla_a \lambda_n) (\nabla_b \lambda_p) (\nabla_c \sigma_2) (\nabla^c \lambda_o) + \\ & \frac{1}{2} \text{G}[\nabla]^{\text{ab}} \mathcal{A}\mathcal{A}\mathcal{A}\mathcal{A}\text{hatpp}_{\text{m}}^{\text{nop}} \beta^m \sigma_1 (\nabla_a \lambda_n) (\nabla_b \lambda_p) (\nabla_c \sigma_2) (\nabla^c \lambda_o) \end{aligned}$$

$$\text{T}[62]: - \text{G}[\nabla]^{\text{ab}} \mathcal{A}\mathcal{A}\mathcal{A}\mathcal{A}\text{checkp}_{\text{m}}^{\text{nop}} \beta^m \sigma_1 (\nabla_a \lambda_n) (\nabla_b \lambda_o) (\nabla_c \sigma_2) (\nabla^c \lambda_p)$$

## ■ 21) $(\sigma_1 \partial_\rho \sigma_2 - \sigma_2 \partial_\rho \sigma_1) \nabla^\mu G^{\nu\rho}$

$$\text{T}[11]: -8 \sigma_1 (\nabla^a \sigma_2) (\nabla_c \nabla_b b_7) (\nabla^c \text{G}[\nabla]_a^b)$$

$$\text{T}[17]: 4 \text{I}6^{\text{m}} \sigma_1 (\nabla^a \sigma_2) (\nabla_b \nabla_c \lambda_m) (\nabla^c \text{G}[\nabla]_a^b) + 4 \text{I}6^{\text{m}} \sigma_1 (\nabla^a \sigma_2) (\nabla_c \nabla_b \lambda_m) (\nabla^c \text{G}[\nabla]_a^b)$$

$$\text{T}[18]: -5 \text{I}7^{\text{m}} \sigma_1 (\nabla^a \sigma_2) (\nabla_b \nabla_c \lambda_m) (\nabla^c \text{G}[\nabla]_a^b) - \text{I}7^{\text{m}} \sigma_1 (\nabla^a \sigma_2) (\nabla_c \nabla_b \lambda_m) (\nabla^c \text{G}[\nabla]_a^b)$$

$$\text{T}[29]: \frac{1}{2} \mathcal{F}\mathcal{F}^{\text{mn}} \beta_n \sigma_1 (\nabla^a \sigma_2) (\nabla_b \nabla_c \lambda_m) (\nabla^c \text{G}[\nabla]_a^b)$$

$$\text{T}[30]:$$

$$\frac{1}{2} \mathcal{F}\mathcal{F}\mathcal{P}^{\text{mn}} \beta_n \sigma_1 (\nabla^a \sigma_2) (\nabla_c \nabla_b \lambda_m) (\nabla^c \text{G}[\nabla]_a^b) - \frac{1}{2} \mathcal{F}\mathcal{F}\mathcal{P}^{\text{mn}} \beta_m \sigma_1 (\nabla^a \sigma_2) (\nabla_c \nabla_b \lambda_n) (\nabla^c \text{G}[\nabla]_a^b)$$

$$\text{T}[37]: \frac{1}{2} \mathcal{C}\mathcal{H}\text{atp}_{\text{m}}^{\text{n}} \beta^m \sigma_1 (\nabla^a \sigma_2) (\nabla_c \nabla_b \lambda_n) (\nabla^c \text{G}[\nabla]_a^b)$$

$$\begin{aligned} \text{T}[51]: & - \mathcal{A}\mathcal{H}\text{atpp}_{\text{m}}^{\text{n}} \beta^m \sigma_1 (\nabla^a \sigma_2) (\nabla_b \nabla_c \lambda_n) (\nabla^c \text{G}[\nabla]_a^b) - \\ & 2 \mathcal{A}\mathcal{H}\text{atpp}_{\text{m}}^{\text{n}} \beta^m \sigma_1 (\nabla^a \sigma_2) (\nabla_c \nabla_b \lambda_n) (\nabla^c \text{G}[\nabla]_a^b) \end{aligned}$$

■ 22)  $(\sigma_1 \partial_\rho \sigma_2 - \sigma_2 \partial_\rho \sigma_1) \nabla^\rho G^{\mu\nu}$

$$T[15]: 4 \sigma_1 (\nabla^a I4^m) (\nabla^b \lambda_m) (\nabla_c G[\nabla]_{ab}) (\nabla^c \sigma_2)$$

$$T[16]: 2 I5^m \sigma_1 (\nabla_a G[\nabla]^{bc}) (\nabla^a \sigma_2) (\nabla_c \nabla_b \lambda_m) + 2 \sigma_1 (\nabla^a I5^m) (\nabla^b \lambda_m) (\nabla_c G[\nabla]_{ab}) (\nabla^c \sigma_2)$$

$$T[17]: 2 I6^m \sigma_1 (\nabla_a G[\nabla]^{bc}) (\nabla^a \sigma_2) (\nabla_c \nabla_b \lambda_m) + 2 \sigma_1 (\nabla^a I6^m) (\nabla^b \lambda_m) (\nabla_c G[\nabla]_{ab}) (\nabla^c \sigma_2)$$

$$T[18]: 5 I7^m \sigma_1 (\nabla_a G[\nabla]^{bc}) (\nabla^a \sigma_2) (\nabla_c \nabla_b \lambda_m) + 5 \sigma_1 (\nabla^a I7^m) (\nabla^b \lambda_m) (\nabla_c G[\nabla]_{ab}) (\nabla^c \sigma_2)$$

$$T[22]: -2 \mathcal{GG}4^{mn} \sigma_1 (\nabla^a \lambda_m) (\nabla^b \lambda_n) (\nabla_c G[\nabla]_{ab}) (\nabla^c \sigma_2)$$

$$T[24]: -\mathcal{HH}2^{mn} \sigma_1 (\nabla^a \lambda_m) (\nabla^b \lambda_n) (\nabla_c G[\nabla]_{ab}) (\nabla^c \sigma_2)$$

$$T[25]: -\mathcal{HH}3^{mn} \sigma_1 (\nabla^a \lambda_m) (\nabla^b \lambda_n) (\nabla_c G[\nabla]_{ab}) (\nabla^c \sigma_2)$$

$$T[26]: -\frac{5}{2} \mathcal{HH}4^{mn} \sigma_1 (\nabla^a \lambda_m) (\nabla^b \lambda_n) (\nabla_c G[\nabla]_{ab}) (\nabla^c \sigma_2)$$

$$T[27]: -2 \mathcal{HH}5^{mn} \sigma_1 (\nabla^a \lambda_m) (\nabla^b \lambda_n) (\nabla_c G[\nabla]_{ab}) (\nabla^c \sigma_2)$$

$$T[28]: -\mathcal{HH}6^{mn} \sigma_1 (\nabla^a \lambda_m) (\nabla^b \lambda_n) (\nabla_c G[\nabla]_{ab}) (\nabla^c \sigma_2)$$

$$T[29]: -\frac{1}{2} \mathcal{FF}^{mn} \beta_m \sigma_1 (\nabla_a G[\nabla]^{bc}) (\nabla^a \sigma_2) (\nabla_c \nabla_b \lambda_n)$$

$$T[30]:$$

$$-\frac{1}{2} \mathcal{FFP}^{mn} \sigma_1 (\nabla^a \beta_n) (\nabla^b \lambda_m) (\nabla_c G[\nabla]_{ab}) (\nabla^c \sigma_2) - \frac{3}{2} \mathcal{FFP}^{mn} \sigma_1 (\nabla^a \lambda_m) (\nabla^b \lambda_n) (\nabla_c G[\nabla]_{ab}) (\nabla^c \sigma_2)$$

$$T[31]: -\frac{1}{4} \mathcal{FFF}_m^{np} \beta^m \sigma_1 (\nabla^a \lambda_n) (\nabla^b \lambda_p) (\nabla_c G[\nabla]_{ab}) (\nabla^c \sigma_2)$$

$$T[34]: \mathcal{DDD}^{mnp} \beta_p \sigma_1 (\nabla^a \lambda_m) (\nabla^b \lambda_n) (\nabla_c G[\nabla]_{ab}) (\nabla^c \sigma_2)$$

$$T[36]: \frac{1}{2} \mathcal{CChat}^{mn} \beta_n \sigma_1 (\nabla_a G[\nabla]^{bc}) (\nabla^a \sigma_2) (\nabla_c \nabla_b \lambda_m)$$

$$T[51]: -\beta^m \sigma_1 (\nabla^a \lambda^n) (\nabla_b G[\nabla]_a^c) (\nabla^b \sigma_2) (\nabla_c \mathcal{Ahatpp}_{mn}) + \\ \mathcal{Ahatpp}_m^n \beta^m \sigma_1 (\nabla_a G[\nabla]^{bc}) (\nabla^a \sigma_2) (\nabla_c \nabla_b \lambda_n) + \\ \mathcal{Ahatpp}^{mn} \sigma_1 (\nabla^a \beta_m) (\nabla^b \lambda_n) (\nabla_c G[\nabla]_{ab}) (\nabla^c \sigma_2) - \\ 2 \mathcal{Ahatpp}^{mn} \sigma_1 (\nabla^a \lambda_m) (\nabla^b \lambda_n) (\nabla_c G[\nabla]_{ab}) (\nabla^c \sigma_2)$$

$$T[55]: -\mathcal{AAhatp}_m^{np} \beta^m \sigma_1 (\nabla^a \lambda_n) (\nabla^b \lambda_p) (\nabla_c G[\nabla]_{ab}) (\nabla^c \sigma_2)$$

$$T[56]: \mathcal{AAcheckp}_m^{np} \beta^m \sigma_1 (\nabla^a \lambda_n) (\nabla^b \lambda_p) (\nabla_c G[\nabla]_{ab}) (\nabla^c \sigma_2)$$

$$T[57]: \frac{1}{2} \mathcal{AAcheckpp}_m^{np} \beta^m \sigma_1 (\nabla^a \lambda_n) (\nabla^b \lambda_p) (\nabla_c G[\nabla]_{ab}) (\nabla^c \sigma_2)$$

$$Z[18]: \mathcal{F}^m \sigma_1 (\nabla_a G[\nabla]^{bc}) (\nabla^a \sigma_2) (\nabla_c \nabla_b \beta_m) + \beta^m \sigma_1 \partial_m \mathcal{F}^n (\nabla_a G[\nabla]^{bc}) (\nabla^a \sigma_2) (\nabla_c \nabla_b \lambda_n)$$

■ 23)  $(\sigma_1 \partial_\mu \sigma_2 - \sigma_2 \partial_\mu \sigma_1) R^2$

$$T[5]: \frac{1}{20} R[\nabla]^2 \sigma_1 (\nabla_a \sigma_2) (\nabla^a b_1)$$

$$T[6]: -\frac{1}{20} R[\nabla]^2 \sigma_1 (\nabla_a \sigma_2) (\nabla^a b_2)$$

$$T[7]: -\frac{1}{40} R[\nabla]^2 \sigma_1 (\nabla_a \sigma_2) (\nabla^a b_3)$$

$$T[8]: -\frac{1}{10} R[\nabla]^2 \sigma_1 (\nabla_a \sigma_2) (\nabla^a b_4)$$

$$T[9]: R[\nabla]^2 \sigma_1 (\nabla_a \sigma_2) (\nabla^a b_5)$$

$$T[14]: \frac{2}{25} R[\nabla]^2 I_3^m \sigma_1 (\nabla_a \sigma_2) (\nabla^a \lambda_m)$$

$$T[16]: \frac{1}{5} R[\nabla]^2 I_5^m \sigma_1 (\nabla_a \sigma_2) (\nabla^a \lambda_m)$$

$$T[17]: \frac{3}{10} R[\nabla]^2 I_6^m \sigma_1 (\nabla_a \sigma_2) (\nabla^a \lambda_m)$$

$$T[18]: \frac{3}{10} R[\nabla]^2 I_7^m \sigma_1 (\nabla_a \sigma_2) (\nabla^a \lambda_m)$$

$$T[21]: -\frac{1}{25} R[\nabla]^2 \mathcal{G} \mathcal{G} 3_m^n \beta^m \sigma_1 (\nabla_a \sigma_2) (\nabla^a \lambda_n)$$

$$Z[10]: \frac{1}{25} R[\nabla]^2 \mathcal{G} 3^m \sigma_1 (\nabla_a \sigma_2) (\nabla^a \beta_m) + \frac{1}{25} R[\nabla]^2 \beta^m \sigma_1 \partial_m \mathcal{G} 3^y (\nabla_a \sigma_2) (\nabla^a \lambda_y)$$

■ 24)  $(\sigma_1 \partial_\mu \sigma_2 - \sigma_2 \partial_\mu \sigma_1) R$

$$T[10]: \frac{1}{2} R[\nabla] \sigma_1 (\nabla_a \nabla_b \nabla^b b_6) (\nabla^a \sigma_2)$$

$$T[14]: \frac{2}{5} R[\nabla] I_3^m \sigma_1 (\nabla_a \nabla_b \nabla^b \lambda_m) (\nabla^a \sigma_2) + \frac{2}{5} R[\nabla] \sigma_1 (\nabla_a \sigma_2) (\nabla^a I_3^m) (\nabla_b \nabla^b \lambda_m) +$$

$$\frac{2}{5} R[\nabla] \sigma_1 (\nabla^a \lambda^m) (\nabla_b \nabla_a I_3^m) (\nabla^b \sigma_2) + \frac{2}{5} R[\nabla] \sigma_1 (\nabla^a I_3^m) (\nabla_b \nabla_a \lambda_m) (\nabla^b \sigma_2)$$

$$T[15]: \frac{2}{5} R[\nabla] I_4^m \sigma_1 (\nabla_a \nabla_b \nabla^b \lambda_m) (\nabla^a \sigma_2) + \frac{2}{5} R[\nabla] \sigma_1 (\nabla_a \sigma_2) (\nabla^a I_4^m) (\nabla_b \nabla^b \lambda_m) +$$

$$\frac{12}{5} R[\nabla] \sigma_1 (\nabla^a \lambda^m) (\nabla_b \nabla_a I_4^m) (\nabla^b \sigma_2) + \frac{12}{5} R[\nabla] \sigma_1 (\nabla^a I_4^m) (\nabla_b \nabla_a \lambda_m) (\nabla^b \sigma_2)$$

$$T[16]: 2 R[\nabla] I_5^m \sigma_1 (\nabla_a \nabla_b \nabla^b \lambda_m) (\nabla^a \sigma_2) + 2 R[\nabla] \sigma_1 (\nabla_a \sigma_2) (\nabla^a I_5^m) (\nabla_b \nabla^b \lambda_m) +$$

$$\frac{4}{5} R[\nabla] \sigma_1 (\nabla_a \nabla_b \lambda_m) (\nabla^a I_5^m) (\nabla^b \sigma_2) + \frac{4}{5} R[\nabla] \sigma_1 (\nabla_a \nabla_b I_5^m) (\nabla^a \lambda^m) (\nabla^b \sigma_2) +$$

$$\frac{6}{5} R[\nabla] \sigma_1 (\nabla^a \lambda^m) (\nabla_b \nabla_a I_5^m) (\nabla^b \sigma_2) + \frac{6}{5} R[\nabla] \sigma_1 (\nabla^a I_5^m) (\nabla_b \nabla_a \lambda_m) (\nabla^b \sigma_2)$$

$$T[17]: 5 R[\nabla] I_6^m \sigma_1 (\nabla_a \nabla_b \nabla^b \lambda_m) (\nabla^a \sigma_2) +$$

$$2 R[\nabla] \sigma_1 (\nabla_a \sigma_2) (\nabla^a \lambda^m) (\nabla_b \nabla^b I_6^m) + 3 R[\nabla] \sigma_1 (\nabla_a \sigma_2) (\nabla^a I_6^m) (\nabla_b \nabla^b \lambda_m) +$$

$$4 R[\nabla] \sigma_1 (\nabla_a \nabla_b \lambda_m) (\nabla^a I_6^m) (\nabla^b \sigma_2) + 2 R[\nabla] \sigma_1 (\nabla_a \nabla_b I_6^m) (\nabla^a \lambda^m) (\nabla^b \sigma_2) +$$

$$R[\nabla] \sigma_1 (\nabla^a \lambda^m) (\nabla_b \nabla_a I_6^m) (\nabla^b \sigma_2) + 3 R[\nabla] \sigma_1 (\nabla^a I_6^m) (\nabla_b \nabla_a \lambda_m) (\nabla^b \sigma_2)$$

$$\begin{aligned}
\text{T}[18]: & \text{R}[\nabla] \text{I7}^m \sigma 1 (\nabla_a \nabla_b \nabla^b \lambda_m) (\nabla^a \sigma 2) - \frac{1}{2} \text{R}[\nabla] \sigma 1 (\nabla_a \sigma 2) (\nabla^a \lambda^m) (\nabla_b \nabla^b \text{I7}_m) + \\
& \frac{3}{2} \text{R}[\nabla] \sigma 1 (\nabla_a \sigma 2) (\nabla^a \text{I7}^m) (\nabla_b \nabla^b \lambda_m) + \frac{1}{2} \text{R}[\nabla] \sigma 1 (\nabla_a \nabla_b \text{I7}_m) (\nabla^a \lambda^m) (\nabla^b \sigma 2) + \\
& \text{R}[\nabla] \sigma 1 (\nabla^a \lambda^m) (\nabla_b \nabla_a \text{I7}_m) (\nabla^b \sigma 2) + \frac{1}{2} \text{R}[\nabla] \sigma 1 (\nabla^a \text{I7}^m) (\nabla_b \nabla_a \lambda_m) (\nabla^b \sigma 2) \\
\text{T}[21]: & -\frac{2}{5} \text{R}[\nabla] \sigma 1 (\nabla_a \lambda^n) (\nabla^a \lambda^m) (\nabla_b \mathcal{GG}3_{mn}) (\nabla^b \sigma 2) - \frac{4}{5} \text{R}[\nabla] \mathcal{GG}3^{mn} \sigma 1 (\nabla^a \lambda_m) (\nabla_b \nabla_a \lambda_n) (\nabla^b \sigma 2) \\
\text{T}[22]: & -\frac{6}{5} \text{R}[\nabla] \sigma 1 (\nabla_a \lambda^n) (\nabla^a \lambda^m) (\nabla_b \mathcal{GG}4_{mn}) (\nabla^b \sigma 2) - \frac{12}{5} \text{R}[\nabla] \mathcal{GG}4^{mn} \sigma 1 (\nabla^a \lambda_m) (\nabla_b \nabla_a \lambda_n) (\nabla^b \sigma 2) \\
\text{T}[23]: & -4 \text{R}[\nabla] \mathcal{HH}1^{mn} \sigma 1 (\nabla_a \sigma 2) (\nabla^a \lambda_m) (\nabla_b \nabla^b \lambda_n) - \\
& 4 \text{R}[\nabla] \sigma 1 (\nabla_a \sigma 2) (\nabla^a \lambda^m) (\nabla_b \mathcal{HH}1_{mn}) (\nabla^b \lambda^n) - 4 \text{R}[\nabla] \mathcal{HH}1^{mn} \sigma 1 (\nabla_a \nabla_b \lambda_n) (\nabla^a \lambda_m) (\nabla^b \sigma 2) + \\
& 4 \text{R}[\nabla] \sigma 1 (\nabla_a \lambda^n) (\nabla^a \lambda^m) (\nabla_b \mathcal{HH}1_{mn}) (\nabla^b \sigma 2) + 8 \text{R}[\nabla] \mathcal{HH}1^{mn} \sigma 1 (\nabla^a \lambda_m) (\nabla_b \nabla_a \lambda_n) (\nabla^b \sigma 2) \\
\text{T}[24]: & -\frac{2}{5} \text{R}[\nabla] \mathcal{HH}2^{mn} \sigma 1 (\nabla_a \sigma 2) (\nabla^a \lambda_m) (\nabla_b \nabla^b \lambda_n) - \\
& \frac{2}{5} \text{R}[\nabla] \sigma 1 (\nabla_a \sigma 2) (\nabla^a \lambda^m) (\nabla_b \mathcal{HH}2_{mn}) (\nabla^b \lambda^n) - \frac{2}{5} \text{R}[\nabla] \mathcal{HH}2^{mn} \sigma 1 (\nabla_a \nabla_b \lambda_n) (\nabla^a \lambda_m) (\nabla^b \sigma 2) - \\
& \frac{3}{5} \text{R}[\nabla] \sigma 1 (\nabla_a \lambda^n) (\nabla^a \lambda^m) (\nabla_b \mathcal{HH}2_{mn}) (\nabla^b \sigma 2) - \frac{6}{5} \text{R}[\nabla] \mathcal{HH}2^{mn} \sigma 1 (\nabla^a \lambda_m) (\nabla_b \nabla_a \lambda_n) (\nabla^b \sigma 2) \\
\text{T}[25]: & -2 \text{R}[\nabla] \mathcal{HH}3^{mn} \sigma 1 (\nabla_a \sigma 2) (\nabla^a \lambda_m) (\nabla_b \nabla^b \lambda_n) - \\
& 2 \text{R}[\nabla] \sigma 1 (\nabla_a \sigma 2) (\nabla^a \lambda^m) (\nabla_b \mathcal{HH}3_{mn}) (\nabla^b \lambda^n) - 2 \text{R}[\nabla] \mathcal{HH}3^{mn} \sigma 1 (\nabla_a \nabla_b \lambda_n) (\nabla^a \lambda_m) (\nabla^b \sigma 2) - \\
& \frac{1}{2} \text{R}[\nabla] \sigma 1 (\nabla_a \lambda^n) (\nabla^a \lambda^m) (\nabla_b \mathcal{HH}3_{mn}) (\nabla^b \sigma 2) - \text{R}[\nabla] \mathcal{HH}3^{mn} \sigma 1 (\nabla^a \lambda_m) (\nabla_b \nabla_a \lambda_n) (\nabla^b \sigma 2) \\
\text{T}[26]: & -\frac{1}{2} \text{R}[\nabla] \sigma 1 (\nabla_a \lambda^n) (\nabla^a \lambda^m) (\nabla_b \mathcal{HH}4_{mn}) (\nabla^b \sigma 2) - \text{R}[\nabla] \mathcal{HH}4^{mn} \sigma 1 (\nabla^a \lambda_m) (\nabla_b \nabla_a \lambda_n) (\nabla^b \sigma 2) \\
\text{T}[27]: & -2 \text{R}[\nabla] \mathcal{HH}5^{mn} \sigma 1 (\nabla_a \sigma 2) (\nabla^a \lambda_m) (\nabla_b \nabla^b \lambda_n) - \\
& 6 \text{R}[\nabla] \sigma 1 (\nabla_a \sigma 2) (\nabla^a \lambda^m) (\nabla_b \mathcal{HH}5_{mn}) (\nabla^b \lambda^n) - 4 \text{R}[\nabla] \mathcal{HH}5^{mn} \sigma 1 (\nabla_a \nabla_b \lambda_n) (\nabla^a \lambda_m) (\nabla^b \sigma 2) - \\
& \text{R}[\nabla] \sigma 1 (\nabla_a \lambda^n) (\nabla^a \lambda^m) (\nabla_b \mathcal{HH}5_{mn}) (\nabla^b \sigma 2) - 2 \text{R}[\nabla] \mathcal{HH}5^{mn} \sigma 1 (\nabla^a \lambda_m) (\nabla_b \nabla_a \lambda_n) (\nabla^b \sigma 2) \\
\text{T}[28]: & -\frac{1}{5} \text{R}[\nabla] \mathcal{HH}6^{mn} \sigma 1 (\nabla_a \sigma 2) (\nabla^a \lambda_m) (\nabla_b \nabla^b \lambda_n) - \\
& \frac{1}{5} \text{R}[\nabla] \sigma 1 (\nabla_a \sigma 2) (\nabla^a \lambda^m) (\nabla_b \mathcal{HH}6_{mn}) (\nabla^b \lambda^n) - \frac{1}{5} \text{R}[\nabla] \mathcal{HH}6^{mn} \sigma 1 (\nabla_a \nabla_b \lambda_n) (\nabla^a \lambda_m) (\nabla^b \sigma 2) - \\
& \frac{1}{2} \text{R}[\nabla] \sigma 1 (\nabla_a \lambda^n) (\nabla^a \lambda^m) (\nabla_b \mathcal{HH}6_{mn}) (\nabla^b \sigma 2) - \text{R}[\nabla] \mathcal{HH}6^{mn} \sigma 1 (\nabla^a \lambda_m) (\nabla_b \nabla_a \lambda_n) (\nabla^b \sigma 2) \\
\text{T}[29]: & \text{R}[\nabla] \mathcal{FF}^{mn} \sigma 1 (\nabla_a \sigma 2) (\nabla^a \lambda_n) (\nabla_b \nabla^b \lambda_m) + \\
& \text{R}[\nabla] \sigma 1 (\nabla_a \lambda_m) (\nabla^a \mathcal{FF}^{mn}) (\nabla_b \sigma 2) (\nabla^b \lambda_n) + 2 \text{R}[\nabla] \mathcal{FF}^{mn} \sigma 1 (\nabla_a \nabla_b \lambda_n) (\nabla^a \lambda_m) (\nabla^b \sigma 2) \\
\text{T}[30]: & \text{R}[\nabla] \mathcal{FFP}^{mn} \sigma 1 (\nabla_a \sigma 2) (\nabla^a \lambda_m) (\nabla_b \nabla^b \lambda_n) - \text{R}[\nabla] \sigma 1 (\nabla_a \sigma 2) (\nabla^a \mathcal{FFP}^{mn}) (\nabla_b \lambda_n) (\nabla^b \lambda_m) + \\
& 2 \text{R}[\nabla] \sigma 1 (\nabla_a \lambda_n) (\nabla^a \mathcal{FFP}^{mn}) (\nabla_b \sigma 2) (\nabla^b \lambda_m) + 2 \text{R}[\nabla] \mathcal{FFP}^{mn} \sigma 1 (\nabla_a \nabla_b \lambda_m) (\nabla^a \lambda_n) (\nabla^b \sigma 2) - \\
& \text{R}[\nabla] \mathcal{FFP}^{mn} \sigma 1 (\nabla^a \lambda_n) (\nabla_b \nabla_a \lambda_m) (\nabla^b \sigma 2) - \text{R}[\nabla] \mathcal{FFP}^{mn} \sigma 1 (\nabla^a \lambda_m) (\nabla_b \nabla_a \lambda_n) (\nabla^b \sigma 2) \\
\text{T}[31]: & \text{R}[\nabla] \mathcal{FFP}^{mnp} \sigma 1 (\nabla_a \lambda_n) (\nabla^a \lambda_m) (\nabla_b \sigma 2) (\nabla^b \lambda_p) \\
\text{T}[32]: & \frac{2}{5} \text{R}[\nabla] \delta\delta\text{hat}^{mn} \sigma 1 (\nabla_a \sigma 2) (\nabla^a \lambda_m) (\nabla_b \nabla^b \lambda_n)
\end{aligned}$$

$$\begin{aligned}
\text{T}[33] &: \frac{1}{5} \text{R}[\nabla] \ \varepsilon \varepsilon \varepsilon^{\text{mnp}} \ \sigma 1 \ (\nabla_a \sigma 2) \ (\nabla^a \lambda_m) \ (\nabla_b \lambda_p) \ (\nabla^b \lambda_n) \\
\text{T}[34] &: \frac{1}{2} \text{R}[\nabla] \ \mathcal{D}\mathcal{D}\mathcal{D}^{\text{mnp}} \ \sigma 1 \ (\nabla_a \sigma 2) \ (\nabla^a \lambda_m) \ (\nabla_b \lambda_p) \ (\nabla^b \lambda_n) + \\
&\quad \frac{1}{2} \text{R}[\nabla] \ \mathcal{D}\mathcal{D}\mathcal{D}^{\text{mnp}} \ \sigma 1 \ (\nabla_a \lambda_p) \ (\nabla^a \lambda_m) \ (\nabla_b \sigma 2) \ (\nabla^b \lambda_n) - \text{R}[\nabla] \ \mathcal{D}\mathcal{D}\mathcal{D}^{\text{mnp}} \ \sigma 1 \ (\nabla_a \lambda_n) \ (\nabla^a \lambda_m) \ (\nabla_b \sigma 2) \ (\nabla^b \lambda_p) \\
\text{T}[37] &: -\frac{1}{2} \text{R}[\nabla] \ \mathcal{C}\mathcal{C}\text{hatp}^{\text{mn}} \ \sigma 1 \ (\nabla_a \nabla_b \lambda_n) \ (\nabla^a \lambda_m) \ (\nabla^b \sigma 2) \\
\text{T}[38] &: -\frac{1}{2} \text{R}[\nabla] \ \mathcal{C}\mathcal{C}\mathcal{C}^{\text{mnp}} \ \sigma 1 \ (\nabla_a \lambda_p) \ (\nabla^a \lambda_m) \ (\nabla_b \sigma 2) \ (\nabla^b \lambda_n) \\
\text{T}[39] &: -\text{R}[\nabla] \ \mathcal{C}\mathcal{C}\mathcal{C}\mathcal{P}^{\text{mnp}} \ \sigma 1 \ (\nabla_a \sigma 2) \ (\nabla^a \lambda_m) \ (\nabla_b \lambda_p) \ (\nabla^b \lambda_n) \\
\text{T}[42] &: \frac{1}{5} \text{R}[\nabla] \ \beta^{\text{m}} \ \sigma 1 \ (\nabla_a \nabla_b \nabla^b \beta_m) \ (\nabla^a \sigma 2) - \frac{1}{5} \text{R}[\nabla] \ \beta^{\text{m}} \ \sigma 1 \ (\nabla_a \nabla_b \nabla^b \beta_m) \ (\nabla^a \sigma 2) - \\
&\quad \frac{2}{5} \text{R}[\nabla] \ \beta^{\text{m}} \ \sigma 1 \ (\nabla_a \nabla_b \nabla^b \lambda_m) \ (\nabla^a \sigma 2) + \frac{1}{5} \text{R}[\nabla] \ \sigma 1 \ (\nabla_a \sigma 2) \ (\nabla^a \beta^{\text{m}}) \ (\nabla_b \nabla^b \beta_m) - \\
&\quad \frac{1}{5} \text{R}[\nabla] \ \sigma 1 \ (\nabla_a \sigma 2) \ (\nabla^a \beta^{\text{m}}) \ (\nabla_b \nabla^b \beta_m) - \frac{6}{5} \text{R}[\nabla] \ \sigma 1 \ (\nabla_a \sigma 2) \ (\nabla^a \beta^{\text{m}}) \ (\nabla_b \nabla^b \lambda_m) + \\
&\quad \frac{2}{5} \text{R}[\nabla] \ \sigma 1 \ (\nabla_a \nabla_b \beta_m) \ (\nabla^a \beta^{\text{m}}) \ (\nabla^b \sigma 2) + \frac{4}{5} \text{R}[\nabla] \ \sigma 1 \ (\nabla_a \nabla_b \lambda_m) \ (\nabla^a \beta^{\text{m}}) \ (\nabla^b \sigma 2) - \\
&\quad \frac{2}{5} \text{R}[\nabla] \ \sigma 1 \ (\nabla_a \nabla_b \beta_m) \ (\nabla^a \beta^{\text{m}}) \ (\nabla^b \sigma 2) - \frac{4}{5} \text{R}[\nabla] \ \sigma 1 \ (\nabla_a \nabla_b \beta_m) \ (\nabla^a \lambda^{\text{m}}) \ (\nabla^b \sigma 2) \\
\text{T}[43] &: \frac{1}{5} \text{R}[\nabla] \ \mathcal{B}\mathcal{B}\text{hat}_m^{\text{n}} \ \beta^{\text{m}} \ \sigma 1 \ (\nabla_a \nabla_b \nabla^b \lambda_n) \ (\nabla^a \sigma 2) - \frac{1}{5} \text{R}[\nabla] \ \mathcal{B}\mathcal{B}\text{hat}^{\text{mn}} \ \sigma 1 \ (\nabla_a \sigma 2) \ (\nabla^a \beta_m) \ (\nabla_b \nabla^b \lambda_n) - \\
&\quad \frac{4}{5} \text{R}[\nabla] \ \mathcal{B}\mathcal{B}\text{hat}^{\text{mn}} \ \sigma 1 \ (\nabla_a \sigma 2) \ (\nabla^a \lambda_m) \ (\nabla_b \nabla^b \lambda_n) + \frac{1}{5} \text{R}[\nabla] \ \beta^{\text{m}} \ \sigma 1 \ (\nabla_a \mathcal{B}\mathcal{B}\text{hat}_m^{\text{n}}) \ (\nabla^a \sigma 2) \ (\nabla_b \nabla^b \lambda_n) \\
\text{T}[44] &: \\
&\quad \frac{1}{5} \text{R}[\nabla] \ \mathcal{B}\mathcal{B}\text{hatp}_m^{\text{n}} \ \beta^{\text{m}} \ \sigma 1 \ (\nabla_a \nabla_b \nabla^b \lambda_n) \ (\nabla^a \sigma 2) - \frac{1}{5} \text{R}[\nabla] \ \mathcal{B}\mathcal{B}\text{hatp}^{\text{mn}} \ \sigma 1 \ (\nabla_a \sigma 2) \ (\nabla^a \lambda_m) \ (\nabla_b \nabla^b \lambda_n) + \\
&\quad \frac{1}{5} \text{R}[\nabla] \ \beta^{\text{m}} \ \sigma 1 \ (\nabla^a \sigma 2) \ (\nabla_b \nabla_a \lambda_n) \ (\nabla^b \mathcal{B}\mathcal{B}\text{hatp}_m^{\text{n}}) + \frac{1}{5} \text{R}[\nabla] \ \mathcal{B}\mathcal{B}\text{hatp}^{\text{mn}} \ \sigma 1 \ (\nabla_a \nabla_b \lambda_n) \ (\nabla^a \lambda_m) \ (\nabla^b \sigma 2) - \\
&\quad \frac{1}{5} \text{R}[\nabla] \ \mathcal{B}\mathcal{B}\text{hatp}^{\text{mn}} \ \sigma 1 \ (\nabla^a \beta_m) \ (\nabla_b \nabla_a \lambda_n) \ (\nabla^b \sigma 2) + \frac{1}{5} \text{R}[\nabla] \ \mathcal{B}\mathcal{B}\text{hatp}^{\text{mn}} \ \sigma 1 \ (\nabla^a \lambda_m) \ (\nabla_b \nabla_a \lambda_n) \ (\nabla^b \sigma 2) \\
\text{T}[45] &: -\frac{1}{5} \text{R}[\nabla] \ \mathcal{B}\mathcal{B}\mathcal{B}_m^{\text{np}} \ \beta^{\text{m}} \ \sigma 1 \ (\nabla_a \sigma 2) \ (\nabla^a \lambda_n) \ (\nabla_b \nabla^b \lambda_p) - \\
&\quad \frac{1}{10} \text{R}[\nabla] \ \mathcal{B}\mathcal{B}\mathcal{B}^{\text{mnp}} \ \sigma 1 \ (\nabla_a \sigma 2) \ (\nabla^a \beta_p) \ (\nabla_b \lambda_n) \ (\nabla^b \lambda_m) - \\
&\quad \frac{2}{5} \text{R}[\nabla] \ \mathcal{B}\mathcal{B}\mathcal{B}^{\text{mnp}} \ \sigma 1 \ (\nabla_a \lambda_n) \ (\nabla^a \lambda_m) \ (\nabla_b \sigma 2) \ (\nabla^b \lambda_p) + \\
&\quad \frac{1}{10} \text{R}[\nabla] \ \beta^{\text{m}} \ \sigma 1 \ (\nabla_a \lambda^{\text{p}}) \ (\nabla^a \lambda^{\text{n}}) \ (\nabla_b \mathcal{B}\mathcal{B}\mathcal{B}_{\text{npm}}) \ (\nabla^b \sigma 2) + \\
&\quad \frac{1}{5} \text{R}[\nabla] \ \mathcal{B}\mathcal{B}\mathcal{B}_m^{\text{np}} \ \beta^{\text{m}} \ \sigma 1 \ (\nabla^a \lambda_n) \ (\nabla_b \nabla_a \lambda_p) \ (\nabla^b \sigma 2)
\end{aligned}$$



$$\begin{aligned}
T[46]: & \frac{1}{10} R[\nabla] \mathcal{BBBp}^{np}_m \beta^m \sigma 1 (\nabla_a \sigma 2) (\nabla^a \lambda_n) (\nabla_b \nabla^b \lambda_p) - \\
& \frac{1}{10} R[\nabla] \mathcal{BBBp}^{mnp} \sigma 1 (\nabla_a \lambda_m) (\nabla^a \beta_p) (\nabla_b \sigma 2) (\nabla^b \lambda_n) + \\
& \frac{1}{5} R[\nabla] \mathcal{BBBp}^{mnp} \sigma 1 (\nabla_a \lambda_p) (\nabla^a \lambda_m) (\nabla_b \sigma 2) (\nabla^b \lambda_n) - \\
& \frac{1}{10} R[\nabla] \mathcal{BBBp}^{mnp} \sigma 1 (\nabla_a \lambda_n) (\nabla^a \lambda_m) (\nabla_b \sigma 2) (\nabla^b \lambda_p) + \\
& \frac{1}{10} R[\nabla] \beta^m \sigma 1 (\nabla_a \sigma 2) (\nabla^a \lambda^n) (\nabla_b \mathcal{BBBp}_{npm}) (\nabla^b \lambda^p) - \\
& \frac{1}{10} R[\nabla] \mathcal{BBBp}^{np}_m \beta^m \sigma 1 (\nabla_a \nabla_b \lambda_p) (\nabla^a \lambda_n) (\nabla^b \sigma 2) + \\
& \frac{1}{10} R[\nabla] \mathcal{BBBp}^{np}_m \beta^m \sigma 1 (\nabla_a \nabla_b \lambda_p) (\nabla^a \lambda_n) (\nabla^b \sigma 2) - \\
& \frac{1}{10} R[\nabla] \mathcal{BBBp}^{np}_m \beta^m \sigma 1 (\nabla^a \lambda_n) (\nabla_b \nabla_a \lambda_p) (\nabla^b \sigma 2)
\end{aligned}$$

$$T[47]: -\frac{1}{5} R[\nabla] \mathcal{BBBp}^{nop}_m \beta^m \sigma 1 (\nabla_a \lambda_o) (\nabla^a \lambda_n) (\nabla_b \sigma 2) (\nabla^b \lambda_p)$$

$$\begin{aligned}
T[48]: & R[\nabla] \sigma 1 (\nabla_a \sigma 2) (\nabla^a \beta^m) (\nabla_b \nabla^b \mathcal{J}_m) + 2 R[\nabla] \sigma 1 (\nabla_a \sigma 2) (\nabla^a \lambda^m) (\nabla_b \nabla^b \mathcal{J}_m) - \\
& R[\nabla] \sigma 1 (\nabla_a \sigma 2) (\nabla^a \mathcal{J}^m) (\nabla_b \nabla^b \beta_m) - 2 R[\nabla] \sigma 1 (\nabla_a \sigma 2) (\nabla^a \mathcal{J}^m) (\nabla_b \nabla^b \lambda_m) + \\
& R[\nabla] \sigma 1 (\nabla_a \nabla_b \beta_m) (\nabla^a \mathcal{J}^m) (\nabla^b \sigma 2) + 2 R[\nabla] \sigma 1 (\nabla_a \nabla_b \lambda_m) (\nabla^a \mathcal{J}^m) (\nabla^b \sigma 2) - \\
& R[\nabla] \sigma 1 (\nabla_a \nabla_b \mathcal{J}_m) (\nabla^a \beta^m) (\nabla^b \sigma 2) - 2 R[\nabla] \sigma 1 (\nabla_a \nabla_b \mathcal{J}_m) (\nabla^a \lambda^m) (\nabla^b \sigma 2)
\end{aligned}$$

$$T[51]:$$

$$\begin{aligned}
& -R[\nabla] \mathcal{AAhatpp}^n_m \beta^m \sigma 1 (\nabla_a \nabla_b \nabla^b \lambda_n) (\nabla^a \sigma 2) - \frac{1}{2} R[\nabla] \mathcal{AAhatpp}^n_m \beta^m \sigma 1 (\nabla^a \sigma 2) (\nabla_b \nabla^b \nabla_a \lambda_n) - \\
& 2 R[\nabla] \beta^m \sigma 1 (\nabla^a \sigma 2) (\nabla_b \nabla_a \lambda_n) (\nabla^b \mathcal{AAhatpp}^n_m) - \frac{3}{2} R[\nabla] \mathcal{AAhatpp}^{mn} \sigma 1 (\nabla_a \nabla_b \lambda_n) (\nabla^a \lambda_m) (\nabla^b \sigma 2) + \\
& R[\nabla] \mathcal{AAhatpp}^{mn} \sigma 1 (\nabla^a \beta_m) (\nabla_b \nabla_a \lambda_n) (\nabla^b \sigma 2) - \frac{3}{2} R[\nabla] \mathcal{AAhatpp}^{mn} \sigma 1 (\nabla^a \lambda_m) (\nabla_b \nabla_a \lambda_n) (\nabla^b \sigma 2)
\end{aligned}$$

$$T[53]: \frac{1}{2} R[\nabla] \mathcal{AAhatp}^{np}_m \beta^m \sigma 1 (\nabla_a \sigma 2) (\nabla^a \lambda_n) (\nabla_b \nabla^b \lambda_p)$$

$$\begin{aligned}
T[55]: & \frac{1}{2} R[\nabla] \mathcal{AAhatp}^{mnp} \sigma 1 (\nabla_a \sigma 2) (\nabla^a \beta_p) (\nabla_b \lambda_n) (\nabla^b \lambda_m) + \\
& 2 R[\nabla] \mathcal{AAhatp}^{mnp} \sigma 1 (\nabla_a \lambda_n) (\nabla^a \lambda_m) (\nabla_b \sigma 2) (\nabla^b \lambda_p) - \\
& \frac{1}{2} R[\nabla] \beta^m \sigma 1 (\nabla_a \lambda^p) (\nabla^a \lambda^n) (\nabla_b \mathcal{AAhatp}_{npm}) (\nabla^b \sigma 2) - \\
& R[\nabla] \mathcal{AAhatp}^{np}_m \beta^m \sigma 1 (\nabla^a \lambda_n) (\nabla_b \nabla_a \lambda_p) (\nabla^b \sigma 2)
\end{aligned}$$

$$\begin{aligned}
T[56]: & -\frac{1}{2} R[\nabla] \mathcal{AAcheckp}^{mnp} \sigma 1 (\nabla_a \sigma 2) (\nabla^a \beta_p) (\nabla_b \lambda_n) (\nabla^b \lambda_m) - \\
& 2 R[\nabla] \mathcal{AAcheckp}^{mnp} \sigma 1 (\nabla_a \lambda_n) (\nabla^a \lambda_m) (\nabla_b \sigma 2) (\nabla^b \lambda_p) + \\
& \frac{1}{2} R[\nabla] \beta^m \sigma 1 (\nabla_a \lambda^p) (\nabla^a \lambda^n) (\nabla_b \mathcal{AAcheckp}_{npm}) (\nabla^b \sigma 2) + \\
& R[\nabla] \mathcal{AAcheckp}^{np}_m \beta^m \sigma 1 (\nabla^a \lambda_n) (\nabla_b \nabla_a \lambda_p) (\nabla^b \sigma 2)
\end{aligned}$$

$$\begin{aligned}
T[57]: & -\frac{1}{4} R[\nabla] \mathcal{A}\mathcal{A}\mathcal{A}\text{checkpp}^{\text{mnp}} \sigma_1 (\nabla_a \sigma_2) (\nabla^a \beta_p) (\nabla_b \lambda_n) (\nabla^b \lambda_m) + \\
& \frac{1}{2} R[\nabla] \mathcal{A}\mathcal{A}\mathcal{A}\text{checkpp}^{\text{mnp}} \sigma_1 (\nabla_a \lambda_m) (\nabla^a \beta_p) (\nabla_b \sigma_2) (\nabla^b \lambda_n) + \\
& R[\nabla] \mathcal{A}\mathcal{A}\mathcal{A}\text{checkpp}^{\text{mnp}} \sigma_1 (\nabla_a \lambda_p) (\nabla^a \lambda_m) (\nabla_b \sigma_2) (\nabla^b \lambda_n) - \\
& R[\nabla] \mathcal{A}\mathcal{A}\mathcal{A}\text{checkpp}^{\text{mnp}} \sigma_1 (\nabla_a \lambda_n) (\nabla^a \lambda_m) (\nabla_b \sigma_2) (\nabla^b \lambda_p) + \\
& \frac{1}{4} R[\nabla] \beta^m \sigma_1 (\nabla_a \lambda^p) (\nabla^a \lambda^n) (\nabla_b \mathcal{A}\mathcal{A}\mathcal{A}\text{checkpp}_{\text{npm}}) (\nabla^b \sigma_2) + \\
& \frac{1}{2} R[\nabla] \mathcal{A}\mathcal{A}\mathcal{A}\text{checkpp}^{\text{np}}_m \beta^m \sigma_1 (\nabla^a \lambda_n) (\nabla_b \nabla_a \lambda_p) (\nabla^b \sigma_2)
\end{aligned}$$

$$T[59]: \frac{1}{4} R[\nabla] \mathcal{A}\mathcal{A}\mathcal{A}\text{hatp}^{\text{no p}}_m \beta^m \sigma_1 (\nabla_a \lambda_o) (\nabla^a \lambda_n) (\nabla_b \sigma_2) (\nabla^b \lambda_p)$$

$$\begin{aligned}
T[60]: & \frac{1}{4} R[\nabla] \mathcal{A}\mathcal{A}\mathcal{A}\text{hatpp}^{\text{no p}}_m \beta^m \sigma_1 (\nabla_a \lambda_p) (\nabla^a \lambda_n) (\nabla_b \sigma_2) (\nabla^b \lambda_o) + \\
& \frac{1}{4} R[\nabla] \mathcal{A}\mathcal{A}\mathcal{A}\text{hatpp}^{\text{nop}}_m \beta^m \sigma_1 (\nabla_a \lambda_p) (\nabla^a \lambda_n) (\nabla_b \sigma_2) (\nabla^b \lambda_o)
\end{aligned}$$

$$T[62]: -\frac{1}{2} R[\nabla] \mathcal{A}\mathcal{A}\mathcal{A}\text{checkp}^{\text{nop}}_m \beta^m \sigma_1 (\nabla_a \lambda_o) (\nabla^a \lambda_n) (\nabla_b \sigma_2) (\nabla^b \lambda_p)$$

$$\begin{aligned}
Z[25]: & \frac{1}{5} R[\nabla] \mathcal{B}\mathcal{B}^{\text{mn}} \sigma_1 (\nabla_a \sigma_2) (\nabla^a \lambda_m) (\nabla_b \nabla^b \beta_n) + \\
& \frac{1}{5} R[\nabla] \mathcal{B}\mathcal{B}^{\text{mn}} \sigma_1 (\nabla_a \sigma_2) (\nabla^a \beta_m) (\nabla_b \nabla^b \lambda_n) + \frac{1}{5} R[\nabla] \beta^m \sigma_1 \partial_m \mathcal{B}\mathcal{B}_n^o (\nabla_a \sigma_2) (\nabla^a \lambda^n) (\nabla_b \nabla^b \lambda_o)
\end{aligned}$$

■ 25)  $(\sigma_1 \partial_\mu \sigma_2 - \sigma_2 \partial_\mu \sigma_1) \partial^\mu R$

$$T[10]: \frac{1}{2} \sigma_1 (\nabla_a \sigma_2) (\nabla^a R[\nabla]) (\nabla_b \nabla^b b_6)$$

$$T[14]: \frac{2}{5} I 3^m \sigma_1 (\nabla_a \sigma_2) (\nabla^a R[\nabla]) (\nabla_b \nabla^b \lambda_m) + \frac{2}{5} \sigma_1 (\nabla_a \sigma_2) (\nabla^a R[\nabla]) (\nabla_b \lambda_m) (\nabla^b I 3^m)$$

$$T[15]: \frac{2}{5} I 4^m \sigma_1 (\nabla_a \sigma_2) (\nabla^a R[\nabla]) (\nabla_b \nabla^b \lambda_m) + \frac{12}{5} \sigma_1 (\nabla_a \sigma_2) (\nabla^a R[\nabla]) (\nabla_b \lambda_m) (\nabla^b I 4^m)$$

$$T[16]: \frac{6}{5} I 5^m \sigma_1 (\nabla_a \sigma_2) (\nabla^a R[\nabla]) (\nabla_b \nabla^b \lambda_m) + \frac{6}{5} \sigma_1 (\nabla_a \sigma_2) (\nabla^a R[\nabla]) (\nabla_b \lambda_m) (\nabla^b I 5^m)$$

$$T[17]: I 6^m \sigma_1 (\nabla_a \sigma_2) (\nabla^a R[\nabla]) (\nabla_b \nabla^b \lambda_m) + \sigma_1 (\nabla_a \sigma_2) (\nabla^a R[\nabla]) (\nabla_b \lambda_m) (\nabla^b I 6^m)$$

$$T[18]: 3 I 7^m \sigma_1 (\nabla_a \sigma_2) (\nabla^a R[\nabla]) (\nabla_b \nabla^b \lambda_m) + 3 \sigma_1 (\nabla_a \sigma_2) (\nabla^a R[\nabla]) (\nabla_b \lambda_m) (\nabla^b I 7^m)$$

$$T[21]: -\frac{2}{5} \mathcal{G}\mathcal{G} 3^{\text{mn}} \sigma_1 (\nabla_a \sigma_2) (\nabla^a R[\nabla]) (\nabla_b \lambda_n) (\nabla^b \lambda_m)$$

$$T[22]: -\frac{6}{5} \mathcal{G}\mathcal{G} 4^{\text{mn}} \sigma_1 (\nabla_a \sigma_2) (\nabla^a R[\nabla]) (\nabla_b \lambda_n) (\nabla^b \lambda_m)$$

$$T[24]: -\frac{3}{5} \mathcal{H}\mathcal{H} 2^{\text{mn}} \sigma_1 (\nabla_a \sigma_2) (\nabla^a R[\nabla]) (\nabla_b \lambda_n) (\nabla^b \lambda_m)$$

$$T[25]: -\frac{1}{2} \mathcal{H}\mathcal{H} 3^{\text{mn}} \sigma_1 (\nabla_a \sigma_2) (\nabla^a R[\nabla]) (\nabla_b \lambda_n) (\nabla^b \lambda_m)$$

$$T[26]: -\frac{3}{2} \mathcal{HH}4^{mn} \sigma_1 (\nabla_a \sigma_2) (\nabla^a R[\nabla]) (\nabla_b \lambda_n) (\nabla^b \lambda_m)$$

$$T[27]: -\mathcal{HH}5^{mn} \sigma_1 (\nabla_a \sigma_2) (\nabla^a R[\nabla]) (\nabla_b \lambda_n) (\nabla^b \lambda_m)$$

$$T[28]: -\frac{3}{5} \mathcal{HH}6^{mn} \sigma_1 (\nabla_a \sigma_2) (\nabla^a R[\nabla]) (\nabla_b \lambda_n) (\nabla^b \lambda_m)$$

$$T[30]:$$

$$-\frac{1}{4} \mathcal{FFP}^{mn} \beta_n \sigma_1 (\nabla_a \sigma_2) (\nabla^a R[\nabla]) (\nabla_b \nabla^b \lambda_m) - \frac{1}{4} \beta^m \sigma_1 (\nabla_a \sigma_2) (\nabla^a R[\nabla]) (\nabla_b \lambda_n) (\nabla^b \mathcal{FFP}^n_m) -$$

$$\frac{1}{4} \mathcal{FFP}^{mn} \sigma_1 (\nabla_a \sigma_2) (\nabla^a R[\nabla]) (\nabla_b \lambda_m) (\nabla^b \beta_n) - \mathcal{FFP}^{mn} \sigma_1 (\nabla_a \sigma_2) (\nabla^a R[\nabla]) (\nabla_b \lambda_n) (\nabla^b \lambda_m)$$

$$T[32]: -\frac{1}{5} \mathcal{E}\mathcal{E}\mathcal{H}\mathcal{A}\mathcal{T}^{mn} \beta_m \sigma_1 (\nabla_a \sigma_2) (\nabla^a R[\nabla]) (\nabla_b \nabla^b \lambda_n)$$

$$T[33]: -\frac{1}{10} \mathcal{E}\mathcal{E}\mathcal{E}_m^{np} \beta^m \sigma_1 (\nabla_a \sigma_2) (\nabla^a R[\nabla]) (\nabla_b \lambda_p) (\nabla^b \lambda_n)$$

$$T[34]: \frac{1}{2} \mathcal{DDD}^{mnp} \beta_p \sigma_1 (\nabla_a \sigma_2) (\nabla^a R[\nabla]) (\nabla_b \lambda_n) (\nabla^b \lambda_m)$$

$$T[42]: \frac{1}{5} \beta^m \sigma_1 (\nabla_a \sigma_2) (\nabla^a R[\nabla]) (\nabla_b \nabla^b \mathcal{B}_m) -$$

$$\frac{1}{5} \mathcal{B}^m \sigma_1 (\nabla_a \sigma_2) (\nabla^a R[\nabla]) (\nabla_b \nabla^b \beta_m) - \frac{6}{5} \mathcal{B}^m \sigma_1 (\nabla_a \sigma_2) (\nabla^a R[\nabla]) (\nabla_b \nabla^b \lambda_m) -$$

$$\frac{2}{5} \sigma_1 (\nabla_a \sigma_2) (\nabla^a R[\nabla]) (\nabla_b \beta_m) (\nabla^b \mathcal{B}^m) - \frac{4}{5} \sigma_1 (\nabla_a \sigma_2) (\nabla^a R[\nabla]) (\nabla_b \lambda_m) (\nabla^b \mathcal{B}^m)$$

$$T[43]: \frac{1}{5} \mathcal{BB}\mathcal{H}\mathcal{A}\mathcal{T}_m^n \beta^m \sigma_1 (\nabla_a \sigma_2) (\nabla^a R[\nabla]) (\nabla_b \nabla^b \lambda_n)$$

$$T[45]: \frac{1}{10} \mathcal{BBB}^{np}_m \beta^m \sigma_1 (\nabla_a \sigma_2) (\nabla^a R[\nabla]) (\nabla_b \lambda_p) (\nabla^b \lambda_n)$$

$$T[51]: \frac{1}{2} \mathcal{AA}\mathcal{H}\mathcal{A}\mathcal{T}\mathcal{P}\mathcal{P}_m^n \beta^m \sigma_1 (\nabla_a \sigma_2) (\nabla^a R[\nabla]) (\nabla_b \nabla^b \lambda_n) +$$

$$\frac{1}{2} \mathcal{AA}\mathcal{H}\mathcal{A}\mathcal{T}\mathcal{P}\mathcal{P}^{mn} \sigma_1 (\nabla_a \sigma_2) (\nabla^a R[\nabla]) (\nabla_b \lambda_n) (\nabla^b \beta_m) -$$

$$\mathcal{AA}\mathcal{H}\mathcal{A}\mathcal{T}\mathcal{P}\mathcal{P}^{mn} \sigma_1 (\nabla_a \sigma_2) (\nabla^a R[\nabla]) (\nabla_b \lambda_n) (\nabla^b \lambda_m) -$$

$$\frac{1}{2} \beta^m \sigma_1 (\nabla_a \sigma_2) (\nabla^a R[\nabla]) (\nabla_b \mathcal{AA}\mathcal{H}\mathcal{A}\mathcal{T}\mathcal{P}\mathcal{P}_{mn}) (\nabla^b \lambda^n)$$

$$T[55]: -\frac{1}{2} \mathcal{AA}\mathcal{H}\mathcal{A}\mathcal{T}\mathcal{P}^{np}_m \beta^m \sigma_1 (\nabla_a \sigma_2) (\nabla^a R[\nabla]) (\nabla_b \lambda_p) (\nabla^b \lambda_n)$$

$$T[56]: \frac{1}{2} \mathcal{AA}\mathcal{C}\mathcal{H}\mathcal{E}\mathcal{C}\mathcal{K}\mathcal{P}^{np}_m \beta^m \sigma_1 (\nabla_a \sigma_2) (\nabla^a R[\nabla]) (\nabla_b \lambda_p) (\nabla^b \lambda_n)$$

$$T[57]: \frac{1}{4} \mathcal{AA}\mathcal{C}\mathcal{H}\mathcal{E}\mathcal{C}\mathcal{K}\mathcal{P}^{np}_m \beta^m \sigma_1 (\nabla_a \sigma_2) (\nabla^a R[\nabla]) (\nabla_b \lambda_p) (\nabla^b \lambda_n)$$

$$Z[18]: \frac{1}{2} \mathcal{F}^m \sigma_1 (\nabla_a \sigma_2) (\nabla^a R[\nabla]) (\nabla_b \nabla^b \beta_m) + \frac{1}{2} \beta^m \sigma_1 \partial_m \mathcal{F}^n (\nabla_a \sigma_2) (\nabla^a R[\nabla]) (\nabla_b \nabla^b \lambda_n)$$

$$Z[19]: \frac{1}{5} \mathcal{E}^m \sigma_1 (\nabla_a \sigma_2) (\nabla^a R[\nabla]) (\nabla_b \nabla^b \beta_m) + \frac{1}{5} \beta^m \sigma_1 \partial_m \mathcal{E}^n (\nabla_a \sigma_2) (\nabla^a R[\nabla]) (\nabla_b \nabla^b \lambda_n)$$

■ 26)  $(\sigma_1 \partial_\mu \sigma_2 - \sigma_2 \partial_\mu \sigma_1) \partial_\nu R$

$$T[10]: \sigma_1 (\nabla^a R[\nabla]) (\nabla_b \nabla_a b6) (\nabla^b \sigma_2)$$

$$T[11]: -4 \sigma_1 (\nabla^a R[\nabla]) (\nabla_b \nabla_a b7) (\nabla^b \sigma_2)$$

$$T[16]: -\frac{4}{5} \sigma_1 (\nabla_a \lambda_m) (\nabla^a R[\nabla]) (\nabla_b \sigma_2) (\nabla^b I5^m) + \frac{4}{5} I5^m \sigma_1 (\nabla_a \nabla_b \lambda_m) (\nabla^a R[\nabla]) (\nabla^b \sigma_2)$$

$$T[17]: 2 \sigma_1 (\nabla_a \lambda_m) (\nabla^a R[\nabla]) (\nabla_b \sigma_2) (\nabla^b I6^m) + 2 \sigma_1 (\nabla_a I6^m) (\nabla^a R[\nabla]) (\nabla_b \sigma_2) (\nabla^b \lambda_m) + \\ 2 I6^m \sigma_1 (\nabla_a \nabla_b \lambda_m) (\nabla^a R[\nabla]) (\nabla^b \sigma_2) + 2 I6^m \sigma_1 (\nabla^a R[\nabla]) (\nabla_b \nabla_a \lambda_m) (\nabla^b \sigma_2)$$

$$T[18]: \frac{1}{2} \sigma_1 (\nabla_a \lambda_m) (\nabla^a R[\nabla]) (\nabla_b \sigma_2) (\nabla^b I7^m) - \frac{5}{2} \sigma_1 (\nabla_a I7^m) (\nabla^a R[\nabla]) (\nabla_b \sigma_2) (\nabla^b \lambda_m) +$$

$$\frac{1}{2} I7^m \sigma_1 (\nabla_a \nabla_b \lambda_m) (\nabla^a R[\nabla]) (\nabla^b \sigma_2) - \frac{5}{2} I7^m \sigma_1 (\nabla^a R[\nabla]) (\nabla_b \nabla_a \lambda_m) (\nabla^b \sigma_2)$$

$$T[24]: -\frac{2}{5} \mathcal{HH}2^{mn} \sigma_1 (\nabla_a \lambda_m) (\nabla^a R[\nabla]) (\nabla_b \sigma_2) (\nabla^b \lambda_n)$$

$$T[25]: -2 \mathcal{HH}3^{mn} \sigma_1 (\nabla_a \lambda_m) (\nabla^a R[\nabla]) (\nabla_b \sigma_2) (\nabla^b \lambda_n)$$

$$T[26]: \mathcal{HH}4^{mn} \sigma_1 (\nabla_a \lambda_m) (\nabla^a R[\nabla]) (\nabla_b \sigma_2) (\nabla^b \lambda_n)$$

$$T[27]: -2 \mathcal{HH}5^{mn} \sigma_1 (\nabla_a \lambda_m) (\nabla^a R[\nabla]) (\nabla_b \sigma_2) (\nabla^b \lambda_n)$$

$$T[28]: \frac{2}{5} \mathcal{HH}6^{mn} \sigma_1 (\nabla_a \lambda_m) (\nabla^a R[\nabla]) (\nabla_b \sigma_2) (\nabla^b \lambda_n)$$

$$T[29]: 2 \mathcal{FF}^{mn} \sigma_1 (\nabla_a \lambda_m) (\nabla^a R[\nabla]) (\nabla_b \sigma_2) (\nabla^b \lambda_n)$$

$$T[30]: \frac{1}{4} \mathcal{FFP}^{mn} \sigma_1 (\nabla_a \beta_n) (\nabla^a R[\nabla]) (\nabla_b \sigma_2) (\nabla^b \lambda_m) + \mathcal{FFP}^{mn} \sigma_1 (\nabla_a \lambda_n) (\nabla^a R[\nabla]) (\nabla_b \sigma_2) (\nabla^b \lambda_m) +$$

$$\frac{1}{4} \beta^m \sigma_1 (\nabla_a \mathcal{FFP}^n_m) (\nabla^a R[\nabla]) (\nabla_b \sigma_2) (\nabla^b \lambda_n) + \frac{1}{4} \mathcal{FFP}^{mn} \beta_n \sigma_1 (\nabla_a \nabla_b \lambda_m) (\nabla^a R[\nabla]) (\nabla^b \sigma_2)$$

$$T[32]:$$

$$\frac{1}{5} \beta^m \sigma_1 (\nabla_a \lambda_n) (\nabla^a R[\nabla]) (\nabla_b \sigma_2) (\nabla^b \varepsilon\hat{\varepsilon}^n_m) - \frac{1}{5} \varepsilon\hat{\varepsilon}^{mn} \sigma_1 (\nabla_a \lambda_m) (\nabla^a R[\nabla]) (\nabla_b \sigma_2) (\nabla^b \beta_n) -$$

$$\frac{4}{5} \varepsilon\hat{\varepsilon}^{mn} \sigma_1 (\nabla_a \lambda_m) (\nabla^a R[\nabla]) (\nabla_b \sigma_2) (\nabla^b \lambda_n) + \frac{1}{5} \varepsilon\hat{\varepsilon}^{mn} \beta_n \sigma_1 (\nabla^a R[\nabla]) (\nabla_b \nabla_a \lambda_m) (\nabla^b \sigma_2)$$

$$T[33]: -\frac{1}{5} \varepsilon\hat{\varepsilon}^n_m{}^p \beta^m \sigma_1 (\nabla_a \lambda_n) (\nabla^a R[\nabla]) (\nabla_b \sigma_2) (\nabla^b \lambda_p)$$

$$T[34]: -\frac{1}{2} \mathcal{DDD}^{mnp} \beta_p \sigma_1 (\nabla_a \lambda_m) (\nabla^a R[\nabla]) (\nabla_b \sigma_2) (\nabla^b \lambda_n)$$

$$T[42]: -\frac{2}{5} \sigma_1 (\nabla_a \beta_m) (\nabla^a R[\nabla]) (\nabla_b \sigma_2) (\nabla^b \mathcal{B}^m) - \frac{4}{5} \sigma_1 (\nabla_a \lambda_m) (\nabla^a R[\nabla]) (\nabla_b \sigma_2) (\nabla^b \mathcal{B}^m) +$$

$$\frac{2}{5} \sigma_1 (\nabla_a \mathcal{B}^m) (\nabla^a R[\nabla]) (\nabla_b \sigma_2) (\nabla^b \beta_m) + \frac{2}{5} \mathcal{B}^m \sigma_1 (\nabla_a \nabla_b \beta_m) (\nabla^a R[\nabla]) (\nabla^b \sigma_2) +$$

$$\frac{4}{5} \mathcal{B}^m \sigma_1 (\nabla_a \nabla_b \lambda_m) (\nabla^a R[\nabla]) (\nabla^b \sigma_2) + \frac{2}{5} \beta^m \sigma_1 (\nabla^a R[\nabla]) (\nabla_b \nabla_a \mathcal{B}_m) (\nabla^b \sigma_2)$$

$$T[44]: \frac{1}{5} \mathcal{BBhatp}_m{}^n \beta^m \sigma_1 (\nabla_a \nabla_b \lambda_n) (\nabla^a R[\nabla]) (\nabla^b \sigma_2)$$

$$\mathbf{T}[46]: \frac{1}{10} \mathcal{B}\mathcal{B}\mathcal{B}\mathbf{p}^{\mathbf{np}}_{\mathbf{m}} \beta^{\mathbf{m}} \sigma 1 \left( \nabla_{\mathbf{a}} \lambda_{\mathbf{n}} \right) \left( \nabla^{\mathbf{a}} \mathbf{R}[\nabla] \right) \left( \nabla_{\mathbf{b}} \sigma 2 \right) \left( \nabla^{\mathbf{b}} \lambda_{\mathbf{p}} \right)$$

$$\mathbf{T}[48]: -\sigma 1 \left( \nabla_{\mathbf{a}} \beta_{\mathbf{m}} \right) \left( \nabla^{\mathbf{a}} \mathbf{R}[\nabla] \right) \left( \nabla_{\mathbf{b}} \sigma 2 \right) \left( \nabla^{\mathbf{b}} \mathcal{A}^{\mathbf{m}} \right) - 2 \sigma 1 \left( \nabla_{\mathbf{a}} \lambda_{\mathbf{m}} \right) \left( \nabla^{\mathbf{a}} \mathbf{R}[\nabla] \right) \left( \nabla_{\mathbf{b}} \sigma 2 \right) \left( \nabla^{\mathbf{b}} \mathcal{A}^{\mathbf{m}} \right) + \\ \sigma 1 \left( \nabla_{\mathbf{a}} \mathcal{A}^{\mathbf{m}} \right) \left( \nabla^{\mathbf{a}} \mathbf{R}[\nabla] \right) \left( \nabla_{\mathbf{b}} \sigma 2 \right) \left( \nabla^{\mathbf{b}} \beta_{\mathbf{m}} \right) + 2 \sigma 1 \left( \nabla_{\mathbf{a}} \mathcal{A}^{\mathbf{m}} \right) \left( \nabla^{\mathbf{a}} \mathbf{R}[\nabla] \right) \left( \nabla_{\mathbf{b}} \sigma 2 \right) \left( \nabla^{\mathbf{b}} \lambda_{\mathbf{m}} \right)$$

$$\mathbf{T}[51]: -\frac{1}{2} \mathcal{A}\mathcal{A}\mathbf{hatpp}^{\mathbf{mn}} \sigma 1 \left( \nabla_{\mathbf{a}} \lambda_{\mathbf{n}} \right) \left( \nabla^{\mathbf{a}} \mathbf{R}[\nabla] \right) \left( \nabla_{\mathbf{b}} \sigma 2 \right) \left( \nabla^{\mathbf{b}} \beta_{\mathbf{m}} \right) +$$

$$\frac{1}{2} \mathcal{A}\mathcal{A}\mathbf{hatpp}^{\mathbf{mn}} \sigma 1 \left( \nabla_{\mathbf{a}} \beta_{\mathbf{m}} \right) \left( \nabla^{\mathbf{a}} \mathbf{R}[\nabla] \right) \left( \nabla_{\mathbf{b}} \sigma 2 \right) \left( \nabla^{\mathbf{b}} \lambda_{\mathbf{n}} \right) -$$

$$\beta^{\mathbf{m}} \sigma 1 \left( \nabla_{\mathbf{a}} \mathcal{A}\mathcal{A}\mathbf{hatpp}_{\mathbf{mn}} \right) \left( \nabla^{\mathbf{a}} \mathbf{R}[\nabla] \right) \left( \nabla_{\mathbf{b}} \sigma 2 \right) \left( \nabla^{\mathbf{b}} \lambda^{\mathbf{n}} \right) -$$

$$\frac{3}{2} \mathcal{A}\mathcal{A}\mathbf{hatpp}_{\mathbf{m}}^{\mathbf{n}} \beta^{\mathbf{m}} \sigma 1 \left( \nabla_{\mathbf{a}} \nabla_{\mathbf{b}} \lambda_{\mathbf{n}} \right) \left( \nabla^{\mathbf{a}} \mathbf{R}[\nabla] \right) \left( \nabla^{\mathbf{b}} \sigma 2 \right) +$$

$$\frac{1}{2} \beta^{\mathbf{m}} \sigma 1 \left( \nabla_{\mathbf{a}} \lambda^{\mathbf{n}} \right) \left( \nabla^{\mathbf{a}} \mathbf{R}[\nabla] \right) \left( \nabla_{\mathbf{b}} \mathcal{A}\mathcal{A}\mathbf{hatpp}_{\mathbf{mn}} \right) \left( \nabla^{\mathbf{b}} \sigma 2 \right) -$$

$$\frac{1}{2} \mathcal{A}\mathcal{A}\mathbf{hatpp}_{\mathbf{m}}^{\mathbf{n}} \beta^{\mathbf{m}} \sigma 1 \left( \nabla^{\mathbf{a}} \mathbf{R}[\nabla] \right) \left( \nabla_{\mathbf{b}} \nabla_{\mathbf{a}} \lambda_{\mathbf{n}} \right) \left( \nabla^{\mathbf{b}} \sigma 2 \right)$$

$$\mathbf{Z}[20]: \frac{1}{5} \varepsilon \varepsilon^{\mathbf{mn}} \sigma 1 \left( \nabla_{\mathbf{a}} \lambda_{\mathbf{n}} \right) \left( \nabla^{\mathbf{a}} \mathbf{R}[\nabla] \right) \left( \nabla_{\mathbf{b}} \sigma 2 \right) \left( \nabla^{\mathbf{b}} \beta_{\mathbf{m}} \right) +$$

$$\frac{1}{5} \varepsilon \varepsilon^{\mathbf{mn}} \sigma 1 \left( \nabla_{\mathbf{a}} \beta_{\mathbf{n}} \right) \left( \nabla^{\mathbf{a}} \mathbf{R}[\nabla] \right) \left( \nabla_{\mathbf{b}} \sigma 2 \right) \left( \nabla^{\mathbf{b}} \lambda_{\mathbf{m}} \right) + \frac{1}{5} \beta^{\mathbf{m}} \sigma 1 \partial_{\mathbf{m}} \varepsilon \varepsilon^{\mathbf{no}} \left( \nabla_{\mathbf{a}} \lambda_{\mathbf{o}} \right) \left( \nabla^{\mathbf{a}} \mathbf{R}[\nabla] \right) \left( \nabla_{\mathbf{b}} \sigma 2 \right) \left( \nabla^{\mathbf{b}} \lambda_{\mathbf{n}} \right)$$

■ 27)  $(\sigma_1 \partial_\mu \sigma_2 - \sigma_2 \partial_\mu \sigma_1) R \partial^\mu R$

$$T[5]: \frac{5}{2} R[\nabla] \ b1 \ \sigma1 \ (\nabla_a \sigma2) \ (\nabla^a R[\nabla])$$

$$T[6]: \frac{23}{10} R[\nabla] \ b2 \ \sigma1 \ (\nabla_a \sigma2) \ (\nabla^a R[\nabla])$$

$$T[7]: \frac{47}{20} R[\nabla] \ b3 \ \sigma1 \ (\nabla_a \sigma2) \ (\nabla^a R[\nabla])$$

$$T[8]: -\frac{1}{5} R[\nabla] \ b4 \ \sigma1 \ (\nabla_a \sigma2) \ (\nabla^a R[\nabla])$$

$$T[9]: 2 R[\nabla] \ b5 \ \sigma1 \ (\nabla_a \sigma2) \ (\nabla^a R[\nabla])$$

$$T[11]: -20 R[\nabla] \ b7 \ \sigma1 \ (\nabla_a \sigma2) \ (\nabla^a R[\nabla])$$

$$T[12]: 8 R[\nabla] \ I1^m \ \beta_m \ \sigma1 \ (\nabla_a \sigma2) \ (\nabla^a R[\nabla])$$

$$T[13]: \frac{24}{5} R[\nabla] \ I2^m \ \beta_m \ \sigma1 \ (\nabla_a \sigma2) \ (\nabla^a R[\nabla])$$

$$T[14]: -\frac{1}{25} R[\nabla] \ I3^m \ \beta_m \ \sigma1 \ (\nabla_a \sigma2) \ (\nabla^a R[\nabla])$$

$$T[16]: \frac{12}{5} R[\nabla] \ I5^m \ \beta_m \ \sigma1 \ (\nabla_a \sigma2) \ (\nabla^a R[\nabla])$$

$$Z[1]: 8 R[\nabla] \ \beta^y \ \sigma1 \ \partial_y b8 \ (\nabla_a \sigma2) \ (\nabla^a R[\nabla])$$

$$Z[2]: \frac{24}{5} R[\nabla] \ \beta^y \ \sigma1 \ \partial_y b9 \ (\nabla_a \sigma2) \ (\nabla^a R[\nabla])$$

$$Z[3]: -\frac{1}{25} R[\nabla] \ \beta^y \ \sigma1 \ \partial_y b10 \ (\nabla_a \sigma2) \ (\nabla^a R[\nabla])$$

$$Z[5]: \frac{12}{5} R[\nabla] \ \beta^y \ \sigma1 \ \partial_y b12 \ (\nabla_a \sigma2) \ (\nabla^a R[\nabla])$$

■ 28)  $(\sigma_1 \partial_\mu \sigma_2 - \sigma_2 \partial_\mu \sigma_1) \nabla^2 R$

$$T[10]: \sigma1 \ (\nabla_a \sigma2) \ (\nabla^a b6) \ (\nabla_b \nabla^b R[\nabla])$$

$$T[15]: \frac{4}{5} I4^m \ \sigma1 \ (\nabla_a \sigma2) \ (\nabla^a \lambda_m) \ (\nabla_b \nabla^b R[\nabla])$$

$$T[22]: -\frac{1}{5} \mathcal{G}4_m^n \ \beta^m \ \sigma1 \ (\nabla_a \sigma2) \ (\nabla^a \lambda_n) \ (\nabla_b \nabla^b R[\nabla])$$

$$T[42]: \frac{1}{5} \beta^m \ \sigma1 \ (\nabla_a \sigma2) \ (\nabla^a \beta_m) \ (\nabla_b \nabla^b R[\nabla]) + \frac{1}{5} \beta^m \ \sigma1 \ (\nabla_a \sigma2) \ (\nabla^a \beta_m) \ (\nabla_b \nabla^b R[\nabla])$$

$$Z[11]: \frac{1}{5} \mathcal{G}4^m \ \sigma1 \ (\nabla_a \sigma2) \ (\nabla^a \beta_m) \ (\nabla_b \nabla^b R[\nabla]) + \frac{1}{5} \beta^m \ \sigma1 \ \partial_m \mathcal{G}4^y \ (\nabla_a \sigma2) \ (\nabla^a \lambda_y) \ (\nabla_b \nabla^b R[\nabla])$$

■ **29)  $(\sigma_1 \partial_\mu \sigma_2 - \sigma_2 \partial_\mu \sigma_1) \partial^\mu \nabla^2 R$**

$$T[10]: b6 \sigma_1 (\nabla_a \nabla_b \nabla^b R[\nabla]) (\nabla^a \sigma_2)$$

$$T[11]: -4 b7 \sigma_1 (\nabla_a \nabla_b \nabla^b R[\nabla]) (\nabla^a \sigma_2)$$

$$T[15]: -\frac{1}{5} \mathcal{I} 4^m \beta_m \sigma_1 (\nabla_a \nabla_b \nabla^b R[\nabla]) (\nabla^a \sigma_2)$$

$$T[42]: -\frac{1}{5} \mathcal{B}^m \beta_m \sigma_1 (\nabla_a \nabla_b \nabla^b R[\nabla]) (\nabla^a \sigma_2)$$

$$Z[4]: -\frac{1}{5} \beta^y \sigma_1 \partial_y b_{11} (\nabla_a \nabla_b \nabla^b R[\nabla]) (\nabla^a \sigma_2)$$

■ **30)  $(\sigma_1 \partial_\mu \sigma_2 - \sigma_2 \partial_\mu \sigma_1) \partial^\mu E_4$**

$$T[5]: -9 b1 \sigma_1 (\nabla_a \sigma_2) (\nabla^a E_4)$$

$$T[6]: -b2 \sigma_1 (\nabla_a \sigma_2) (\nabla^a E_4)$$

$$T[8]: -b4 \sigma_1 (\nabla_a \sigma_2) (\nabla^a E_4)$$

$$T[11]: 32 b7 \sigma_1 (\nabla_a \sigma_2) (\nabla^a E_4)$$

$$T[12]: -\mathcal{I} 1^m \beta_m \sigma_1 (\nabla_a \sigma_2) (\nabla^a E_4)$$

$$Z[1]: -\beta^y \sigma_1 \partial_y b_8 (\nabla_a \sigma_2) (\nabla^a E_4)$$

■ **31)  $(\sigma_1 \partial_\mu \sigma_2 - \sigma_2 \partial_\mu \sigma_1) \partial^\mu F$**

$$T[5]: -\frac{1}{2} b1 \sigma_1 (\nabla_a \sigma_2) (\nabla^a F)$$

$$T[6]: -\frac{1}{6} b2 \sigma_1 (\nabla_a \sigma_2) (\nabla^a F)$$

$$T[8]: -\frac{2}{3} b4 \sigma_1 (\nabla_a \sigma_2) (\nabla^a F)$$

$$T[11]: -\frac{28}{3} b7 \sigma_1 (\nabla_a \sigma_2) (\nabla^a F)$$

$$T[13]: -\mathcal{I} 2^m \beta_m \sigma_1 (\nabla_a \sigma_2) (\nabla^a F)$$

$$Z[2]: -\beta^y \sigma_1 \partial_y b_9 (\nabla_a \sigma_2) (\nabla^a F)$$

■ **32)  $(\sigma_1 \partial_\nu \sigma_2 - \sigma_2 \partial_\nu \sigma_1) H_1^{\mu\nu}$**

$$T[4]: 6 H_1^{ab} \sigma_1 (\nabla_a a) (\nabla_b \sigma_2)$$

$$T[5]: H_1^{ab} \sigma_1 (\nabla_a b_1) (\nabla_b \sigma_2)$$

$$T[7]: -\frac{1}{15} H_1^{ab} \sigma_1 (\nabla_a b_3) (\nabla_b \sigma_2)$$

$$T[23]: -H_1^{ab} \mathcal{H} H_{1m}^n \beta^m \sigma_1 (\nabla_a \lambda_n) (\nabla_b \sigma_2)$$

$$Z[12]: H_1^{ab} \mathcal{H} 1^m \sigma_1 (\nabla_a \beta_m) (\nabla_b \sigma_2) + H_1^{ab} \beta^m \sigma_1 \partial_m \mathcal{H} 1^y (\nabla_a \lambda_y) (\nabla_b \sigma_2)$$

■ **33)  $(\sigma_1 \partial_\nu \sigma_2 - \sigma_2 \partial_\nu \sigma_1) H_2^{\mu\nu}$**

$$T[5]: 30 H_2^{ab} \sigma_1 (\nabla_a b_1) (\nabla_b \sigma_2)$$

$$T[6]: 2 H_2^{ab} \sigma_1 (\nabla_a b_2) (\nabla_b \sigma_2)$$

$$T[7]: - H_2^{ab} \sigma_1 (\nabla_a b_3) (\nabla_b \sigma_2)$$

$$T[8]: 2 H_2^{ab} \sigma_1 (\nabla_a b_4) (\nabla_b \sigma_2)$$

$$T[16]: 2 H_2^{ab} I_5^m \sigma_1 (\nabla_a \lambda_m) (\nabla_b \sigma_2)$$

$$T[18]: 5 H_2^{ab} I_7^m \sigma_1 (\nabla_a \lambda_m) (\nabla_b \sigma_2)$$

$$T[24]: - H_2^{ab} \mathcal{H}H_2^m \beta^m \sigma_1 (\nabla_a \lambda_n) (\nabla_b \sigma_2)$$

$$T[37]: - \frac{5}{4} H_2^{ab} C\text{Chatp}_m^n \beta^m \sigma_1 (\nabla_a \lambda_n) (\nabla_b \sigma_2)$$

$$T[44]: H_2^{ab} \mathcal{B}\mathcal{B}\text{hatp}_m^n \beta^m \sigma_1 (\nabla_a \lambda_n) (\nabla_b \sigma_2)$$

$$Z[13]: H_2^{ab} \mathcal{H}2^m \sigma_1 (\nabla_a \beta_m) (\nabla_b \sigma_2) + H_2^{ab} \beta^m \sigma_1 \partial_m \mathcal{H}2^y (\nabla_a \lambda_y) (\nabla_b \sigma_2)$$

■ **34)  $(\sigma_1 \partial_\mu \sigma_2 - \sigma_2 \partial_\mu \sigma_1) \nabla_\nu H_2^{\mu\nu}$**

$$T[5]: 30 b_1 \sigma_1 (\nabla^a \sigma_2) (\nabla_b H_2^a{}^b)$$

$$T[6]: 2 b_2 \sigma_1 (\nabla^a \sigma_2) (\nabla_b H_2^a{}^b)$$

$$T[7]: - b_3 \sigma_1 (\nabla^a \sigma_2) (\nabla_b H_2^a{}^b)$$

$$T[8]: 2 b_4 \sigma_1 (\nabla^a \sigma_2) (\nabla_b H_2^a{}^b)$$

$$T[11]: - 80 b_7 \sigma_1 (\nabla^a \sigma_2) (\nabla_b H_2^a{}^b)$$

$$T[16]: - I_5^m \beta_m \sigma_1 (\nabla^a \sigma_2) (\nabla_b H_2^a{}^b)$$

$$Z[5]: - \beta^y \sigma_1 \partial_y b_{12} (\nabla^a \sigma_2) (\nabla_b H_2^a{}^b)$$

■ **35)  $(\sigma_1 \partial_\nu \sigma_2 - \sigma_2 \partial_\nu \sigma_1) H_3^{\mu\nu}$**

$$T[5]: - 12 H_3^{ab} \sigma_1 (\nabla_a b_1) (\nabla_b \sigma_2)$$

$$T[7]: H_3^{ab} \sigma_1 (\nabla_a b_3) (\nabla_b \sigma_2)$$

$$T[11]: - 8 H_3^{ab} \sigma_1 (\nabla_a b_7) (\nabla_b \sigma_2)$$

$$T[17]: 6 H_3^{ab} I_6^m \sigma_1 (\nabla_a \lambda_m) (\nabla_b \sigma_2)$$

$$T[18]: - 2 H_3^{ab} I_7^m \sigma_1 (\nabla_a \lambda_m) (\nabla_b \sigma_2)$$

$$T[25]: - H_3^{ab} \mathcal{H}H_3^m \beta^m \sigma_1 (\nabla_a \lambda_n) (\nabla_b \sigma_2)$$

$$T[29]: \frac{1}{2} H_3^{ab} \mathcal{F}\mathcal{F}^{mn} \beta_n \sigma_1 (\nabla_a \lambda_m) (\nabla_b \sigma_2)$$

$$T[37]: \frac{1}{2} H_3^{ab} C\text{Chatp}_m^n \beta^m \sigma_1 (\nabla_a \lambda_n) (\nabla_b \sigma_2)$$

$$T[51]: - H_3^{ab} \mathcal{A}\mathcal{A}\text{hatpp}_m^n \beta^m \sigma_1 (\nabla_a \lambda_n) (\nabla_b \sigma_2)$$

$$Z[14]: H_3^{ab} \mathcal{H}3^m \sigma_1 (\nabla_a \beta_m) (\nabla_b \sigma_2) + H_3^{ab} \beta^m \sigma_1 \partial_m \mathcal{H}3^y (\nabla_a \lambda_y) (\nabla_b \sigma_2)$$



■ **36)  $(\sigma_1 \partial_\mu \sigma_2 - \sigma_2 \partial_\mu \sigma_1) \nabla_\nu H_3^{\mu\nu}$**

$$T[5]: -12 \, b1 \, \sigma1 \, (\nabla^a \sigma2) \, (\nabla_b H3_a^b)$$

$$T[7]: b3 \, \sigma1 \, (\nabla^a \sigma2) \, (\nabla_b H3_a^b)$$

$$T[11]: 16 \, b7 \, \sigma1 \, (\nabla^a \sigma2) \, (\nabla_b H3_a^b)$$

$$T[17]: -I6^m \, \beta_m \, \sigma1 \, (\nabla^a \sigma2) \, (\nabla_b H3_a^b)$$

$$Z[6]: -\beta^y \, \sigma1 \, \partial_y b13 \, (\nabla^a \sigma2) \, (\nabla_b H3_a^b)$$

■ **37)  $(\sigma_1 \partial_\nu \sigma_2 - \sigma_2 \partial_\nu \sigma_1) H_4^{\mu\nu}$**

$$T[5]: -12 \, H4^{ab} \, \sigma1 \, (\nabla_a b1) \, (\nabla_b \sigma2)$$

$$T[11]: 8 \, H4^{ab} \, \sigma1 \, (\nabla_a b7) \, (\nabla_b \sigma2)$$

$$T[18]: -2 \, H4^{ab} \, I7^m \, \sigma1 \, (\nabla_a \lambda_m) \, (\nabla_b \sigma2)$$

$$T[26]: -H4^{ab} \, \mathcal{H}H4_m^n \, \beta^m \, \sigma1 \, (\nabla_a \lambda_n) \, (\nabla_b \sigma2)$$

$$T[29]: -\frac{1}{2} \, H4^{ab} \, \mathcal{F}F^{mn} \, \beta_n \, \sigma1 \, (\nabla_a \lambda_m) \, (\nabla_b \sigma2)$$

$$Z[15]: H4^{ab} \, \mathcal{H}4^m \, \sigma1 \, (\nabla_a \beta_m) \, (\nabla_b \sigma2) + H4^{ab} \, \beta^m \, \sigma1 \, \partial_m \mathcal{H}4^y \, (\nabla_a \lambda_y) \, (\nabla_b \sigma2)$$

■ **38)  $(\sigma_1 \partial_\mu \sigma_2 - \sigma_2 \partial_\mu \sigma_1) \nabla_\nu H_4^{\mu\nu}$**

$$T[5]: -12 \, b1 \, \sigma1 \, (\nabla^a \sigma2) \, (\nabla_b H4_a^b)$$

$$T[11]: 32 \, b7 \, \sigma1 \, (\nabla^a \sigma2) \, (\nabla_b H4_a^b)$$

$$T[18]: -I7^m \, \beta_m \, \sigma1 \, (\nabla^a \sigma2) \, (\nabla_b H4_a^b)$$

$$Z[7]: -\beta^y \, \sigma1 \, \partial_y b14 \, (\nabla^a \sigma2) \, (\nabla_b H4_a^b)$$

■ **39)  $(\sigma_1 \partial_\nu \sigma_2 - \sigma_2 \partial_\nu \sigma_1) H_5^{\mu\nu}$**

$$T[11]: -8 \, H5^{ab} \, \sigma1 \, (\nabla_a b7) \, (\nabla_b \sigma2)$$

$$T[27]: -H5^{ab} \, \mathcal{H}H5_m^n \, \beta^m \, \sigma1 \, (\nabla_a \lambda_n) \, (\nabla_b \sigma2)$$

$$T[30]: \frac{1}{2} \, H5^{ab} \, \mathcal{F}F^{mn} \, \beta_n \, \sigma1 \, (\nabla_a \lambda_m) \, (\nabla_b \sigma2)$$

$$T[51]: -H5^{ab} \, \mathcal{A}A^{pp}_m^n \, \beta^m \, \sigma1 \, (\nabla_a \lambda_n) \, (\nabla_b \sigma2)$$

$$Z[16]: H5^{ab} \, \mathcal{H}5^m \, \sigma1 \, (\nabla_a \beta_m) \, (\nabla_b \sigma2) + H5^{ab} \, \beta^m \, \sigma1 \, \partial_m \mathcal{H}5^y \, (\nabla_a \lambda_y) \, (\nabla_b \sigma2)$$

■ 40)  $(\sigma_1 \partial_\nu \sigma_2 - \sigma_2 \partial_\nu \sigma_1) H_6^{\mu\nu}$ 

$$T[10]: 5 H_6^{ab} \sigma_1 (\nabla_a b_6) (\nabla_b \sigma_2)$$

$$T[11]: -20 H_6^{ab} \sigma_1 (\nabla_a b_7) (\nabla_b \sigma_2)$$

$$T[28]: -H_6^{ab} \mathcal{H} \mathcal{H} 6_m^n \beta^m \sigma_1 (\nabla_a \lambda_n) (\nabla_b \sigma_2)$$

$$T[30]: -\frac{5}{4} H_6^{ab} \mathcal{F} \mathcal{F} \mathcal{P}^{mn} \beta_n \sigma_1 (\nabla_a \lambda_m) (\nabla_b \sigma_2)$$

$$T[32]: H_6^{ab} \mathcal{E} \mathcal{E} \text{hat}^{mn} \beta_n \sigma_1 (\nabla_a \lambda_m) (\nabla_b \sigma_2)$$

$$T[42]: 2 H_6^{ab} \beta^m \sigma_1 (\nabla_a \mathcal{B}_m) (\nabla_b \sigma_2) - 2 H_6^{ab} \mathcal{B}^m \sigma_1 (\nabla_a \beta_m) (\nabla_b \sigma_2) - 4 H_6^{ab} \mathcal{B}^m \sigma_1 (\nabla_a \lambda_m) (\nabla_b \sigma_2)$$

$$Z[17]: H_6^{ab} \mathcal{H} 6^m \sigma_1 (\nabla_a \beta_m) (\nabla_b \sigma_2) + H_6^{ab} \beta^m \sigma_1 \partial_m \mathcal{H} 6^y (\nabla_a \lambda_y) (\nabla_b \sigma_2)$$

■ 41)  $\sigma_1 \partial_\mu \sigma_2 - \sigma_2 \partial_\mu \sigma_1$ 

$$T[15]: 2 I_4^m \sigma_1 (\nabla_a \nabla_c \nabla^c \nabla_b \nabla^b \lambda_m) (\nabla^a \sigma_2) + 2 \sigma_1 (\nabla_a \nabla_c \nabla^c \lambda_m) (\nabla^a \sigma_2) (\nabla_b \nabla^b I_4^m) + \\ 2 \sigma_1 (\nabla_a \nabla_c \nabla^c I_4^m) (\nabla^a \sigma_2) (\nabla_b \nabla^b \lambda^m) + 2 \sigma_1 (\nabla_a \nabla^b \lambda^m) (\nabla^a \sigma_2) (\nabla_b \nabla_c \nabla^c I_4^m) + \\ 6 \sigma_1 (\nabla_a \nabla^b I_4^m) (\nabla^a \sigma_2) (\nabla_b \nabla_c \nabla^c \lambda_m) + 2 \sigma_1 (\nabla^a \lambda^m) (\nabla_b \nabla_a \nabla_c \nabla^c I_4^m) (\nabla^b \sigma_2) + \\ 6 \sigma_1 (\nabla^a I_4^m) (\nabla_b \nabla_a \nabla_c \nabla^c \lambda_m) (\nabla^b \sigma_2) + 2 \sigma_1 (\nabla_a \sigma_2) (\nabla^a I_4^m) (\nabla_c \nabla^c \nabla_b \nabla^b \lambda_m) + \\ 4 \sigma_1 (\nabla_a \nabla_c \nabla_b \lambda_m) (\nabla^a \sigma_2) (\nabla^c \nabla^b I_4^m) + 4 \sigma_1 (\nabla_a \nabla_c \nabla_b I_4^m) (\nabla^a \sigma_2) (\nabla^c \nabla^b \lambda^m)$$

$$T[22]: -2 \mathcal{G} \mathcal{G} 4^{mn} \sigma_1 (\nabla_a \nabla^b \lambda_m) (\nabla^a \sigma_2) (\nabla_b \nabla_c \nabla^c \lambda_n) - 4 \sigma_1 (\nabla_a \nabla^c \lambda_m) (\nabla^a \sigma_2) (\nabla_b \nabla_c \lambda_n) (\nabla^b \mathcal{G} \mathcal{G} 4^{mn}) - \\ 2 \sigma_1 (\nabla_a \nabla_c \nabla^c \lambda_n) (\nabla^a \lambda^m) (\nabla_b \mathcal{G} \mathcal{G} 4_m^n) (\nabla^b \sigma_2) - 2 \mathcal{G} \mathcal{G} 4^{mn} \sigma_1 (\nabla^a \lambda_m) (\nabla_b \nabla_a \nabla_c \nabla^c \lambda_n) (\nabla^b \sigma_2) - \\ \sigma_1 (\nabla_a \lambda^n) (\nabla^a \lambda^m) (\nabla_b \nabla_c \nabla^c \mathcal{G} \mathcal{G} 4_{mn}) (\nabla^b \sigma_2) - 2 \sigma_1 (\nabla^a \lambda^m) (\nabla_b \nabla_a \lambda^n) (\nabla^b \sigma_2) (\nabla_c \nabla^c \mathcal{G} \mathcal{G} 4_{mn}) - \\ 4 \sigma_1 (\nabla^a \lambda^m) (\nabla_b \nabla_c \nabla_a \lambda_n) (\nabla^b \sigma_2) (\nabla^c \mathcal{G} \mathcal{G} 4_m^n) - 4 \sigma_1 (\nabla^a \lambda^m) (\nabla_b \nabla_c \mathcal{G} \mathcal{G} 4_{mn}) (\nabla^b \sigma_2) (\nabla^c \nabla_a \lambda^n) - \\ 4 \mathcal{G} \mathcal{G} 4^{mn} \sigma_1 (\nabla_a \nabla_c \nabla_b \lambda_n) (\nabla^a \sigma_2) (\nabla^c \nabla^b \lambda_m) - 2 \sigma_1 (\nabla_a \mathcal{G} \mathcal{G} 4^{mn}) (\nabla^a \sigma_2) (\nabla_c \nabla_b \lambda_n) (\nabla^c \nabla^b \lambda_m)$$

$$T[27]: -\mathcal{H} \mathcal{H} 5^{mn} \sigma_1 (\nabla_a \nabla^b \lambda_m) (\nabla^a \sigma_2) (\nabla_b \nabla_c \nabla^c \lambda_n) - 12 \sigma_1 (\nabla_a \sigma_2) (\nabla^a \lambda^m) (\nabla_b \nabla_c \nabla^c \lambda_n) (\nabla^b \mathcal{H} \mathcal{H} 5_m^n) - \\ 2 \sigma_1 (\nabla_a \nabla^c \lambda_m) (\nabla^a \sigma_2) (\nabla_b \nabla_c \lambda_n) (\nabla^b \mathcal{H} \mathcal{H} 5^{mn}) - 2 \sigma_1 (\nabla_a \sigma_2) (\nabla^a \lambda^m) (\nabla_b \nabla_c \nabla^c \mathcal{H} \mathcal{H} 5_{mn}) (\nabla^b \lambda^n) - \\ \sigma_1 (\nabla_a \nabla_c \nabla^c \lambda_n) (\nabla^a \lambda^m) (\nabla_b \mathcal{H} \mathcal{H} 5_m^n) (\nabla^b \sigma_2) - \mathcal{H} \mathcal{H} 5^{mn} \sigma_1 (\nabla^a \lambda_m) (\nabla_b \nabla_a \nabla_c \nabla^c \lambda_n) (\nabla^b \sigma_2) - \\ \frac{1}{2} \sigma_1 (\nabla_a \lambda^n) (\nabla^a \lambda^m) (\nabla_b \nabla_c \nabla^c \mathcal{H} \mathcal{H} 5_{mn}) (\nabla^b \sigma_2) - 8 \mathcal{H} \mathcal{H} 5^{mn} \sigma_1 (\nabla^a \sigma_2) (\nabla_b \nabla_c \nabla^c \lambda_n) (\nabla^b \nabla_a \lambda_m) - \\ 2 \sigma_1 (\nabla_a \sigma_2) (\nabla^a \lambda^m) (\nabla_b \nabla^b \lambda^n) (\nabla_c \nabla^c \mathcal{H} \mathcal{H} 5_{mn}) - 2 \sigma_1 (\nabla_a \nabla_b \lambda^n) (\nabla^a \lambda^m) (\nabla^b \sigma_2) (\nabla_c \nabla^c \mathcal{H} \mathcal{H} 5_{mn}) - \\ \sigma_1 (\nabla^a \lambda^m) (\nabla_b \nabla_a \lambda^n) (\nabla^b \sigma_2) (\nabla_c \nabla^c \mathcal{H} \mathcal{H} 5_{mn}) - 4 \mathcal{H} \mathcal{H} 5^{mn} \sigma_1 (\nabla_a \sigma_2) (\nabla^a \lambda_m) (\nabla_c \nabla^c \nabla_b \nabla^b \lambda_n) - \\ 2 \sigma_1 (\nabla^a \lambda^m) (\nabla_b \nabla_c \nabla_a \lambda_n) (\nabla^b \sigma_2) (\nabla^c \mathcal{H} \mathcal{H} 5_m^n) - 8 \sigma_1 (\nabla^a \sigma_2) (\nabla_b \nabla_c \lambda_n) (\nabla^b \mathcal{H} \mathcal{H} 5^{mn}) (\nabla^c \nabla_a \lambda_m) - \\ 4 \sigma_1 (\nabla^a \sigma_2) (\nabla^b \mathcal{H} \mathcal{H} 5^{mn}) (\nabla_c \nabla_b \lambda_n) (\nabla^c \nabla_a \lambda_m) - 2 \sigma_1 (\nabla^a \lambda^m) (\nabla_b \nabla_c \mathcal{H} \mathcal{H} 5_{mn}) (\nabla^b \sigma_2) (\nabla^c \nabla_a \lambda^n) - \\ 2 \mathcal{H} \mathcal{H} 5^{mn} \sigma_1 (\nabla_a \nabla_c \nabla_b \lambda_n) (\nabla^a \sigma_2) (\nabla^c \nabla^b \lambda_m) - 4 \mathcal{H} \mathcal{H} 5^{mn} \sigma_1 (\nabla^a \sigma_2) (\nabla_b \nabla_c \nabla_a \lambda_n) (\nabla^c \nabla^b \lambda_m) - \\ \sigma_1 (\nabla_a \mathcal{H} \mathcal{H} 5^{mn}) (\nabla^a \sigma_2) (\nabla_c \nabla_b \lambda_n) (\nabla^c \nabla^b \lambda_m) - 8 \sigma_1 (\nabla_a \sigma_2) (\nabla^a \lambda^m) (\nabla_b \nabla_c \mathcal{H} \mathcal{H} 5_{mn}) (\nabla^c \nabla^b \lambda^n)$$

$$T[28]: -2 \mathcal{H} \mathcal{H} 6^{mn} \sigma_1 (\nabla_a \nabla_c \nabla^c \lambda_n) (\nabla^a \sigma_2) (\nabla_b \nabla^b \lambda_m) - 2 \mathcal{H} \mathcal{H} 6^{mn} \sigma_1 (\nabla_a \nabla^b \lambda_m) (\nabla^a \sigma_2) (\nabla_b \nabla_c \nabla^c \lambda_n) - \\ 2 \sigma_1 (\nabla_a \nabla_c \nabla^c \lambda_n) (\nabla^a \lambda^m) (\nabla_b \mathcal{H} \mathcal{H} 6_m^n) (\nabla^b \sigma_2) - 2 \mathcal{H} \mathcal{H} 6^{mn} \sigma_1 (\nabla^a \lambda_m) (\nabla_b \nabla_a \nabla_c \nabla^c \lambda_n) (\nabla^b \sigma_2) - \\ 2 \sigma_1 (\nabla_a \nabla^c \lambda^n) (\nabla^a \lambda^m) (\nabla_b \nabla_c \mathcal{H} \mathcal{H} 6_{mn}) (\nabla^b \sigma_2) - 2 \sigma_1 (\nabla_a \mathcal{H} \mathcal{H} 6_m^n) (\nabla^a \lambda^m) (\nabla_b \nabla_c \nabla^c \lambda_n) (\nabla^b \sigma_2) - \\ \sigma_1 (\nabla_a \nabla_c \mathcal{H} \mathcal{H} 6_{mn}) (\nabla^a \lambda^m) (\nabla_b \nabla^c \lambda^n) (\nabla^b \sigma_2) - \sigma_1 (\nabla^a \lambda^m) (\nabla_b \nabla^c \lambda^n) (\nabla^b \sigma_2) (\nabla_c \nabla_a \mathcal{H} \mathcal{H} 6_{mn}) - \\ \sigma_1 (\nabla_a \mathcal{H} \mathcal{H} 6^{mn}) (\nabla^a \sigma_2) (\nabla_b \nabla^b \lambda_m) (\nabla_c \nabla^c \lambda_n) - 2 \sigma_1 (\nabla_a \nabla_b \lambda_m) (\nabla^a \sigma_2) (\nabla^b \mathcal{H} \mathcal{H} 6^{mn}) (\nabla_c \nabla^c \lambda_n) - \\ 2 \sigma_1 (\nabla^a \lambda^m) (\nabla_b \nabla_a \mathcal{H} \mathcal{H} 6_{mn}) (\nabla^b \sigma_2) (\nabla_c \nabla^c \lambda^n) - 2 \sigma_1 (\nabla^a \lambda^m) (\nabla_b \nabla_a \nabla_c \lambda_n) (\nabla^b \sigma_2) (\nabla^c \mathcal{H} \mathcal{H} 6_m^n) - \\ \sigma_1 (\nabla^a \lambda^m) (\nabla^b \lambda^n) (\nabla_c \nabla_b \nabla_a \mathcal{H} \mathcal{H} 6_{mn}) (\nabla^c \sigma_2) - 2 \sigma_1 (\nabla_a \nabla_c \lambda_n) (\nabla^a \sigma_2) (\nabla^b \mathcal{H} \mathcal{H} 6^{mn}) (\nabla^c \nabla_b \lambda_m) - \\ 2 \mathcal{H} \mathcal{H} 6^{mn} \sigma_1 (\nabla_a \nabla_b \nabla_c \lambda_n) (\nabla^a \sigma_2) (\nabla^c \nabla^b \lambda_m) - \sigma_1 (\nabla_a \mathcal{H} \mathcal{H} 6^{mn}) (\nabla^a \sigma_2) (\nabla_b \nabla_c \lambda_n) (\nabla^c \nabla^b \lambda_m)$$



$$\begin{aligned}
& \text{T}[32]: 2 \, \varepsilon\varepsilon\text{hat}^{\text{mn}} \, \sigma_1 (\nabla_a \nabla_c \nabla^c \lambda_n) (\nabla^a \sigma_2) (\nabla_b \nabla^b \lambda_m) + \\
& 2 \, \varepsilon\varepsilon\text{hat}^{\text{mn}} \, \sigma_1 (\nabla_a \nabla_c \nabla^c \lambda_m) (\nabla^a \sigma_2) (\nabla_b \nabla^b \lambda_n) + 2 \, \varepsilon\varepsilon\text{hat}^{\text{mn}} \, \sigma_1 (\nabla_a \nabla^b \lambda_m) (\nabla^a \sigma_2) (\nabla_b \nabla_c \nabla^c \lambda_n) + \\
& 2 \, \sigma_1 (\nabla_a \sigma_2) (\nabla^a \varepsilon\varepsilon\text{hat}^{\text{mn}}) (\nabla_b \nabla_c \nabla^c \lambda_n) (\nabla^b \lambda_m) + 2 \, \varepsilon\varepsilon\text{hat}^{\text{mn}} \, \sigma_1 (\nabla^a \lambda_m) (\nabla_b \nabla_a \nabla_c \nabla^c \lambda_n) (\nabla^b \sigma_2) + \\
& 2 \, \sigma_1 (\nabla_a \lambda_m) (\nabla^a \varepsilon\varepsilon\text{hat}^{\text{mn}}) (\nabla_b \nabla_c \nabla^c \lambda_n) (\nabla^b \sigma_2) + 2 \, \sigma_1 (\nabla_a \sigma_2) (\nabla^a \varepsilon\varepsilon\text{hat}^{\text{mn}}) (\nabla_b \nabla^b \lambda_m) (\nabla_c \nabla^c \lambda_n) + \\
& 2 \, \sigma_1 (\nabla^a \lambda^m) (\nabla_b \nabla_a \varepsilon\varepsilon\text{hat}_m^n) (\nabla^b \sigma_2) (\nabla_c \nabla^c \lambda_n) + 2 \, \sigma_1 (\nabla^a \varepsilon\varepsilon\text{hat}^{\text{mn}}) (\nabla_b \nabla_a \lambda_m) (\nabla^b \sigma_2) (\nabla_c \nabla^c \lambda_n) \\
\\
& \text{T}[33]: \\
& 2 \, \varepsilon\varepsilon\varepsilon^{\text{mnp}} \, \sigma_1 (\nabla_a \nabla^c \lambda_n) (\nabla^a \lambda_m) (\nabla_b \nabla_c \lambda_p) (\nabla^b \sigma_2) + \varepsilon\varepsilon\varepsilon^{\text{mnp}} \, \sigma_1 (\nabla_a \lambda_p) (\nabla^a \lambda_n) (\nabla_b \nabla_c \nabla^c \lambda_m) (\nabla^b \sigma_2) + \\
& 2 \, \varepsilon\varepsilon\varepsilon^{\text{mnp}} \, \sigma_1 (\nabla^a \lambda_n) (\nabla_b \nabla^c \lambda_m) (\nabla^b \sigma_2) (\nabla_c \nabla_a \lambda_p) + \\
& 2 \, \varepsilon\varepsilon\varepsilon^{\text{mnp}} \, \sigma_1 (\nabla^a \lambda_n) (\nabla_b \nabla_a \lambda_p) (\nabla^b \sigma_2) (\nabla_c \nabla^c \lambda_m) + \\
& \sigma_1 (\nabla_a \lambda^n) (\nabla^a \lambda^m) (\nabla_b \varepsilon\varepsilon\varepsilon_{mn}^p) (\nabla^b \sigma_2) (\nabla_c \nabla^c \lambda_p) + \\
& \sigma_1 (\nabla_a \lambda^n) (\nabla^a \lambda^m) (\nabla_b \nabla_c \lambda_p) (\nabla^b \sigma_2) (\nabla^c \varepsilon\varepsilon\varepsilon_{mn}^p) + \\
& 2 \, \sigma_1 (\nabla_a \nabla_b \lambda_p) (\nabla^a \lambda^m) (\nabla^b \lambda^n) (\nabla_c \varepsilon\varepsilon\varepsilon_{mn}^p) (\nabla^c \sigma_2) + \\
& 2 \, \varepsilon\varepsilon\varepsilon^{\text{mnp}} \, \sigma_1 (\nabla^a \lambda_m) (\nabla^b \lambda_n) (\nabla_c \nabla_a \nabla_b \lambda_p) (\nabla^c \sigma_2) + \\
& \sigma_1 (\nabla_a \lambda^n) (\nabla^a \lambda^m) (\nabla^b \lambda^p) (\nabla_c \nabla_b \varepsilon\varepsilon\varepsilon_{pmn}) (\nabla^c \sigma_2) + \\
& 2 \, \sigma_1 (\nabla_a \varepsilon\varepsilon\varepsilon_{mn}^p) (\nabla^a \lambda^m) (\nabla^b \lambda^n) (\nabla_c \nabla_b \lambda_p) (\nabla^c \sigma_2) \\
\\
& \text{T}[34]: \mathcal{DDD}^{\text{mnp}} \, \sigma_1 (\nabla_a \nabla_c \nabla^c \lambda_p) (\nabla^a \lambda_m) (\nabla_b \sigma_2) (\nabla^b \lambda_n) - \\
& \mathcal{DDD}^{\text{mnp}} \, \sigma_1 (\nabla_a \lambda_n) (\nabla^a \lambda_m) (\nabla_b \nabla_c \nabla^c \lambda_p) (\nabla^b \sigma_2) - \mathcal{DDD}^{\text{mnp}} \, \sigma_1 (\nabla_a \sigma_2) (\nabla^a \lambda_m) (\nabla_b \nabla^b \lambda_n) (\nabla_c \nabla^c \lambda_p) - \\
& \sigma_1 (\nabla_a \lambda_n) (\nabla^a \mathcal{DDD}^{\text{mnp}}) (\nabla_b \sigma_2) (\nabla^b \lambda_m) (\nabla_c \nabla^c \lambda_p) - \\
& \mathcal{DDD}^{\text{mnp}} \, \sigma_1 (\nabla_a \nabla_b \lambda_m) (\nabla^a \lambda_n) (\nabla^b \sigma_2) (\nabla_c \nabla^c \lambda_p) + \\
& \sigma_1 (\nabla_a \nabla_b \lambda_p) (\nabla^a \mathcal{DDD}^{\text{mnp}}) (\nabla^b \lambda_m) (\nabla_c \sigma_2) (\nabla^c \lambda_n) + \\
& \sigma_1 (\nabla^a \mathcal{DDD}^{\text{mnp}}) (\nabla_b \sigma_2) (\nabla^b \lambda_m) (\nabla_c \nabla_a \lambda_p) (\nabla^c \lambda_n) - \\
& \sigma_1 (\nabla_a \nabla_c \lambda_p) (\nabla^a \mathcal{DDD}^{\text{mnp}}) (\nabla_b \lambda_n) (\nabla^b \lambda_m) (\nabla^c \sigma_2) - \\
& \mathcal{DDD}^{\text{mnp}} \, \sigma_1 (\nabla^a \lambda_n) (\nabla^b \sigma_2) (\nabla_c \nabla_b \lambda_p) (\nabla^c \nabla_a \lambda_m) - \mathcal{DDD}^{\text{mnp}} \, \sigma_1 (\nabla^a \lambda_m) (\nabla^b \sigma_2) (\nabla_c \nabla_b \lambda_p) (\nabla^c \nabla_a \lambda_n) + \\
& \mathcal{DDD}^{\text{mnp}} \, \sigma_1 (\nabla_a \nabla_c \lambda_p) (\nabla^a \lambda_n) (\nabla^b \sigma_2) (\nabla^c \nabla_b \lambda_m) + \mathcal{DDD}^{\text{mnp}} \, \sigma_1 (\nabla^a \lambda_m) (\nabla^b \sigma_2) (\nabla_c \nabla_a \lambda_p) (\nabla^c \nabla_b \lambda_n) + \\
& \mathcal{DDD}^{\text{mnp}} \, \sigma_1 (\nabla_a \sigma_2) (\nabla^a \lambda_n) (\nabla_c \nabla_b \lambda_p) (\nabla^c \nabla^b \lambda_m) + \mathcal{DDD}^{\text{mnp}} \, \sigma_1 (\nabla_a \sigma_2) (\nabla^a \lambda_m) (\nabla_b \nabla_c \lambda_p) (\nabla^c \nabla^b \lambda_n) \\
\\
& \text{T}[35]: - \mathcal{DDDD}^{\text{mnop}} \, \sigma_1 (\nabla_a \lambda_o) (\nabla^a \lambda_m) (\nabla_b \sigma_2) (\nabla^b \lambda_n) (\nabla_c \nabla^c \lambda_p) + \\
& \mathcal{DDDD}^{\text{mnop}} \, \sigma_1 (\nabla^a \lambda_m) (\nabla_b \nabla_a \lambda_p) (\nabla^b \lambda_n) (\nabla_c \sigma_2) (\nabla^c \lambda_o) - \\
& \mathcal{DDDD}^{\text{mnop}} \, \sigma_1 (\nabla_a \sigma_2) (\nabla^a \lambda_m) (\nabla^b \lambda_n) (\nabla_c \nabla_b \lambda_p) (\nabla^c \lambda_o) - \\
& \sigma_1 (\nabla_a \lambda^n) (\nabla^a \lambda^m) (\nabla_b \sigma_2) (\nabla^b \lambda^o) (\nabla_c \mathcal{DDDD}_{monp}) (\nabla^c \lambda^p) - \\
& \mathcal{DDDD}^{\text{mnop}} \, \sigma_1 (\nabla_a \lambda_o) (\nabla^a \lambda_m) (\nabla_b \nabla_c \lambda_p) (\nabla^b \lambda_n) (\nabla^c \sigma_2) \\
\\
& \text{T}[36]: 2 \, C\text{Chat}^{\text{mn}} \, \sigma_1 (\nabla_a \nabla_c \nabla^c \lambda_n) (\nabla^a \sigma_2) (\nabla_b \nabla^b \lambda_m) - 2 \, C\text{Chat}^{\text{mn}} \, \sigma_1 (\nabla^a \sigma_2) (\nabla_b \nabla_c \nabla^c \lambda_n) (\nabla^b \nabla_a \lambda_m) + \\
& 2 \, \sigma_1 (\nabla_a \sigma_2) (\nabla^a C\text{Chat}^{\text{mn}}) (\nabla_b \nabla^b \lambda_m) (\nabla_c \nabla^c \lambda_n) - 2 \, \sigma_1 (\nabla_a \nabla_b \lambda_m) (\nabla^a C\text{Chat}^{\text{mn}}) (\nabla^b \sigma_2) (\nabla_c \nabla^c \lambda_n) \\
\\
& \text{T}[37]: - C\text{Chatp}^{\text{mn}} \, \sigma_1 (\nabla^a \sigma_2) (\nabla_b \nabla_c \nabla^c \lambda_n) (\nabla^b \nabla_a \lambda_m) - \\
& \sigma_1 (\nabla^a \sigma_2) (\nabla^b C\text{Chatp}^{\text{mn}}) (\nabla_c \nabla_b \lambda_n) (\nabla^c \nabla_a \lambda_m) + 2 \, C\text{Chatp}^{\text{mn}} \, \sigma_1 (\nabla_a \nabla_c \nabla_b \lambda_n) (\nabla^a \sigma_2) (\nabla^c \nabla^b \lambda_m) - \\
& C\text{Chatp}^{\text{mn}} \, \sigma_1 (\nabla^a \sigma_2) (\nabla_b \nabla_c \nabla_a \lambda_n) (\nabla^c \nabla^b \lambda_m) + \sigma_1 (\nabla_a C\text{Chatp}^{\text{mn}}) (\nabla^a \sigma_2) (\nabla_c \nabla_b \lambda_n) (\nabla^c \nabla^b \lambda_m)
\end{aligned}$$

$$\begin{aligned}
\text{T[38]} : & - CCC^{mnp} \sigma_1 (\nabla_a \sigma_2) (\nabla^a \lambda_m) (\nabla_b \nabla_c \nabla^c \lambda_p) (\nabla^b \lambda_n) + \\
& CCC^{mnp} \sigma_1 (\nabla_a \nabla_c \lambda_p) (\nabla^a \lambda_m) (\nabla_b \nabla^c \lambda_n) (\nabla^b \sigma_2) + CCC^{mnp} \sigma_1 (\nabla^a \lambda_m) (\nabla_b \nabla^c \lambda_n) (\nabla^b \sigma_2) (\nabla_c \nabla_a \lambda_p) - \\
& \sigma_1 (\nabla_a \sigma_2) (\nabla^a \lambda^m) (\nabla_b \nabla_c \lambda_p) (\nabla^b \lambda^n) (\nabla^c CCC_{mn}^p) + \\
& \sigma_1 (\nabla^a \lambda^m) (\nabla_b \nabla_a \lambda_p) (\nabla^b \lambda^n) (\nabla_c CCC_{mn}^p) (\nabla^c \sigma_2) + \\
& CCC^{mnp} \sigma_1 (\nabla^a \lambda_m) (\nabla^b \lambda_n) (\nabla_c \nabla_b \nabla_a \lambda_p) (\nabla^c \sigma_2) - \\
& CCC^{mnp} \sigma_1 (\nabla_a \nabla_c \lambda_p) (\nabla^a \lambda_m) (\nabla^b \sigma_2) (\nabla^c \nabla_b \lambda_n) - CCC^{mnp} \sigma_1 (\nabla_a \sigma_2) (\nabla^a \lambda_m) (\nabla_b \nabla_c \lambda_p) (\nabla^c \nabla^b \lambda_n) \\
\text{T[39]} : & - 2 CCCp^{mnp} \sigma_1 (\nabla_a \sigma_2) (\nabla^a \lambda_m) (\nabla_b \nabla_c \nabla^c \lambda_p) (\nabla^b \lambda_n) + \\
& 2 CCCp^{mnp} \sigma_1 (\nabla_a \nabla_c \lambda_p) (\nabla^a \lambda_m) (\nabla_b \nabla^c \lambda_n) (\nabla^b \sigma_2) + \\
& 2 CCCp^{mnp} \sigma_1 (\nabla^a \lambda_n) (\nabla_b \nabla^c \lambda_m) (\nabla^b \sigma_2) (\nabla_c \nabla_a \lambda_p) - \\
& 2 \sigma_1 (\nabla_a \nabla_c \lambda_p) (\nabla^a CCCp^{mnp}) (\nabla_b \sigma_2) (\nabla^b \lambda_m) (\nabla^c \lambda_n) + \\
& 2 \sigma_1 (\nabla_a \sigma_2) (\nabla^a CCCp^{mnp}) (\nabla_b \nabla_c \lambda_p) (\nabla^b \lambda_m) (\nabla^c \lambda_n) + \\
& 2 CCCp^{mnp} \sigma_1 (\nabla^a \lambda_m) (\nabla^b \lambda_n) (\nabla_c \nabla_a \nabla_b \lambda_p) (\nabla^c \sigma_2) - \\
& 2 CCCp^{mnp} \sigma_1 (\nabla^a \lambda_n) (\nabla^b \sigma_2) (\nabla_c \nabla_a \lambda_p) (\nabla^c \nabla_b \lambda_m) - \\
& 2 CCCp^{mnp} \sigma_1 (\nabla_a \sigma_2) (\nabla^a \lambda_m) (\nabla_c \nabla_b \lambda_p) (\nabla^c \nabla^b \lambda_n) \\
\text{T[40]} : & \sigma_1 (\nabla_a \lambda^n) (\nabla^a \lambda^m) (\nabla_b CCCpp_{mn}^p) (\nabla^b \sigma_2) (\nabla_c \nabla^c \lambda_p) + \\
& 2 CCCpp^{mnp} \sigma_1 (\nabla^a \lambda_m) (\nabla_b \nabla_a \lambda_n) (\nabla^b \sigma_2) (\nabla_c \nabla^c \lambda_p) - \\
& \sigma_1 (\nabla_a \lambda^n) (\nabla^a \lambda^m) (\nabla^b \sigma_2) (\nabla_c \nabla_b \lambda_p) (\nabla^c CCCpp_{mn}^p) - \\
& 2 CCCpp^{mnp} \sigma_1 (\nabla^a \lambda_m) (\nabla^b \sigma_2) (\nabla_c \nabla_b \lambda_p) (\nabla^c \nabla_a \lambda_n) \\
\text{T[41]} : & - \frac{1}{2} CCCc^{mnop} \sigma_1 (\nabla_a \sigma_2) (\nabla^a \lambda_m) (\nabla_b \lambda_p) (\nabla^b \lambda_o) (\nabla_c \nabla^c \lambda_n) - \\
& CCCc^{mnop} \sigma_1 (\nabla_a \sigma_2) (\nabla^a \lambda_m) (\nabla_b \nabla_c \lambda_p) (\nabla^b \lambda_n) (\nabla^c \lambda_o) - \\
& \frac{1}{2} \sigma_1 (\nabla_a \lambda^n) (\nabla^a \lambda^m) (\nabla_b \sigma_2) (\nabla^b \lambda^o) (\nabla_c CCCc_{opmn}) (\nabla^c \lambda^p) - \\
& \frac{1}{2} CCCc^{mnop} \sigma_1 (\nabla_a \nabla_c \lambda_n) (\nabla^a \lambda_m) (\nabla_b \lambda_p) (\nabla^b \lambda_o) (\nabla^c \sigma_2) + \\
& \frac{1}{2} \sigma_1 (\nabla_a \lambda^n) (\nabla^a \lambda^m) (\nabla_b \lambda^p) (\nabla^b \lambda^o) (\nabla_c CCCc_{mnop}) (\nabla^c \sigma_2) + \\
& CCCc^{mnop} \sigma_1 (\nabla^a \lambda_m) (\nabla_b \lambda_p) (\nabla^b \lambda_o) (\nabla_c \nabla_a \lambda_n) (\nabla^c \sigma_2) + \\
& CCCc^{mnop} \sigma_1 (\nabla_a \lambda_n) (\nabla^a \lambda_m) (\nabla^b \lambda_o) (\nabla_c \nabla_b \lambda_p) (\nabla^c \sigma_2) \\
\text{T[42]} : & - 2 \mathcal{B}^m \sigma_1 (\nabla_a \nabla_c \nabla^c \nabla_b \nabla^b \lambda_m) (\nabla^a \sigma_2) - 2 \sigma_1 (\nabla_a \sigma_2) (\nabla^a \mathcal{B}^m) (\nabla_c \nabla^c \nabla_b \nabla^b \lambda_m) \\
\text{T[43]} : & - 2 \mathcal{B}\mathcal{B}\mathcal{h}\mathcal{a}\mathcal{t}^{mn} \sigma_1 (\nabla_a \nabla_c \nabla^c \lambda_n) (\nabla^a \sigma_2) (\nabla_b \nabla^b \lambda_m) - \sigma_1 (\nabla_a \mathcal{B}\mathcal{B}\mathcal{h}\mathcal{a}\mathcal{t}^{mn}) (\nabla^a \sigma_2) (\nabla_b \nabla^b \lambda_m) (\nabla_c \nabla^c \lambda_n) \\
\text{T[44]} : & - 2 \mathcal{B}\mathcal{B}\mathcal{h}\mathcal{a}\mathcal{t}\mathcal{p}^{mn} \sigma_1 (\nabla_a \nabla_c \nabla_b \lambda_n) (\nabla^a \sigma_2) (\nabla^c \nabla^b \lambda_m) - \sigma_1 (\nabla_a \mathcal{B}\mathcal{B}\mathcal{h}\mathcal{a}\mathcal{t}\mathcal{p}^{mn}) (\nabla^a \sigma_2) (\nabla_c \nabla_b \lambda_n) (\nabla^c \nabla^b \lambda_m) \\
\text{T[45]} : & - \mathcal{B}\mathcal{B}\mathcal{B}^{mnp} \sigma_1 (\nabla_a \lambda_n) (\nabla^a \lambda_m) (\nabla_b \nabla_c \nabla^c \lambda_p) (\nabla^b \sigma_2) - \\
& \sigma_1 (\nabla_a \lambda^n) (\nabla^a \lambda^m) (\nabla_b \mathcal{B}\mathcal{B}\mathcal{B}_{mn}^p) (\nabla^b \sigma_2) (\nabla_c \nabla^c \lambda_p) - \\
& 2 \mathcal{B}\mathcal{B}\mathcal{B}^{mnp} \sigma_1 (\nabla^a \lambda_m) (\nabla_b \nabla_a \lambda_n) (\nabla^b \sigma_2) (\nabla_c \nabla^c \lambda_p)
\end{aligned}$$

[illegible]

$$\begin{aligned} \mathbf{T}[52]: & \frac{3}{4} \mathcal{A}\mathcal{A}\mathcal{A}\text{hat}_m^{\text{np}} \beta^m \sigma 1 (\nabla_a \nabla_c \nabla^c \lambda_p) (\nabla^a \sigma 2) (\nabla_b \nabla^b \lambda_n) - \\ & \frac{3}{8} \mathcal{A}\mathcal{A}\mathcal{A}\text{hat}_m^{\text{mnp}} \sigma 1 (\nabla_a \sigma 2) (\nabla^a \beta_m) (\nabla_b \nabla^b \lambda_n) (\nabla_c \nabla^c \lambda_p) - \\ & \frac{3}{2} \mathcal{A}\mathcal{A}\mathcal{A}\text{hat}_m^{\text{mnp}} \sigma 1 (\nabla_a \sigma 2) (\nabla^a \lambda_m) (\nabla_b \nabla^b \lambda_n) (\nabla_c \nabla^c \lambda_p) + \\ & \frac{3}{8} \beta^m \sigma 1 (\nabla_a \mathcal{A}\mathcal{A}\mathcal{A}\text{hat}_m^{\text{np}}) (\nabla^a \sigma 2) (\nabla_b \nabla^b \lambda_n) (\nabla_c \nabla^c \lambda_p) \\ \mathbf{T}[53]: & \mathcal{A}\mathcal{A}\mathcal{A}\text{hatp}_m^{\text{np}} \beta^m \sigma 1 (\nabla_a \nabla_c \nabla^c \lambda_n) (\nabla^a \sigma 2) (\nabla_b \nabla^b \lambda_p) + \\ & \mathcal{A}\mathcal{A}\mathcal{A}\text{hatp}_m^{\text{np}} \beta^m \sigma 1 (\nabla^a \sigma 2) (\nabla_b \nabla_c \nabla^c \lambda_p) (\nabla^b \nabla_a \lambda_n) - \\ & \mathcal{A}\mathcal{A}\mathcal{A}\text{hatp}_m^{\text{mnp}} \sigma 1 (\nabla_a \sigma 2) (\nabla^a \lambda_m) (\nabla_b \nabla^b \lambda_n) (\nabla_c \nabla^c \lambda_p) + \\ & \beta^m \sigma 1 (\nabla^a \sigma 2) (\nabla_b \nabla_a \lambda_n) (\nabla^b \mathcal{A}\mathcal{A}\mathcal{A}\text{hatp}_m^{\text{np}}) (\nabla_c \nabla^c \lambda_p) + \\ & \mathcal{A}\mathcal{A}\mathcal{A}\text{hatp}_m^{\text{mnp}} \sigma 1 (\nabla_a \nabla_b \lambda_n) (\nabla^a \lambda_m) (\nabla^b \sigma 2) (\nabla_c \nabla^c \lambda_p) - \\ & \mathcal{A}\mathcal{A}\mathcal{A}\text{hatp}_m^{\text{mnp}} \sigma 1 (\nabla^a \beta_m) (\nabla_b \nabla_a \lambda_n) (\nabla^b \sigma 2) (\nabla_c \nabla^c \lambda_p) + \\ & \mathcal{A}\mathcal{A}\mathcal{A}\text{hatp}_m^{\text{mnp}} \sigma 1 (\nabla^a \lambda_m) (\nabla_b \nabla_a \lambda_n) (\nabla^b \sigma 2) (\nabla_c \nabla^c \lambda_p) - \\ & \frac{1}{2} \mathcal{A}\mathcal{A}\mathcal{A}\text{hatp}_m^{\text{mnp}} \sigma 1 (\nabla_a \sigma 2) (\nabla^a \beta_p) (\nabla_c \nabla_b \lambda_n) (\nabla^c \nabla^b \lambda_m) - \\ & 2 \mathcal{A}\mathcal{A}\mathcal{A}\text{hatp}_m^{\text{mnp}} \sigma 1 (\nabla_a \sigma 2) (\nabla^a \lambda_p) (\nabla_c \nabla_b \lambda_n) (\nabla^c \nabla^b \lambda_m) + \\ & \mathcal{A}\mathcal{A}\mathcal{A}\text{hatp}_m^{\text{np}} \beta^m \sigma 1 (\nabla_a \nabla_c \nabla_b \lambda_p) (\nabla^a \sigma 2) (\nabla^c \nabla^b \lambda_n) + \\ & \frac{1}{2} \beta^m \sigma 1 (\nabla_a \mathcal{A}\mathcal{A}\mathcal{A}\text{hatp}_m^{\text{np}}) (\nabla^a \sigma 2) (\nabla_c \nabla_b \lambda_p) (\nabla^c \nabla^b \lambda_n) \end{aligned}$$

$$\begin{aligned}
\text{T}[54]: & - \mathcal{A}\mathcal{A}\mathcal{A}\text{hatpp}^{\text{mnp}} \beta_p \sigma_1 (\nabla_a \nabla_c \nabla^c \lambda_n) (\nabla^a \sigma_2) (\nabla_b \nabla^b \lambda_m) - \\
& \mathcal{A}\mathcal{A}\mathcal{A}\text{hatpp}^{\text{mnp}} \beta_p \sigma_1 (\nabla_a \nabla_c \nabla^c \lambda_m) (\nabla^a \sigma_2) (\nabla_b \nabla^b \lambda_n) - \\
& \mathcal{A}\mathcal{A}\mathcal{A}\text{hatpp}^{\text{mnp}} \beta_m \sigma_1 (\nabla_a \nabla_c \nabla^c \lambda_p) (\nabla^a \sigma_2) (\nabla_b \nabla^b \lambda_n) - \\
& \mathcal{A}\mathcal{A}\mathcal{A}\text{hatpp}^{\text{mnp}} \beta_p \sigma_1 (\nabla_a \nabla^b \lambda_m) (\nabla^a \sigma_2) (\nabla_b \nabla_c \nabla^c \lambda_n) + \\
& \mathcal{A}\mathcal{A}\mathcal{A}\text{hatpp}^{\text{mnp}} \beta_n \sigma_1 (\nabla_a \nabla^b \lambda_m) (\nabla^a \sigma_2) (\nabla_b \nabla_c \nabla^c \lambda_p) + \\
& \mathcal{A}\mathcal{A}\mathcal{A}\text{hatpp}^{\text{mnp}} \sigma_1 (\nabla_a \sigma_2) (\nabla^a \beta_p) (\nabla_b \nabla_c \nabla^c \lambda_n) (\nabla^b \lambda_m) - \\
& \mathcal{A}\mathcal{A}\mathcal{A}\text{hatpp}^{\text{mnp}} \sigma_1 (\nabla_a \sigma_2) (\nabla^a \beta_n) (\nabla_b \nabla_c \nabla^c \lambda_p) (\nabla^b \lambda_m) - \\
& 4 \mathcal{A}\mathcal{A}\mathcal{A}\text{hatpp}^{\text{mnp}} \sigma_1 (\nabla_a \nabla_c \nabla^c \lambda_p) (\nabla^a \lambda_m) (\nabla_b \sigma_2) (\nabla^b \lambda_n) + \\
& \beta^m \sigma_1 (\nabla_a \sigma_2) (\nabla^a \mathcal{A}\mathcal{A}\mathcal{A}\text{hatpp}^{\text{n p}}_m) (\nabla_b \nabla_c \nabla^c \lambda_p) (\nabla^b \lambda_n) - \\
& \beta^m \sigma_1 (\nabla_a \sigma_2) (\nabla^a \mathcal{A}\mathcal{A}\mathcal{A}\text{hatpp}^{\text{np}}_m) (\nabla_b \nabla_c \nabla^c \lambda_p) (\nabla^b \lambda_n) + \\
& 4 \mathcal{A}\mathcal{A}\mathcal{A}\text{hatpp}^{\text{mnp}} \sigma_1 (\nabla_a \sigma_2) (\nabla^a \lambda_m) (\nabla_b \nabla_c \nabla^c \lambda_n) (\nabla^b \lambda_p) - \\
& \mathcal{A}\mathcal{A}\mathcal{A}\text{hatpp}^{\text{mnp}} \beta_p \sigma_1 (\nabla^a \lambda_m) (\nabla_b \nabla_a \nabla_c \nabla^c \lambda_n) (\nabla^b \sigma_2) + \\
& \mathcal{A}\mathcal{A}\mathcal{A}\text{hatpp}^{\text{mnp}} \beta_n \sigma_1 (\nabla^a \lambda_m) (\nabla_b \nabla_a \nabla_c \nabla^c \lambda_p) (\nabla^b \sigma_2) - \\
& \beta^m \sigma_1 (\nabla_a \lambda_n) (\nabla^a \mathcal{A}\mathcal{A}\mathcal{A}\text{hatpp}^{\text{np}}_m) (\nabla_b \nabla_c \nabla^c \lambda_p) (\nabla^b \sigma_2) - \\
& \mathcal{A}\mathcal{A}\mathcal{A}\text{hatpp}^{\text{mnp}} \sigma_1 (\nabla_a \sigma_2) (\nabla^a \lambda_m) (\nabla_b \nabla^b \beta_p) (\nabla_c \nabla^c \lambda_n) + \\
& \mathcal{A}\mathcal{A}\mathcal{A}\text{hatpp}^{\text{mnp}} \sigma_1 (\nabla_a \sigma_2) (\nabla^a \beta_p) (\nabla_b \nabla^b \lambda_m) (\nabla_c \nabla^c \lambda_n) + \\
& \sigma_1 (\nabla_a \lambda_m) (\nabla^a \mathcal{A}\mathcal{A}\mathcal{A}\text{hatpp}^{\text{mnp}}) (\nabla_b \sigma_2) (\nabla^b \beta_p) (\nabla_c \nabla^c \lambda_n) + \\
& 4 \sigma_1 (\nabla_a \lambda_p) (\nabla^a \mathcal{A}\mathcal{A}\mathcal{A}\text{hatpp}^{\text{mnp}}) (\nabla_b \sigma_2) (\nabla^b \lambda_m) (\nabla_c \nabla^c \lambda_n) - \\
& 4 \mathcal{A}\mathcal{A}\mathcal{A}\text{hatpp}^{\text{mnp}} \sigma_1 (\nabla_a \nabla_b \lambda_p) (\nabla^a \lambda_m) (\nabla^b \sigma_2) (\nabla_c \nabla^c \lambda_n) + \\
& 4 \mathcal{A}\mathcal{A}\mathcal{A}\text{hatpp}^{\text{mnp}} \sigma_1 (\nabla_a \nabla_b \lambda_m) (\nabla^a \lambda_p) (\nabla^b \sigma_2) (\nabla_c \nabla^c \lambda_n) - \\
& \beta^m \sigma_1 (\nabla_a \sigma_2) (\nabla^a \mathcal{A}\mathcal{A}\mathcal{A}\text{hatpp}^{\text{np}}_m) (\nabla_b \nabla^b \lambda_n) (\nabla_c \nabla^c \lambda_p) + \\
& 6 \mathcal{A}\mathcal{A}\mathcal{A}\text{hatpp}^{\text{mnp}} \sigma_1 (\nabla_a \sigma_2) (\nabla^a \lambda_m) (\nabla_b \nabla^b \lambda_n) (\nabla_c \nabla^c \lambda_p) - \\
& \beta^m \sigma_1 (\nabla^a \lambda^n) (\nabla_b \nabla_a \mathcal{A}\mathcal{A}\mathcal{A}\text{hatpp}^{\text{p}}_n) (\nabla^b \sigma_2) (\nabla_c \nabla^c \lambda_p) - \\
& \beta^m \sigma_1 (\nabla^a \mathcal{A}\mathcal{A}\mathcal{A}\text{hatpp}^{\text{np}}_m) (\nabla_b \nabla_a \lambda_n) (\nabla^b \sigma_2) (\nabla_c \nabla^c \lambda_p)
\end{aligned}$$



$$\begin{aligned}
\text{T}[55]: & - \mathcal{A}\mathcal{A}\mathcal{A}\text{hatp}_m^{\text{np}} \beta^m \sigma_1 (\nabla_a \nabla^b \lambda_n) (\nabla^a \sigma_2) (\nabla_b \nabla_c \nabla^c \lambda_p) - \\
& \mathcal{A}\mathcal{A}\mathcal{A}\text{hatp}_m^{\text{np}} \beta^m \sigma_1 (\nabla_a \nabla^b \lambda_n) (\nabla^a \sigma_2) (\nabla_b \nabla_c \nabla^c \lambda_p) + \\
& \beta^m \sigma_1 (\nabla_a \sigma_2) (\nabla^a \lambda^n) (\nabla_b \nabla_c \nabla^c \lambda_p) (\nabla^b \mathcal{A}\mathcal{A}\mathcal{A}\text{hatp}_{mn}^p) + \\
& \mathcal{A}\mathcal{A}\mathcal{A}\text{hatp}^{\text{mnp}} \sigma_1 (\nabla_a \sigma_2) (\nabla^a \beta_p) (\nabla_b \nabla_c \nabla^c \lambda_n) (\nabla^b \lambda_m) + \\
& 4 \mathcal{A}\mathcal{A}\mathcal{A}\text{hatp}^{\text{mnp}} \sigma_1 (\nabla_a \nabla_c \nabla^c \lambda_n) (\nabla^a \lambda_m) (\nabla_b \sigma_2) (\nabla^b \lambda_p) - \\
& \beta^m \sigma_1 (\nabla_a \nabla_c \nabla^c \lambda_p) (\nabla^a \lambda^n) (\nabla_b \mathcal{A}\mathcal{A}\mathcal{A}\text{hatp}_n^p) (\nabla^b \sigma_2) - \\
& \mathcal{A}\mathcal{A}\mathcal{A}\text{hatp}_m^{\text{np}} \beta^m \sigma_1 (\nabla^a \lambda_n) (\nabla_b \nabla_a \nabla_c \nabla^c \lambda_p) (\nabla^b \sigma_2) - \\
& \beta^m \sigma_1 (\nabla_a \nabla^c \lambda^p) (\nabla^a \lambda^n) (\nabla_b \nabla_c \mathcal{A}\mathcal{A}\mathcal{A}\text{hatp}_{n\text{p}m}) (\nabla^b \sigma_2) - \\
& \mathcal{A}\mathcal{A}\mathcal{A}\text{hatp}^{\text{mnp}} \sigma_1 (\nabla_a \lambda_n) (\nabla^a \beta_m) (\nabla_b \nabla_c \nabla^c \lambda_p) (\nabla^b \sigma_2) + \\
& \mathcal{A}\mathcal{A}\mathcal{A}\text{hatp}^{\text{mnp}} \sigma_1 (\nabla_a \lambda_n) (\nabla^a \lambda_m) (\nabla_b \nabla_c \nabla^c \lambda_p) (\nabla^b \sigma_2) + \\
& \mathcal{A}\mathcal{A}\mathcal{A}\text{hatp}_m^{\text{np}} \beta^m \sigma_1 (\nabla^a \sigma_2) (\nabla_b \nabla_c \nabla^c \lambda_p) (\nabla^b \nabla_a \lambda_n) - \\
& \mathcal{A}\mathcal{A}\mathcal{A}\text{hatp}^{\text{mnp}} \sigma_1 (\nabla_a \nabla_b \lambda_n) (\nabla^a \lambda_m) (\nabla^b \sigma_2) (\nabla_c \nabla^c \beta_p) + \\
& 2 \mathcal{A}\mathcal{A}\mathcal{A}\text{hatp}^{\text{mnp}} \sigma_1 (\nabla_a \nabla_b \lambda_n) (\nabla^a \lambda_m) (\nabla^b \sigma_2) (\nabla_c \nabla^c \lambda_p) + \\
& \mathcal{A}\mathcal{A}\mathcal{A}\text{hatp}_m^{\text{np}} \beta^m \sigma_1 (\nabla_a \sigma_2) (\nabla^a \lambda_n) (\nabla_c \nabla^c \nabla_b \nabla^b \lambda_p) + \\
& \sigma_1 (\nabla_a \sigma_2) (\nabla^a \beta^m) (\nabla_b \nabla_c \lambda_p) (\nabla^b \lambda^n) (\nabla^c \mathcal{A}\mathcal{A}\mathcal{A}\text{hatp}_n^p) + \\
& 4 \sigma_1 (\nabla_a \sigma_2) (\nabla^a \lambda^m) (\nabla_b \nabla_c \lambda_p) (\nabla^b \lambda^n) (\nabla^c \mathcal{A}\mathcal{A}\mathcal{A}\text{hatp}_n^p) - \\
& \beta^m \sigma_1 (\nabla^a \lambda^n) (\nabla_b \nabla_a \nabla_c \lambda_p) (\nabla^b \sigma_2) (\nabla^c \mathcal{A}\mathcal{A}\mathcal{A}\text{hatp}_n^p) - \\
& \beta^m \sigma_1 (\nabla_a \nabla_c \lambda_p) (\nabla^a \sigma_2) (\nabla^b \mathcal{A}\mathcal{A}\mathcal{A}\text{hatp}_m^{\text{np}}) (\nabla^c \nabla_b \lambda_n) + \\
& \mathcal{A}\mathcal{A}\mathcal{A}\text{hatp}^{\text{mnp}} \sigma_1 (\nabla_a \sigma_2) (\nabla^a \beta_p) (\nabla_b \nabla_c \lambda_n) (\nabla^c \nabla^b \lambda_m) + \\
& 4 \mathcal{A}\mathcal{A}\mathcal{A}\text{hatp}^{\text{mnp}} \sigma_1 (\nabla_a \sigma_2) (\nabla^a \lambda_p) (\nabla_b \nabla_c \lambda_n) (\nabla^c \nabla^b \lambda_m) - \\
& 2 \mathcal{A}\mathcal{A}\mathcal{A}\text{hatp}_m^{\text{np}} \beta^m \sigma_1 (\nabla_a \nabla_b \nabla_c \lambda_p) (\nabla^a \sigma_2) (\nabla^c \nabla^b \lambda_n) - \\
& \beta^m \sigma_1 (\nabla_a \mathcal{A}\mathcal{A}\mathcal{A}\text{hatp}_m^{\text{np}}) (\nabla^a \sigma_2) (\nabla_b \nabla_c \lambda_p) (\nabla^c \nabla^b \lambda_n)
\end{aligned}$$

$$\begin{aligned} \mathbf{T}[57]: \mathcal{AA}\mathcal{A}\text{checkpp}^{\text{np}}_{\text{m}} \beta^{\text{m}} \sigma 1 \left( \nabla_{\text{a}} \nabla_{\text{c}} \nabla^{\text{c}} \lambda_{\text{p}} \right) \left( \nabla^{\text{a}} \sigma 2 \right) \left( \nabla_{\text{b}} \nabla^{\text{b}} \lambda_{\text{n}} \right) + \\ \mathcal{AA}\mathcal{A}\text{checkpp}^{\text{np}}_{\text{m}} \beta^{\text{m}} \sigma 1 \left( \nabla_{\text{a}} \nabla^{\text{b}} \lambda_{\text{n}} \right) \left( \nabla^{\text{a}} \sigma 2 \right) \left( \nabla_{\text{b}} \nabla_{\text{c}} \nabla^{\text{c}} \lambda_{\text{p}} \right) - \\ \mathcal{AA}\mathcal{A}\text{checkpp}^{\text{mnp}} \sigma 1 \left( \nabla_{\text{a}} \sigma 2 \right) \left( \nabla^{\text{a}} \beta_{\text{p}} \right) \left( \nabla_{\text{b}} \nabla_{\text{c}} \nabla^{\text{c}} \lambda_{\text{n}} \right) \left( \nabla^{\text{b}} \lambda_{\text{m}} \right) + \\ \frac{1}{2} \mathcal{AA}\mathcal{A}\text{checkpp}^{\text{mnp}} \sigma 1 \left( \nabla_{\text{a}} \sigma 2 \right) \left( \nabla^{\text{a}} \lambda_{\text{m}} \right) \left( \nabla_{\text{b}} \nabla_{\text{c}} \nabla^{\text{c}} \beta_{\text{p}} \right) \left( \nabla^{\text{b}} \lambda_{\text{n}} \right) + \\ 4 \mathcal{AA}\mathcal{A}\text{checkpp}^{\text{mnp}} \sigma 1 \left( \nabla_{\text{a}} \sigma 2 \right) \left( \nabla^{\text{a}} \lambda_{\text{m}} \right) \left( \nabla_{\text{b}} \nabla_{\text{c}} \nabla^{\text{c}} \lambda_{\text{p}} \right) \left( \nabla^{\text{b}} \lambda_{\text{n}} \right) - \\ 2 \mathcal{AA}\mathcal{A}\text{checkpp}^{\text{mnp}} \sigma 1 \left( \nabla_{\text{a}} \nabla_{\text{c}} \nabla^{\text{c}} \lambda_{\text{n}} \right) \left( \nabla^{\text{a}} \lambda_{\text{m}} \right) \left( \nabla_{\text{b}} \sigma 2 \right) \left( \nabla^{\text{b}} \lambda_{\text{p}} \right) - \\ 2 \mathcal{AA}\mathcal{A}\text{checkpp}^{\text{mnp}} \sigma 1 \left( \nabla_{\text{a}} \sigma 2 \right) \left( \nabla^{\text{a}} \lambda_{\text{m}} \right) \left( \nabla_{\text{b}} \nabla_{\text{c}} \nabla^{\text{c}} \lambda_{\text{n}} \right) \left( \nabla^{\text{b}} \lambda_{\text{p}} \right) - \\ \frac{1}{2} \mathcal{AA}\mathcal{A}\text{checkpp}^{\text{np}}_{\text{m}} \beta^{\text{m}} \sigma 1 \left( \nabla_{\text{a}} \nabla_{\text{b}} \nabla_{\text{c}} \nabla^{\text{c}} \lambda_{\text{p}} \right) \left( \nabla^{\text{a}} \lambda_{\text{n}} \right) \left( \nabla^{\text{b}} \sigma 2 \right) + \\ \beta^{\text{m}} \sigma 1 \left( \nabla_{\text{a}} \nabla_{\text{c}} \nabla^{\text{c}} \lambda_{\text{p}} \right) \left( \nabla^{\text{a}} \lambda^{\text{n}} \right) \left( \nabla_{\text{b}} \mathcal{AA}\mathcal{A}\text{checkpp}^{\text{p}}_{\text{m}} \right) \left( \nabla^{\text{b}} \sigma 2 \right) - \end{aligned}$$

$$\begin{aligned}
& \frac{1}{2} \mathcal{A}\mathcal{A}\mathcal{A}\text{checkpp}_m^{\text{np}} \beta^m \sigma 1 (\nabla^a \lambda_n) (\nabla_b \nabla_a \nabla_c \nabla^c \lambda_p) (\nabla^b \sigma 2) + \\
& \mathcal{A}\mathcal{A}\mathcal{A}\text{checkpp}_m^{\text{np}} \beta^m \sigma 1 (\nabla^a \lambda_n) (\nabla_b \nabla_a \nabla_c \nabla^c \lambda_p) (\nabla^b \sigma 2) + \\
& \beta^m \sigma 1 (\nabla_a \nabla^c \lambda^p) (\nabla^a \lambda^n) (\nabla_b \nabla_c \mathcal{A}\mathcal{A}\mathcal{A}\text{checkpp}_{\text{npm}}) (\nabla^b \sigma 2) - \\
& \frac{1}{2} \mathcal{A}\mathcal{A}\mathcal{A}\text{checkpp}^{\text{mnp}} \sigma 1 (\nabla_a \lambda_n) (\nabla^a \lambda_m) (\nabla_b \nabla_c \nabla^c \lambda_p) (\nabla^b \sigma 2) + \\
& \beta^m \sigma 1 (\nabla_a \mathcal{A}\mathcal{A}\mathcal{A}\text{checkpp}_n^{\text{p}}) (\nabla^a \lambda^n) (\nabla_b \nabla_c \nabla^c \lambda_p) (\nabla^b \sigma 2) + \\
& \frac{1}{2} \beta^m \sigma 1 (\nabla_a \nabla_c \mathcal{A}\mathcal{A}\mathcal{A}\text{checkpp}_{\text{npm}}) (\nabla^a \lambda^n) (\nabla_b \nabla^c \lambda^p) (\nabla^b \sigma 2) + \\
& \frac{1}{2} \beta^m \sigma 1 (\nabla^a \lambda^n) (\nabla_b \nabla^c \lambda^p) (\nabla^b \sigma 2) (\nabla_c \nabla_a \mathcal{A}\mathcal{A}\mathcal{A}\text{checkpp}_{\text{npm}}) + \\
& \mathcal{A}\mathcal{A}\mathcal{A}\text{checkpp}^{\text{mnp}} \sigma 1 (\nabla_a \nabla^c \beta_p) (\nabla^a \lambda_m) (\nabla^b \sigma 2) (\nabla_c \nabla_b \lambda_n) - \\
& 2 \mathcal{A}\mathcal{A}\mathcal{A}\text{checkpp}^{\text{mnp}} \sigma 1 (\nabla_a \nabla^c \lambda_n) (\nabla^a \lambda_m) (\nabla^b \sigma 2) (\nabla_c \nabla_b \lambda_p) + \\
& \frac{1}{2} \sigma 1 (\nabla_a \sigma 2) (\nabla^a \lambda^m) (\nabla_b \mathcal{A}\mathcal{A}\mathcal{A}\text{checkpp}_{\text{mn}}^{\text{p}}) (\nabla^b \lambda^n) (\nabla_c \nabla^c \beta_p) + \\
& \frac{1}{2} \mathcal{A}\mathcal{A}\mathcal{A}\text{checkpp}^{\text{mnp}} \sigma 1 (\nabla_a \nabla_b \lambda_n) (\nabla^a \lambda_m) (\nabla^b \sigma 2) (\nabla_c \nabla^c \beta_p) + \\
& \frac{1}{2} \mathcal{A}\mathcal{A}\mathcal{A}\text{checkpp}^{\text{mnp}} \sigma 1 (\nabla_a \sigma 2) (\nabla^a \lambda_m) (\nabla_b \nabla^b \beta_p) (\nabla_c \nabla^c \lambda_n) - \\
& \frac{1}{2} \mathcal{A}\mathcal{A}\mathcal{A}\text{checkpp}^{\text{mnp}} \sigma 1 (\nabla_a \sigma 2) (\nabla^a \beta_p) (\nabla_b \nabla^b \lambda_m) (\nabla_c \nabla^c \lambda_n) - \\
& \mathcal{A}\mathcal{A}\mathcal{A}\text{checkpp}^{\text{mnp}} \sigma 1 (\nabla_a \nabla_b \beta_p) (\nabla^a \lambda_m) (\nabla^b \sigma 2) (\nabla_c \nabla^c \lambda_n) - \\
& 2 \mathcal{A}\mathcal{A}\mathcal{A}\text{checkpp}^{\text{mnp}} \sigma 1 (\nabla_a \nabla_b \lambda_m) (\nabla^a \lambda_p) (\nabla^b \sigma 2) (\nabla_c \nabla^c \lambda_n) - \\
& 3 \mathcal{A}\mathcal{A}\mathcal{A}\text{checkpp}^{\text{mnp}} \sigma 1 (\nabla_a \sigma 2) (\nabla^a \lambda_m) (\nabla_b \nabla^b \lambda_n) (\nabla_c \nabla^c \lambda_p) + \\
& \frac{1}{2} \beta^m \sigma 1 (\nabla_a \mathcal{A}\mathcal{A}\mathcal{A}\text{checkpp}_m^{\text{np}}) (\nabla^a \sigma 2) (\nabla_b \nabla^b \lambda_n) (\nabla_c \nabla^c \lambda_p) + \\
& \beta^m \sigma 1 (\nabla_a \nabla_b \lambda_n) (\nabla^a \sigma 2) (\nabla^b \mathcal{A}\mathcal{A}\mathcal{A}\text{checkpp}_m^{\text{np}}) (\nabla_c \nabla^c \lambda_p) - \\
& 3 \sigma 1 (\nabla_a \sigma 2) (\nabla^a \lambda^m) (\nabla_b \mathcal{A}\mathcal{A}\mathcal{A}\text{checkpp}_{\text{mn}}^{\text{p}}) (\nabla^b \lambda^n) (\nabla_c \nabla^c \lambda_p) - \\
& 2 \sigma 1 (\nabla_a \sigma 2) (\nabla^a \lambda^m) (\nabla_b \mathcal{A}\mathcal{A}\mathcal{A}\text{checkpp}_m^{\text{p}}) (\nabla^b \lambda^n) (\nabla_c \nabla^c \lambda_p) - \\
& \sigma 1 (\nabla_a \sigma 2) (\nabla^a \beta^m) (\nabla_b \mathcal{A}\mathcal{A}\mathcal{A}\text{checkpp}_n^{\text{p}}) (\nabla^b \lambda^n) (\nabla_c \nabla^c \lambda_p) - \\
& \mathcal{A}\mathcal{A}\mathcal{A}\text{checkpp}^{\text{mnp}} \sigma 1 (\nabla_a \nabla_b \lambda_n) (\nabla^a \lambda_m) (\nabla^b \sigma 2) (\nabla_c \nabla^c \lambda_p) + \\
& \beta^m \sigma 1 (\nabla^a \lambda^n) (\nabla_b \nabla_a \mathcal{A}\mathcal{A}\mathcal{A}\text{checkpp}_{\text{npm}}) (\nabla^b \sigma 2) (\nabla_c \nabla^c \lambda^p) + \\
& \sigma 1 (\nabla_a \sigma 2) (\nabla^a \lambda^m) (\nabla_b \nabla_c \beta_p) (\nabla^b \lambda^n) (\nabla^c \mathcal{A}\mathcal{A}\mathcal{A}\text{checkpp}_{\text{mn}}^{\text{p}}) + \\
& 2 \sigma 1 (\nabla_a \sigma 2) (\nabla^a \lambda^m) (\nabla_b \nabla_c \lambda_p) (\nabla^b \lambda^n) (\nabla^c \mathcal{A}\mathcal{A}\mathcal{A}\text{checkpp}_{\text{mn}}^{\text{p}}) - \\
& 2 \sigma 1 (\nabla_a \sigma 2) (\nabla^a \lambda^m) (\nabla_b \nabla_c \lambda_p) (\nabla^b \lambda^n) (\nabla^c \mathcal{A}\mathcal{A}\mathcal{A}\text{checkpp}_m^{\text{p}}) - \\
& \sigma 1 (\nabla_a \sigma 2) (\nabla^a \beta^m) (\nabla_b \nabla_c \lambda_p) (\nabla^b \lambda^n) (\nabla^c \mathcal{A}\mathcal{A}\mathcal{A}\text{checkpp}_n^{\text{p}}) - \\
& 2 \sigma 1 (\nabla_a \sigma 2) (\nabla^a \lambda^m) (\nabla_b \nabla_c \lambda_p) (\nabla^b \lambda^n) (\nabla^c \mathcal{A}\mathcal{A}\mathcal{A}\text{checkpp}_n^{\text{p}}) + \\
& \beta^m \sigma 1 (\nabla^a \lambda^n) (\nabla_b \nabla_a \nabla_c \lambda_p) (\nabla^b \sigma 2) (\nabla^c \mathcal{A}\mathcal{A}\mathcal{A}\text{checkpp}_n^{\text{p}}) - \\
& 2 \sigma 1 (\nabla_a \sigma 2) (\nabla^a \lambda^m) (\nabla^b \lambda^n) (\nabla_c \nabla_b \mathcal{A}\mathcal{A}\mathcal{A}\text{checkpp}_{\text{npm}}) (\nabla^c \lambda^p) - \\
& \frac{1}{2} \sigma 1 (\nabla_a \sigma 2) (\nabla^a \beta^m) (\nabla^b \lambda^n) (\nabla_c \nabla_b \mathcal{A}\mathcal{A}\mathcal{A}\text{checkpp}_{\text{npm}}) (\nabla^c \lambda^p) - \\
& \mathcal{A}\mathcal{A}\mathcal{A}\text{checkpp}^{\text{mnp}} \sigma 1 (\nabla^a \lambda_m) (\nabla_b \nabla_a \nabla_c \beta_p) (\nabla^b \lambda_n) (\nabla^c \sigma 2) -
\end{aligned}$$

$$\begin{aligned}
& 2 \mathcal{A}\mathcal{A}\mathcal{A}\text{checkpp}^{\text{mnp}} \sigma_1 (\nabla^a \lambda_m) (\nabla_b \nabla_a \nabla_c \lambda_p) (\nabla^b \lambda_n) (\nabla^c \sigma_2) - \\
& \sigma_1 (\nabla_a \mathcal{A}\mathcal{A}\mathcal{A}\text{checkpp}_{\text{mn}}^{\text{p}}) (\nabla^a \lambda^m) (\nabla_b \nabla_c \beta_p) (\nabla^b \lambda^n) (\nabla^c \sigma_2) - \\
& 2 \sigma_1 (\nabla_a \mathcal{A}\mathcal{A}\mathcal{A}\text{checkpp}_{\text{m}}^{\text{p}} \lambda_n) (\nabla^a \lambda^m) (\nabla_b \nabla_c \lambda_p) (\nabla^b \lambda^n) (\nabla^c \sigma_2) + \\
& \frac{1}{2} \beta^m \sigma_1 (\nabla^a \lambda^n) (\nabla^b \lambda^p) (\nabla_c \nabla_b \nabla_a \mathcal{A}\mathcal{A}\mathcal{A}\text{checkpp}_{\text{npm}}) (\nabla^c \sigma_2) - \\
& \mathcal{A}\mathcal{A}\mathcal{A}\text{checkpp}^{\text{mnp}} \sigma_1 (\nabla_a \nabla_c \lambda_n) (\nabla^a \lambda_m) (\nabla^b \sigma_2) (\nabla^c \nabla_b \beta_p) + \\
& \beta^m \sigma_1 (\nabla_a \nabla_c \lambda_p) (\nabla^a \sigma_2) (\nabla^b \mathcal{A}\mathcal{A}\mathcal{A}\text{checkpp}_{\text{m}}^{\text{np}}) (\nabla^c \nabla_b \lambda_n) + \\
& 2 \mathcal{A}\mathcal{A}\mathcal{A}\text{checkpp}^{\text{mnp}} \sigma_1 (\nabla_a \nabla_c \lambda_p) (\nabla^a \lambda_m) (\nabla^b \sigma_2) (\nabla^c \nabla_b \lambda_n) + \\
& \mathcal{A}\mathcal{A}\mathcal{A}\text{checkpp}^{\text{mnp}} \sigma_1 (\nabla_a \sigma_2) (\nabla^a \lambda_m) (\nabla_b \nabla_c \lambda_n) (\nabla^c \nabla^b \beta_p) - \\
& \frac{1}{2} \mathcal{A}\mathcal{A}\mathcal{A}\text{checkpp}^{\text{mnp}} \sigma_1 (\nabla_a \sigma_2) (\nabla^a \beta_p) (\nabla_b \nabla_c \lambda_n) (\nabla^c \nabla^b \lambda_m) - \\
& 2 \mathcal{A}\mathcal{A}\mathcal{A}\text{checkpp}^{\text{mnp}} \sigma_1 (\nabla_a \sigma_2) (\nabla^a \lambda_p) (\nabla_b \nabla_c \lambda_n) (\nabla^c \nabla^b \lambda_m) + \\
& \mathcal{A}\mathcal{A}\mathcal{A}\text{checkpp}_{\text{m}}^{\text{np}} \beta^m \sigma_1 (\nabla_a \nabla_b \nabla_c \lambda_p) (\nabla^a \sigma_2) (\nabla^c \nabla^b \lambda_n) + \\
& 2 \mathcal{A}\mathcal{A}\mathcal{A}\text{checkpp}^{\text{mnp}} \sigma_1 (\nabla_a \sigma_2) (\nabla^a \lambda_m) (\nabla_b \nabla_c \lambda_p) (\nabla^c \nabla^b \lambda_n) + \\
& \frac{1}{2} \beta^m \sigma_1 (\nabla_a \mathcal{A}\mathcal{A}\mathcal{A}\text{checkpp}_{\text{m}}^{\text{np}}) (\nabla^a \sigma_2) (\nabla_b \nabla_c \lambda_p) (\nabla^c \nabla^b \lambda_n) \\
\text{T[58]: } & \frac{1}{2} \mathcal{A}\mathcal{A}\mathcal{A}\text{hat}^{\text{no p}}_{\text{m}} \beta^m \sigma_1 (\nabla_a \lambda_o) (\nabla^a \lambda_n) (\nabla_b \nabla_c \nabla^c \lambda_p) (\nabla^b \sigma_2) - \\
& \frac{1}{2} \mathcal{A}\mathcal{A}\mathcal{A}\text{hat}_{\text{m}}^{\text{nop}} \beta^m \sigma_1 (\nabla_a \sigma_2) (\nabla^a \lambda_n) (\nabla_b \nabla^b \lambda_o) (\nabla_c \nabla^c \lambda_p) - \\
& \frac{1}{2} \mathcal{A}\mathcal{A}\mathcal{A}\text{hat}^{\text{mnop}} \sigma_1 (\nabla_a \sigma_2) (\nabla^a \beta_o) (\nabla_b \lambda_n) (\nabla^b \lambda_m) (\nabla_c \nabla^c \lambda_p) - \\
& 2 \mathcal{A}\mathcal{A}\mathcal{A}\text{hat}^{\text{mnop}} \sigma_1 (\nabla_a \lambda_n) (\nabla^a \lambda_m) (\nabla_b \sigma_2) (\nabla^b \lambda_o) (\nabla_c \nabla^c \lambda_p) + \\
& \frac{1}{2} \beta^m \sigma_1 (\nabla_a \lambda^o) (\nabla^a \lambda^n) (\nabla_b \mathcal{A}\mathcal{A}\mathcal{A}\text{hat}_{\text{nom}}^{\text{p}}) (\nabla^b \sigma_2) (\nabla_c \nabla^c \lambda_p) + \\
& \mathcal{A}\mathcal{A}\mathcal{A}\text{hat}^{\text{no p}}_{\text{m}} \beta^m \sigma_1 (\nabla^a \lambda_n) (\nabla_b \nabla_a \lambda_o) (\nabla^b \sigma_2) (\nabla_c \nabla^c \lambda_p) \\
\text{T[59]: } & \frac{1}{2} \mathcal{A}\mathcal{A}\mathcal{A}\text{hatp}^{\text{no p}}_{\text{m}} \beta^m \sigma_1 (\nabla_a \lambda_o) (\nabla^a \lambda_n) (\nabla_b \nabla_c \nabla^c \lambda_p) (\nabla^b \sigma_2) - \\
& \frac{1}{2} \mathcal{A}\mathcal{A}\mathcal{A}\text{hatp}^{\text{mnop}} \sigma_1 (\nabla_a \lambda_n) (\nabla^a \lambda_m) (\nabla_b \sigma_2) (\nabla^b \lambda_o) (\nabla_c \nabla^c \lambda_p) + \\
& \frac{1}{2} \beta^m \sigma_1 (\nabla_a \lambda^o) (\nabla^a \lambda^n) (\nabla^b \sigma_2) (\nabla_c \nabla_b \lambda_p) (\nabla^c \mathcal{A}\mathcal{A}\mathcal{A}\text{hatp}_{\text{nom}}^{\text{p}}) + \\
& \frac{1}{2} \mathcal{A}\mathcal{A}\mathcal{A}\text{hatp}^{\text{mnop}} \sigma_1 (\nabla_a \lambda_n) (\nabla^a \lambda_m) (\nabla_b \nabla_c \lambda_p) (\nabla^b \lambda_o) (\nabla^c \sigma_2) - \\
& \frac{1}{2} \mathcal{A}\mathcal{A}\mathcal{A}\text{hatp}^{\text{mnop}} \sigma_1 (\nabla^a \beta_o) (\nabla_b \lambda_n) (\nabla^b \lambda_m) (\nabla_c \nabla_a \lambda_p) (\nabla^c \sigma_2) + \\
& \frac{1}{2} \mathcal{A}\mathcal{A}\mathcal{A}\text{hatp}^{\text{mnop}} \sigma_1 (\nabla_a \lambda_n) (\nabla^a \lambda_m) (\nabla^b \lambda_o) (\nabla_c \nabla_b \lambda_p) (\nabla^c \sigma_2) + \\
& \mathcal{A}\mathcal{A}\mathcal{A}\text{hatp}^{\text{no p}}_{\text{m}} \beta^m \sigma_1 (\nabla^a \lambda_n) (\nabla^b \sigma_2) (\nabla_c \nabla_b \lambda_p) (\nabla^c \nabla_a \lambda_o) - \\
& \frac{1}{2} \mathcal{A}\mathcal{A}\mathcal{A}\text{hatp}_{\text{m}}^{\text{nop}} \beta^m \sigma_1 (\nabla_a \sigma_2) (\nabla^a \lambda_n) (\nabla_c \nabla_b \lambda_p) (\nabla^c \nabla^b \lambda_o)
\end{aligned}$$

$$\begin{aligned} \Gamma[60]: & \frac{1}{2} \mathcal{A}\mathcal{A}\mathcal{A}\text{hatpp}_m^{\text{no } p} \beta^m \sigma_1 (\nabla_a \sigma_2) (\nabla^a \lambda_n) (\bar{\nabla}_b \nabla_c \nabla^c \lambda_p) (\bar{\nabla}^b \lambda_o) + \\ & -\frac{1}{2} \mathcal{A}\mathcal{A}\mathcal{A}\text{hatpp}_m^{\text{nop}} \beta^m \sigma_1 (\nabla_a \sigma_2) (\nabla^a \lambda_n) (\bar{\nabla}_b \nabla_c \nabla^c \lambda_p) (\bar{\nabla}^b \lambda_o) - \\ & -\frac{1}{2} \mathcal{A}\mathcal{A}\mathcal{A}\text{hatpp}_m^{\text{nop}} \beta^m \sigma_1 (\nabla_a \nabla^c \lambda_o) (\nabla^a \lambda_n) (\bar{\nabla}_b \nabla_c \lambda_p) (\bar{\nabla}^b \sigma_2) - \\ & -\frac{1}{2} \mathcal{A}\mathcal{A}\mathcal{A}\text{hatpp}_m^{\text{nop}} \beta^m \sigma_1 (\nabla_a \nabla_c \lambda_p) (\nabla^a \lambda_n) (\bar{\nabla}_b \nabla^c \lambda_o) (\bar{\nabla}^b \sigma_2) + \\ & -\frac{1}{2} \beta^m \sigma_1 (\nabla_a \sigma_2) (\nabla^a \lambda^n) (\bar{\nabla}_b \nabla_c \lambda_p) (\bar{\nabla}^b \lambda^o) (\nabla^c \mathcal{A}\mathcal{A}\mathcal{A}\text{hatpp}_{\text{nom}}^p) + \\ & -\frac{1}{2} \beta^m \sigma_1 (\nabla_a \sigma_2) (\nabla^a \lambda^n) (\bar{\nabla}_b \nabla_c \lambda_p) (\bar{\nabla}^b \lambda^o) (\nabla^c \mathcal{A}\mathcal{A}\mathcal{A}\text{hatpp}_{\text{no } m}^p) + \\ & -\frac{1}{2} \mathcal{A}\mathcal{A}\mathcal{A}\text{hatpp}^{\text{mnop}} \sigma_1 (\nabla_a \sigma_2) (\nabla^a \lambda_m) (\bar{\nabla}_b \nabla_c \lambda_p) (\bar{\nabla}^b \lambda_n) (\nabla^c \lambda_o) - \\ & -\frac{1}{2} \mathcal{A}\mathcal{A}\mathcal{A}\text{hatpp}^{\text{mnop}} \sigma_1 (\nabla^a \lambda_m) (\bar{\nabla}_b \nabla_a \lambda_p) (\bar{\nabla}^b \lambda_n) (\nabla_c \sigma_2) (\nabla^c \lambda_o) + \\ & -\frac{1}{2} \mathcal{A}\mathcal{A}\mathcal{A}\text{hatpp}^{\text{mnop}} \sigma_1 (\nabla_a \sigma_2) (\nabla^a \lambda_m) (\bar{\nabla}_b \nabla_c \lambda_o) (\bar{\nabla}^b \lambda_n) (\nabla^c \lambda_p) - \\ & -\frac{1}{2} \mathcal{A}\mathcal{A}\mathcal{A}\text{hatpp}^{\text{mnop}} \sigma_1 (\nabla^a \lambda_m) (\bar{\nabla}_b \nabla_a \lambda_o) (\bar{\nabla}^b \lambda_n) (\nabla_c \sigma_2) (\nabla^c \lambda_p) - \\ & -\frac{1}{2} \mathcal{A}\mathcal{A}\mathcal{A}\text{hatpp}^{\text{mnop}} \sigma_1 (\nabla_a \lambda_m) (\nabla^a \beta_p) (\bar{\nabla}_b \nabla_c \lambda_o) (\bar{\nabla}^b \lambda_n) (\nabla^c \sigma_2) + \\ & -\frac{1}{2} \mathcal{A}\mathcal{A}\mathcal{A}\text{hatpp}^{\text{mnop}} \sigma_1 (\nabla_a \lambda_p) (\nabla^a \lambda_m) (\bar{\nabla}_b \nabla_c \lambda_o) (\bar{\nabla}^b \lambda_n) (\nabla^c \sigma_2) - \\ & -\frac{1}{2} \mathcal{A}\mathcal{A}\mathcal{A}\text{hatpp}^{\text{mnop}} \sigma_1 (\nabla_a \lambda_m) (\nabla^a \beta_o) (\bar{\nabla}_b \nabla_c \lambda_p) (\bar{\nabla}^b \lambda_n) (\nabla^c \sigma_2) + \\ & -\frac{1}{2} \mathcal{A}\mathcal{A}\mathcal{A}\text{hatpp}^{\text{mnop}} \sigma_1 (\nabla_a \lambda_o) (\nabla^a \lambda_m) (\bar{\nabla}_b \nabla_c \lambda_p) (\bar{\nabla}^b \lambda_n) (\nabla^c \sigma_2) + \\ & -\frac{1}{2} \mathcal{A}\mathcal{A}\mathcal{A}\text{hatpp}_m^{\text{no } p} \beta^m \sigma_1 (\nabla_a \nabla_c \lambda_p) (\nabla^a \lambda_n) (\bar{\nabla}^b \sigma_2) (\nabla^c \bar{\nabla}_b \lambda_o) + \\ & -\frac{1}{2} \mathcal{A}\mathcal{A}\mathcal{A}\text{hatpp}_m^{\text{nop}} \beta^m \sigma_1 (\nabla_a \nabla_c \lambda_p) (\nabla^a \lambda_n) (\bar{\nabla}^b \sigma_2) (\nabla^c \bar{\nabla}_b \lambda_o) + \\ & -\frac{1}{2} \mathcal{A}\mathcal{A}\mathcal{A}\text{hatpp}_m^{\text{no } p} \beta^m \sigma_1 (\nabla_a \sigma_2) (\nabla^a \lambda_n) (\bar{\nabla}_b \nabla_c \lambda_p) (\nabla^c \bar{\nabla}^b \lambda_o) + \\ & -\frac{1}{2} \mathcal{A}\mathcal{A}\mathcal{A}\text{hatpp}_m^{\text{nop}} \beta^m \sigma_1 (\nabla_a \sigma_2) (\nabla^a \lambda_n) (\bar{\nabla}_b \nabla_c \lambda_p) (\nabla^c \bar{\nabla}^b \lambda_o) \end{aligned}$$

[illegible]

$$\begin{aligned}
& \beta^m \sigma 1 (\nabla_a \sigma 2) (\nabla^a \lambda^n) (\nabla_b \nabla_c \lambda_p) (\nabla^b \lambda^o) (\nabla^c \mathcal{A}\mathcal{A}\mathcal{A}\mathcal{A}\text{checkp}_{\text{on}}^p{}_m) - \\
& \frac{1}{2} \beta^m \sigma 1 (\nabla_a \sigma 2) (\nabla^a \lambda^n) (\nabla_b \nabla_c \lambda_p) (\nabla^b \lambda^o) (\nabla^c \mathcal{A}\mathcal{A}\mathcal{A}\mathcal{A}\text{checkp}_{\text{nom}}^p) - \\
& \mathcal{A}\mathcal{A}\mathcal{A}\mathcal{A}\text{checkp}^{\text{mnop}} \sigma 1 (\nabla^a \beta_p) (\nabla_b \nabla_a \lambda_o) (\nabla^b \lambda_m) (\nabla_c \sigma 2) (\nabla^c \lambda_n) + \\
& \mathcal{A}\mathcal{A}\mathcal{A}\mathcal{A}\text{checkp}^{\text{mnop}} \sigma 1 (\nabla^a \beta_p) (\nabla_b \sigma 2) (\nabla^b \lambda_m) (\nabla_c \nabla_a \lambda_o) (\nabla^c \lambda_n) - \\
& \mathcal{A}\mathcal{A}\mathcal{A}\mathcal{A}\text{checkp}^{\text{mnop}} \sigma 1 (\nabla_a \nabla_c \beta_p) (\nabla^a \lambda_m) (\nabla_b \sigma 2) (\nabla^b \lambda_n) (\nabla^c \lambda_o) + \\
& \frac{3}{2} \mathcal{A}\mathcal{A}\mathcal{A}\mathcal{A}\text{checkp}^{\text{mnop}} \sigma 1 (\nabla_a \nabla_c \lambda_p) (\nabla^a \lambda_m) (\nabla_b \sigma 2) (\nabla^b \lambda_n) (\nabla^c \lambda_o) + \\
& \frac{1}{2} \mathcal{A}\mathcal{A}\mathcal{A}\mathcal{A}\text{checkp}^{\text{mnop}} \sigma 1 (\nabla^a \lambda_m) (\nabla_b \sigma 2) (\nabla^b \lambda_n) (\nabla_c \nabla_a \lambda_p) (\nabla^c \lambda_o) + \\
& \frac{1}{2} \mathcal{A}\mathcal{A}\mathcal{A}\mathcal{A}\text{checkp}^{\text{mnop}} \sigma 1 (\nabla_a \sigma 2) (\nabla^a \lambda_m) (\nabla^b \lambda_n) (\nabla_c \nabla_b \beta_p) (\nabla^c \lambda_o) - \\
& \mathcal{A}\mathcal{A}\mathcal{A}\mathcal{A}\text{checkp}^{\text{mnop}} \sigma 1 (\nabla_a \sigma 2) (\nabla^a \lambda_m) (\nabla_b \nabla_c \lambda_o) (\nabla^b \lambda_n) (\nabla^c \lambda_p) + \\
& \mathcal{A}\mathcal{A}\mathcal{A}\mathcal{A}\text{checkp}^{\text{mnop}} \sigma 1 (\nabla_a \sigma 2) (\nabla^a \lambda_m) (\nabla^b \lambda_n) (\nabla_c \nabla_b \lambda_o) (\nabla^c \lambda_p) + \\
& \frac{1}{2} \sigma 1 (\nabla_a \lambda^n) (\nabla^a \lambda^m) (\nabla_b \sigma 2) (\nabla^b \lambda^o) (\nabla_c \mathcal{A}\mathcal{A}\mathcal{A}\mathcal{A}\text{checkp}_{\text{omnp}}) (\nabla^c \lambda^p) - \\
& \sigma 1 (\nabla_a \lambda^n) (\nabla^a \lambda^m) (\nabla_b \sigma 2) (\nabla^b \lambda^o) (\nabla_c \mathcal{A}\mathcal{A}\mathcal{A}\mathcal{A}\text{checkp}_{\text{omnp}}) (\nabla^c \lambda^p) + \\
& \sigma 1 (\nabla_a \lambda^n) (\nabla^a \beta^m) (\nabla_b \sigma 2) (\nabla^b \lambda^o) (\nabla_c \mathcal{A}\mathcal{A}\mathcal{A}\mathcal{A}\text{checkp}_{\text{onpm}}) (\nabla^c \lambda^p) - \\
& \frac{1}{2} \sigma 1 (\nabla_a \lambda^n) (\nabla^a \beta^m) (\nabla_b \sigma 2) (\nabla^b \lambda^o) (\nabla_c \mathcal{A}\mathcal{A}\mathcal{A}\mathcal{A}\text{checkp}_{\text{pnom}}) (\nabla^c \lambda^p) - \\
& \frac{1}{2} \beta^m \sigma 1 (\nabla_a \sigma 2) (\nabla^a \lambda^n) (\nabla^b \lambda^o) (\nabla_c \nabla_b \mathcal{A}\mathcal{A}\mathcal{A}\mathcal{A}\text{checkp}_{\text{onpm}}) (\nabla^c \lambda^p) - \\
& \frac{1}{2} \mathcal{A}\mathcal{A}\mathcal{A}\mathcal{A}\text{checkp}^{\text{mnop}} \sigma 1 (\nabla_a \nabla_c \lambda_p) (\nabla^a \lambda_m) (\nabla_b \lambda_o) (\nabla^b \lambda_n) (\nabla^c \sigma 2) - \\
& \frac{1}{2} \mathcal{A}\mathcal{A}\mathcal{A}\mathcal{A}\text{checkp}_m^{\text{n op}} \beta^m \sigma 1 (\nabla_a \nabla_b \nabla_c \lambda_p) (\nabla^a \lambda_n) (\nabla^b \lambda_o) (\nabla^c \sigma 2) - \\
& \frac{1}{2} \mathcal{A}\mathcal{A}\mathcal{A}\mathcal{A}\text{checkp}_m^{\text{n op}} \beta^m \sigma 1 (\nabla_a \nabla_c \nabla_b \lambda_p) (\nabla^a \lambda_n) (\nabla^b \lambda_o) (\nabla^c \sigma 2) + \\
& \mathcal{A}\mathcal{A}\mathcal{A}\mathcal{A}\text{checkp}^{\text{mnop}} \sigma 1 (\nabla_a \lambda_n) (\nabla^a \beta_p) (\nabla_b \nabla_c \lambda_m) (\nabla^b \lambda_o) (\nabla^c \sigma 2) - \\
& \mathcal{A}\mathcal{A}\mathcal{A}\mathcal{A}\text{checkp}^{\text{mnop}} \sigma 1 (\nabla_a \lambda_p) (\nabla^a \lambda_n) (\nabla_b \nabla_c \lambda_m) (\nabla^b \lambda_o) (\nabla^c \sigma 2) - \\
& \frac{1}{2} \mathcal{A}\mathcal{A}\mathcal{A}\mathcal{A}\text{checkp}^{\text{mnop}} \sigma 1 (\nabla_a \lambda_n) (\nabla^a \lambda_m) (\nabla_b \nabla_c \lambda_p) (\nabla^b \lambda_o) (\nabla^c \sigma 2) - \\
& \frac{1}{2} \beta^m \sigma 1 (\nabla_a \mathcal{A}\mathcal{A}\mathcal{A}\mathcal{A}\text{checkp}_{\text{no}}^p{}_m) (\nabla^a \lambda^n) (\nabla_b \nabla_c \lambda_p) (\nabla^b \lambda^o) (\nabla^c \sigma 2) + \\
& \frac{1}{2} \mathcal{A}\mathcal{A}\mathcal{A}\mathcal{A}\text{checkp}^{\text{mnop}} \sigma 1 (\nabla_a \lambda_o) (\nabla^a \lambda_n) (\nabla_b \nabla_c \lambda_m) (\nabla^b \lambda_p) (\nabla^c \sigma 2) - \\
& \frac{1}{2} \mathcal{A}\mathcal{A}\mathcal{A}\mathcal{A}\text{checkp}^{\text{mnop}} \sigma 1 (\nabla_a \lambda_n) (\nabla^a \lambda_m) (\nabla^b \lambda_o) (\nabla_c \nabla_b \lambda_p) (\nabla^c \sigma 2) - \\
& \frac{1}{2} \mathcal{A}\mathcal{A}\mathcal{A}\mathcal{A}\text{checkp}_m^{\text{nop}} \beta^m \sigma 1 (\nabla^a \lambda_n) (\nabla^b \lambda_o) (\nabla_c \nabla_b \nabla_a \lambda_p) (\nabla^c \sigma 2) - \\
& \mathcal{A}\mathcal{A}\mathcal{A}\mathcal{A}\text{checkp}_m^{\text{nop}} \beta^m \sigma 1 (\nabla_a \nabla_c \lambda_p) (\nabla^a \lambda_n) (\nabla^b \sigma 2) (\nabla^c \nabla_b \lambda_o) - \\
& \mathcal{A}\mathcal{A}\mathcal{A}\mathcal{A}\text{checkp}_m^{\text{nop}} \beta^m \sigma 1 (\nabla_a \sigma 2) (\nabla^a \lambda_o) (\nabla_b \nabla_c \lambda_p) (\nabla^c \nabla^b \lambda_n)
\end{aligned}$$

$$\begin{aligned}
T[63]: & -\mathcal{A}\mathcal{A}\mathcal{A}\mathcal{A}_m^{\text{nopq}} \beta^m \sigma_1 (\nabla_a \sigma_2) (\nabla^a \lambda_n) (\nabla_b \lambda_p) (\nabla^b \lambda_o) (\nabla_c \nabla^c \lambda_q) - \\
& \frac{1}{4} \mathcal{A}\mathcal{A}\mathcal{A}\mathcal{A}^{\text{mnopq}} \sigma_1 (\nabla_a \sigma_2) (\nabla^a \beta_q) (\nabla_b \lambda_n) (\nabla^b \lambda_m) (\nabla_c \lambda_p) (\nabla^c \lambda_o) - \\
& \mathcal{A}\mathcal{A}\mathcal{A}\mathcal{A}^{\text{mnopq}} \sigma_1 (\nabla_a \lambda_n) (\nabla^a \lambda_m) (\nabla_b \lambda_p) (\nabla^b \lambda_o) (\nabla_c \sigma_2) (\nabla^c \lambda_q) + \\
& \frac{1}{4} \beta^m \sigma_1 (\nabla_a \lambda^o) (\nabla^a \lambda^n) (\nabla_b \lambda^q) (\nabla^b \lambda^p) (\nabla_c \mathcal{A}\mathcal{A}\mathcal{A}\mathcal{A}_{\text{nopqm}}) (\nabla^c \sigma_2) + \\
& \mathcal{A}\mathcal{A}\mathcal{A}\mathcal{A}^{\text{nopq}}_m \beta^m \sigma_1 (\nabla_a \lambda_o) (\nabla^a \lambda_n) (\nabla^b \lambda_p) (\nabla_c \nabla_b \lambda_q) (\nabla^c \sigma_2)
\end{aligned}$$

$$\begin{aligned}
T[64]: & \frac{1}{4} \mathcal{A}\mathcal{A}\mathcal{A}\mathcal{A}\mathcal{P}^{\text{nopq}}_m \beta^m \sigma_1 (\nabla_a \lambda_o) (\nabla^a \lambda_n) (\nabla_b \sigma_2) (\nabla^b \lambda_p) (\nabla_c \nabla^c \lambda_q) - \\
& \frac{1}{4} \mathcal{A}\mathcal{A}\mathcal{A}\mathcal{A}\mathcal{P}^{\text{mnopq}} \sigma_1 (\nabla_a \lambda_o) (\nabla^a \beta_q) (\nabla_b \lambda_n) (\nabla^b \lambda_m) (\nabla_c \sigma_2) (\nabla^c \lambda_p) + \\
& \frac{1}{2} \mathcal{A}\mathcal{A}\mathcal{A}\mathcal{A}\mathcal{P}^{\text{mnopq}} \sigma_1 (\nabla_a \lambda_n) (\nabla^a \lambda_m) (\nabla_b \lambda_q) (\nabla^b \lambda_o) (\nabla_c \sigma_2) (\nabla^c \lambda_p) - \\
& \frac{1}{2} \mathcal{A}\mathcal{A}\mathcal{A}\mathcal{A}\mathcal{P}_m^{\text{nopq}} \beta^m \sigma_1 (\nabla_a \sigma_2) (\nabla^a \lambda_n) (\nabla^b \lambda_o) (\nabla_c \nabla_b \lambda_q) (\nabla^c \lambda_p) - \\
& \frac{1}{4} \mathcal{A}\mathcal{A}\mathcal{A}\mathcal{A}\mathcal{P}^{\text{mnopq}} \sigma_1 (\nabla_a \lambda_n) (\nabla^a \lambda_m) (\nabla_b \lambda_p) (\nabla^b \lambda_o) (\nabla_c \sigma_2) (\nabla^c \lambda_q) + \\
& \frac{1}{2} \mathcal{A}\mathcal{A}\mathcal{A}\mathcal{A}\mathcal{P}^{\text{nopq}}_m \beta^m \sigma_1 (\nabla^a \lambda_n) (\nabla_b \sigma_2) (\nabla^b \lambda_p) (\nabla_c \nabla_a \lambda_o) (\nabla^c \lambda_q) + \\
& \frac{1}{4} \beta^m \sigma_1 (\nabla_a \lambda^o) (\nabla^a \lambda^n) (\nabla_b \sigma_2) (\nabla^b \lambda^p) (\nabla_c \mathcal{A}\mathcal{A}\mathcal{A}\mathcal{A}\mathcal{P}_{\text{nopqm}}) (\nabla^c \lambda^q) - \\
& \frac{1}{4} \mathcal{A}\mathcal{A}\mathcal{A}\mathcal{A}\mathcal{P}^{\text{no pq}}_m \beta^m \sigma_1 (\nabla_a \lambda_o) (\nabla^a \lambda_n) (\nabla_b \nabla_c \lambda_q) (\nabla^b \lambda_p) (\nabla^c \sigma_2) + \\
& \frac{1}{4} \mathcal{A}\mathcal{A}\mathcal{A}\mathcal{A}\mathcal{P}^{\text{nopq}}_m \beta^m \sigma_1 (\nabla_a \lambda_o) (\nabla^a \lambda_n) (\nabla_b \nabla_c \lambda_q) (\nabla^b \lambda_p) (\nabla^c \sigma_2) - \\
& \frac{1}{4} \mathcal{A}\mathcal{A}\mathcal{A}\mathcal{A}\mathcal{P}^{\text{no pq}}_m \beta^m \sigma_1 (\nabla_a \lambda_o) (\nabla^a \lambda_n) (\nabla^b \lambda_p) (\nabla_c \nabla_b \lambda_q) (\nabla^c \sigma_2)
\end{aligned}$$

$$T[65]: -\frac{3}{4} \mathcal{A}\mathcal{A}\mathcal{A}\mathcal{A}\mathcal{A}_m^{\text{nopqr}} \beta^m \sigma_1 (\nabla_a \sigma_2) (\nabla^a \lambda_n) (\nabla_b \lambda_p) (\nabla^b \lambda_o) (\nabla_c \lambda_r) (\nabla^c \lambda_q)$$

$$\begin{aligned}
Z[26]: & \mathcal{A}\mathcal{A}^{\text{mn}} \sigma_1 (\nabla_a \nabla^b \lambda_n) (\nabla^a \sigma_2) (\nabla_b \nabla_c \nabla^c \beta_m) + \\
& \mathcal{A}\mathcal{A}^{\text{mn}} \sigma_1 (\nabla_a \nabla^b \beta_n) (\nabla^a \sigma_2) (\nabla_b \nabla_c \nabla^c \lambda_m) + \beta^m \sigma_1 \partial_m \mathcal{A}\mathcal{A}^{\text{no}} (\nabla_a \nabla^b \lambda_o) (\nabla^a \sigma_2) (\nabla_b \nabla_c \nabla^c \lambda_n)
\end{aligned}$$

$$\begin{aligned}
Z[27]: & \mathcal{A}\mathcal{A}\mathcal{P}^{\text{mn}} \sigma_1 (\nabla_a \sigma_2) (\nabla^a \lambda_m) (\nabla_c \nabla^c \nabla_b \nabla^b \beta_n) + \\
& \mathcal{A}\mathcal{A}\mathcal{P}^{\text{mn}} \sigma_1 (\nabla_a \sigma_2) (\nabla^a \beta_m) (\nabla_c \nabla^c \nabla_b \nabla^b \lambda_n) + \beta^m \sigma_1 \partial_m \mathcal{A}\mathcal{A}\mathcal{P}^{\text{no}} (\nabla_a \sigma_2) (\nabla^a \lambda_n) (\nabla_c \nabla^c \nabla_b \nabla^b \lambda_o)
\end{aligned}$$

$$\begin{aligned}
Z[28]: & \mathcal{A}\mathcal{A}\mathcal{A}^{\text{mno}} \sigma_1 (\nabla^a \lambda_m) (\nabla_b \nabla_a \lambda_n) (\nabla^b \sigma_2) (\nabla_c \nabla^c \beta_o) + \\
& \mathcal{A}\mathcal{A}\mathcal{A}^{\text{mno}} \sigma_1 (\nabla^a \lambda_m) (\nabla_b \nabla_a \beta_n) (\nabla^b \sigma_2) (\nabla_c \nabla^c \lambda_o) + \mathcal{A}\mathcal{A}\mathcal{A}^{\text{mno}} \sigma_1 (\nabla^a \beta_m) (\nabla_b \nabla_a \lambda_n) (\nabla^b \sigma_2) (\nabla_c \nabla^c \lambda_o) + \\
& \beta^m \sigma_1 \partial_m \mathcal{A}\mathcal{A}\mathcal{A}^{\text{nop}} (\nabla^a \lambda_n) (\nabla_b \nabla_a \lambda_o) (\nabla^b \sigma_2) (\nabla_c \nabla^c \lambda_p)
\end{aligned}$$

$$\begin{aligned}
Z[29]: & \mathcal{A}\mathcal{A}\mathcal{P}^{\text{mno}} \sigma_1 (\nabla_a \nabla^c \beta_o) (\nabla^a \lambda_m) (\nabla_b \nabla_c \lambda_n) (\nabla^b \sigma_2) + \mathcal{A}\mathcal{A}\mathcal{P}^{\text{mno}} \sigma_1 (\nabla_a \nabla_c \lambda_o) (\nabla^a \lambda_m) (\nabla_b \nabla^c \beta_n) (\nabla^b \sigma_2) + \\
& \mathcal{A}\mathcal{A}\mathcal{P}^{\text{mno}} \sigma_1 (\nabla_a \nabla_c \lambda_o) (\nabla^a \beta_m) (\nabla_b \nabla^c \lambda_n) (\nabla^b \sigma_2) + \\
& \beta^m \sigma_1 \partial_m \mathcal{A}\mathcal{A}\mathcal{P}_n^{\text{op}} (\nabla_a \nabla_c \lambda_p) (\nabla^a \lambda^n) (\nabla_b \nabla^c \lambda_o) (\nabla^b \sigma_2)
\end{aligned}$$



$$\begin{aligned}
Z[30]: & \frac{1}{2} \mathcal{R}\mathcal{R}\mathcal{R}\mathcal{R}^{mnop} \sigma_1 (\nabla_a \lambda_n) (\nabla^a \lambda_m) (\nabla_b \sigma_2) (\nabla^b \lambda_o) (\nabla_c \nabla^c \beta_p) + \\
& \frac{1}{2} \mathcal{R}\mathcal{R}\mathcal{R}\mathcal{R}^{mnop} \sigma_1 (\nabla_a \sigma_2) (\nabla^a \beta_o) (\nabla_b \lambda_n) (\nabla^b \lambda_m) (\nabla_c \nabla^c \lambda_p) + \\
& \mathcal{R}\mathcal{R}\mathcal{R}\mathcal{R}^{mnop} \sigma_1 (\nabla_a \lambda_n) (\nabla^a \beta_m) (\nabla_b \sigma_2) (\nabla^b \lambda_o) (\nabla_c \nabla^c \lambda_p) + \\
& \frac{1}{2} \beta^m \sigma_1 \partial_m \mathcal{R}\mathcal{R}\mathcal{R}\mathcal{R}_{nop}{}^q (\nabla_a \lambda^o) (\nabla^a \lambda^n) (\nabla_b \sigma_2) (\nabla^b \lambda^p) (\nabla_c \nabla^c \lambda_q)
\end{aligned}$$
